# Supplementary material for: Two-loop corrections to the Carroll-Field-Jackiw term in a CPT-odd Lorentz-violating scalar QED
Source: arXiv:2310.15715 source file (2024-02-04)
Supplement: Supplementary file 1 [file Supplemental_Material-LV-ODD-SQED-2_pn.pdf]

# Supplemental Material: Two-loop corrections to the Carroll-Field-Jackiw term in a CPT-odd Lorentz-violating scalar QED

A. C. Lehum,[1,*] J. R. Nascimento,[2,†] and A. Yu. Petrov[2,‡]

[1]*Faculdade de Física, Universidade Federal do Pará, 66075-110, Belém, Pará, Brazil*

[2]*Departamento de Física, Universidade Federal da Paraíba, Caixa Postal 5008, 58051-970 João Pessoa, Paraíba, Brazil*

## Abstract

This supplemental material accompanies the paper titled "Two-loop corrections to the Carroll-Field-Jackiw term in a CPT-odd Lorentz-violating scalar QED". In this document, we provide additional information and calculation details that were omitted from the main text, including the two-loop diagrams associated with the photon and scalar field self-energies. Throughout this supplementary material, we adopt natural units with $c = \hbar = 1$, and employ the spacetime signature $(+ - - -)$.

*Electronic address: lehum@ufpa.br

†Electronic address: jroberto@fisica.ufpb.br

‡Electronic address: petrov@fisica.ufpb.br

## I. CALCULATION OF THE TWO-LOOP SELF-ENERGY DIAGRAMS

We initiate our analysis by investigating the two-loop corrections associated with the photon self-energy. The computation of the diagrams is performed utilizing a set of MATHEMATICA packages [1–5].

The Lorentz-violating (LV) corrections to the two-loop photon self-energy are depicted in Figure 1. While the diagrams shown in Figure 2 are expected to contribute to the photon self-energy at the same order as the two-loop diagrams, they collectively cancel each other out, resulting in a net contribution of zero. The two-loop LV corrections to the sdcalar field self-energy is depicted in Figure 3.

Upon combining all the contributions from Figure 1, we derive the following result:

$$\begin{aligned}\Pi^{\mu\beta}_{2l}(p) &= \frac{8e^4Q_2}{(D-4)^2(D-1)p^2}b_\sigma p_\rho\epsilon^{\beta\mu\rho\sigma}\Big[(D-4)p^2(\mathbf{B}^{(D)}_{\{1,0\},\{1,0\}})^2 \\ &\quad +(D^4-12D^3+49D^2-82D+48)\mathbf{J}^{(D)}_{\{1,0\},\{1,0\},\{1,0\}}\Big] \\ &= \frac{e^4Q_2(6\zeta(3)-5)p_\rho b_\sigma\epsilon^{\beta\mu\rho\sigma}}{192\pi^4}, \end{aligned} \tag{1}$$

where the definitions of the integrals are provided in the Appendix. It is worth noting that this contribution is UV finite. This constitutes the two-loop corrections to the Carroll-Field-Jackiw term.

First we contruct the amplitudes through the Feynman rules and the subsequent step involves applying the Tarasov algorithm [6] to express the scalar integrals in terms of a set of fundamental ones. This procedure is facilitated by utilizing the TARCER package [5] within the MATHEMATICA software.

The basic integrals used in this text and employed by the TARCER package, as defined in Ref. [5], are

$$\mathbf{B}^{(D)}_{\{1,0\},\{1,0\}} = \frac{1}{\pi^{D/2}}\int\frac{d^Dk}{k^2(k-p)^2} = \frac{i}{\epsilon} - i\left(\log(-p^2)+\gamma_E-2\right)+\mathcal{O}(\epsilon); \tag{2}$$

$$\mathbf{J}^{(D)}_{\{1,0\},\{1,0\},\{1,0\}} = \frac{1}{\pi^D}\int\frac{d^Dk_1\,d^Dk_2}{k_1^2(k_1-k_2)^2(k_2-p)^2} = \frac{p^2}{2}\left(\frac{1}{2\epsilon}-\log(-p^2)-\gamma_E+\frac{13}{4}\right)+\mathcal{O}(\epsilon), \tag{3}$$

where $\gamma_E$ is the Euler-Mascheroni constant and $D=4-2\epsilon$. The one-loop integrals are well-known and have been extensively studied in the literature. A comprehensive calculation of the two-loop integral was carried out in Ref. [7].

The diagrams shown in Figure 1 follow the format

$\Pi_i^{\mu\beta}(p) = \int \frac{d^D k_1}{(2\pi)^D} \frac{d^D k_2}{(2\pi)^D} \tilde{\Pi}_i^{\mu\beta}(p, k_1, k_2)$, and each individual contribution can be expressed as:

$$\tilde{\Pi}_1^{\mu\beta}(p, k_1, k_2) = -2\, i\, \mathrm{e}^4\, Q_1\, (p^\mu + 2\, k_1{}^\mu)\, (k_2 \cdot u) \left( \frac{(\xi - 1)\left(k_1{}^2 - k_2{}^2\right)\left(k_1{}^\beta + k_2{}^\beta\right)}{\left(k_2{}^2\right)^2 . k_1{}^2 . (\, k_1 + p\,)^2 . (\, k_1 + k_2\,)^{22}} + \frac{k_1{}^\beta - k_2{}^\beta}{\left(k_2{}^2\right)^2 . k_1{}^2 . (\, k_1 + p\,)^2 . (\, k_1 + k_2\,)^2} \right)$$

$$\tilde{\Pi}_2^{\mu\beta}(p, k_1, k_2) = 2\, i\, \mathrm{e}^4\, Q_1\, (p^\mu + 2\, k_1{}^\mu)\, (k_2 \cdot u) \left( \frac{(\xi - 1)\left(k_1{}^2 - k_2{}^2\right)\left(k_1{}^\beta + k_2{}^\beta\right)}{\left(k_2{}^2\right)^2 . k_1{}^2 . (\, k_1 + p\,)^2 . (\, k_1 + k_2\,)^{22}} + \frac{k_1{}^\beta - k_2{}^\beta}{\left(k_2{}^2\right)^2 . k_1{}^2 . (\, k_1 + p\,)^2 . (\, k_1 + k_2\,)^2} \right)$$

$$\tilde{\Pi}_3^{\mu\beta}(p, k_1, k_2) = \frac{8\, \mathrm{e}^4\, Q_2\, (p^\mu + 2\, k_1{}^\mu)\, \epsilon^{\beta b k_1 k_2}}{\left(k_2{}^2\right)^2 . k_1{}^2 . (\, k_1 + p\,)^2 . (\, k_1 + k_2\,)^2}$$

$$\tilde{\Pi}_4^{\mu\beta}(p, k_1, k_2) = \frac{8\, \mathrm{e}^4\, Q_2\, (p^\mu + 2\, k_1{}^\mu)\, \epsilon^{\beta b k_1 k_2}}{\left(k_2{}^2\right)^2 . k_1{}^2 . (\, k_1 + p\,)^2 . (\, k_1 + k_2\,)^2}$$

$$\tilde{\Pi}_5^{\mu\beta}(p, k_1, k_2) =$$

$$-i\, \mathrm{e}^4\, Q_1\, (p^\mu + 2\, k_1{}^\mu)\left(2\, k_2{}^\beta - p^\beta\right) \left( \frac{(\xi - 1)\left(k_1{}^2 - k_2{}^2\right)(k_1 \cdot u + k_2 \cdot u)}{k_2{}^2 . k_1{}^2 . (\, k_1 + p\,)^2 . (\, k_2 - p\,)^2 . (\, k_1 + k_2\,)^{22}} + \frac{k_1 \cdot u - k_2 \cdot u}{k_2{}^2 . k_1{}^2 . (\, k_1 + p\,)^2 . (\, k_2 - p\,)^2 . (\, k_1 + k_2\,)^2} \right)$$

$$\tilde{\Pi}_6^{\mu\beta}(p, k_1, k_2) = i\, \mathrm{e}^4\, Q_1\, (p^\mu + 2\, k_1{}^\mu)\left(2\, k_2{}^\beta - p^\beta\right)$$
$$\left( \frac{(\xi - 1)\left(k_1{}^2 - k_2{}^2\right)(k_1 \cdot u + k_2 \cdot u)}{k_2{}^2 . k_1{}^2 . (\, k_1 + p\,)^2 . (\, k_2 - p\,)^2 . (\, k_1 + k_2\,)^{22}} + \frac{k_1 \cdot u - k_2 \cdot u}{k_2{}^2 . k_1{}^2 . (\, k_1 + p\,)^2 . (\, k_2 - p\,)^2 . (\, k_1 + k_2\,)^2} \right)$$

$$\tilde{\Pi}_7^{\mu\beta}(p, k_1, k_2) = -2\, i\, \mathrm{e}^4\, Q_1 \left(2\, k_2{}^\beta - p^\beta\right)(k_1 \cdot u) \left( \frac{(\xi - 1)\left(k_1{}^2 - k_2{}^2\right)(k_1{}^\mu + k_2{}^\mu)}{k_1{}^2 . k_2{}^2 . k_1{}^2 . (\, k_2 - p\,)^2 . (\, k_1 + k_2\,)^{22}} + \frac{k_1{}^\mu - k_2{}^\mu}{k_1{}^2 . k_2{}^2 . k_1{}^2 . (\, k_2 - p\,)^2 . (\, k_1 + k_2\,)^2} \right)$$

$$\tilde{\Pi}_8^{\mu\beta}(p, k_1, k_2) = 2\, i\, \mathrm{e}^4\, Q_1 \left(2\, k_2{}^\beta - p^\beta\right)(k_1 \cdot u) \left( \frac{(\xi - 1)\left(k_1{}^2 - k_2{}^2\right)(k_1{}^\mu + k_2{}^\mu)}{k_1{}^2 . k_2{}^2 . k_1{}^2 . (\, k_2 - p\,)^2 . (\, k_1 + k_2\,)^{22}} + \frac{k_1{}^\mu - k_2{}^\mu}{k_1{}^2 . k_2{}^2 . k_1{}^2 . (\, k_2 - p\,)^2 . (\, k_1 + k_2\,)^2} \right)$$

$$\tilde{\Pi}_9^{\mu\beta}(p, k_1, k_2) = \frac{8\, \mathrm{e}^4\, Q_2 \left(p^\beta - 2\, k_2{}^\beta\right) \epsilon^{\mu b k_1 k_2}}{k_1{}^2 . k_2{}^2 . k_1{}^2 . (\, k_2 - p\,)^2 . (\, k_1 + k_2\,)^2}$$

$$\tilde{\Pi}_{10}^{\mu\beta}(p, k_1, k_2) = \frac{8\, \mathrm{e}^4\, Q_2 \left(p^\beta - 2\, k_2{}^\beta\right) \epsilon^{\mu b k_1 k_2}}{k_1{}^2 . k_2{}^2 . k_1{}^2 . (\, k_2 - p\,)^2 . (\, k_1 + k_2\,)^2}$$

$$\tilde{\Pi}_{11}^{\mu\beta}(p, k_1, k_2) = -i\, \mathrm{e}^4\, Q_1\, (p^\mu + 2\, k_1{}^\mu)\left(2\, k_2{}^\beta - p^\beta\right)(k_2 \cdot u - p \cdot u)$$
$$\left( \frac{(\xi - 1)\left(k_1{}^2 - k_2{}^2\right)\left(2\,(k_1 \cdot p) + 2\,(k_2 \cdot p) + k_1{}^2 - k_2{}^2\right)}{k_2{}^2 . k_1{}^2 . (\, k_1 + p\,)^2 . (\, k_2 - p\,)^{22} . (\, k_1 + k_2\,)^{22}} + \frac{2\,(k_1 \cdot p) - 2\,(k_2 \cdot p) - 2\,(k_1 \cdot k_2) + k_1{}^2 + k_2{}^2}{k_2{}^2 . k_1{}^2 . (\, k_1 + p\,)^2 . (\, k_2 - p\,)^{22} . (\, k_1 + k_2\,)^2} \right)$$

$$\tilde{\Pi}_{12}^{\mu\beta}(p, k_1, k_2) = i\, \mathrm{e}^4\, Q_1\, (p^\mu + 2\, k_1{}^\mu)\left(2\, k_2{}^\beta - p^\beta\right)(k_2 \cdot u - p \cdot u)$$
$$\left( \frac{(\xi - 1)\left(k_1{}^2 - k_2{}^2\right)\left(2\,(k_1 \cdot p) + 2\,(k_2 \cdot p) + k_1{}^2 - k_2{}^2\right)}{k_2{}^2 . k_1{}^2 . (\, k_1 + p\,)^2 . (\, k_2 - p\,)^{22} . (\, k_1 + k_2\,)^{22}} + \frac{2\,(k_1 \cdot p) - 2\,(k_2 \cdot p) - 2\,(k_1 \cdot k_2) + k_1{}^2 + k_2{}^2}{k_2{}^2 . k_1{}^2 . (\, k_1 + p\,)^2 . (\, k_2 - p\,)^{22} . (\, k_1 + k_2\,)^2} \right)$$

$$\tilde{\Pi}_{13}^{\mu\beta}(p, k_1, k_2) = -i\, \mathrm{e}^4\, Q_1\, (2\, k_1{}^\mu - p^\mu)\left(2\, k_2{}^\beta - p^\beta\right)(k_1 \cdot u)$$
$$\left( \frac{(\xi - 1)\left(2\,(k_2 \cdot p) - p^2 + k_1{}^2 - k_2{}^2\right)\left(-2\,(k_1 \cdot p) + p^2 + k_1{}^2 - k_2{}^2\right)}{k_1{}^2 . k_2{}^2 . k_1{}^2 . (\, k_1 - p\,)^2 . (\, k_2 - p\,)^2 . (\, k_1 + k_2 - p\,)^{22}} + \frac{-p^2 - 2\,(k_1 \cdot k_2) + k_1{}^2 + k_2{}^2}{k_1{}^2 . k_2{}^2 . k_1{}^2 . (\, k_1 - p\,)^2 . (\, k_2 - p\,)^2 . (\, k_1 + k_2 - p\,)^2} \right)$$

$$\tilde{\Pi}_{14}^{\mu\beta}(p, k_1, k_2) = i\, \mathrm{e}^4\, Q_1\, (2\, k_1{}^\mu - p^\mu)\left(2\, k_2{}^\beta - p^\beta\right)(k_1 \cdot u)$$
$$\left( \frac{(\xi - 1)\left(2\,(k_2 \cdot p) - p^2 + k_1{}^2 - k_2{}^2\right)\left(-2\,(k_1 \cdot p) + p^2 + k_1{}^2 - k_2{}^2\right)}{k_1{}^2 . k_2{}^2 . k_1{}^2 . (\, k_1 - p\,)^2 . (\, k_2 - p\,)^2 . (\, k_1 + k_2 - p\,)^{22}} + \frac{-p^2 - 2\,(k_1 \cdot k_2) + k_1{}^2 + k_2{}^2}{k_1{}^2 . k_2{}^2 . k_1{}^2 . (\, k_1 - p\,)^2 . (\, k_2 - p\,)^2 . (\, k_1 + k_2 - p\,)^2} \right)$$

$$\tilde{\Pi}_{15}^{\mu\beta}(p, k_1, k_2) = -i\, \mathrm{e}^4\, Q_1 \left(2\, k_1{}^\beta - p^\beta\right)(2\, k_1{}^\mu - p^\mu)\, (k_2 \cdot u)$$
$$\left( \frac{(\xi - 1)\left(-2\,(k_1 \cdot p) + p^2 + k_1{}^2 - k_2{}^2\right)^2}{\left(k_2{}^2\right)^2 . k_1{}^2 . (\, k_1 - p\,)^{22} . (\, k_1 + k_2 - p\,)^{22}} + \frac{-2\,(k_1 \cdot p) + 2\,(k_2 \cdot p) + p^2 - 2\,(k_1 \cdot k_2) + k_1{}^2 + k_2{}^2}{\left(k_2{}^2\right)^2 . k_1{}^2 . (\, k_1 - p\,)^{22} . (\, k_1 + k_2 - p\,)^2} \right)$$

$$\tilde{\Pi}_{16}^{\mu\beta}(p,k_1,k_2) = i\,\mathrm{e}^4\,Q_1\left(2\,k_1{}^\beta - p^\beta\right)(2\,k_1{}^\mu - p^\mu)\,(k_2\cdot u)$$

$$\left(\frac{(\xi-1)\left(-2\,(k_1\cdot p)+p^2+k_1{}^2-k_2{}^2\right)^2}{\left(k_2{}^2\right)^2.k_1{}^2.(\,k_1-p\,)^{22}.(\,k_1+k_2-p\,)^{22}} + \frac{-2\,(k_1\cdot p)+2\,(k_2\cdot p)+p^2-2\,(k_1\cdot k_2)+k_1{}^2+k_2{}^2}{\left(k_2{}^2\right)^2.k_1{}^2.(\,k_1-p\,)^{22}.(\,k_1+k_2-p\,)^2}\right)$$

$$\tilde{\Pi}_{17}^{\mu\beta}(p,k_1,k_2) = 0$$

$$\tilde{\Pi}_{18}^{\mu\beta}(p,k_1,k_2) = 0$$

$$\tilde{\Pi}_{19}^{\mu\beta}(p,k_1,k_2) =$$

$$-2\,i\,\mathrm{e}^4\,Q_1\,(2\,k_1{}^\mu - p^\mu)\left(\frac{(\xi-1)\left(-p^\beta+k_1{}^\beta-k_2{}^\beta\right)(-p\cdot u+k_1\cdot u-k_2\cdot u)}{k_2{}^2.k_1{}^2.(\,k_1-p\,)^2.(\,-k_1+k_2+p\,)^{22}} + \frac{u^\beta}{k_2{}^2.k_1{}^2.(\,k_1-p\,)^2.(\,-k_1+k_2+p\,)^2}\right)$$

$$\tilde{\Pi}_{20}^{\mu\beta}(p,k_1,k_2) = 2\,i\,\mathrm{e}^4\,Q_1\,(2\,k_1{}^\mu - p^\mu)\left(\frac{(\xi-1)\left(-p^\beta+k_1{}^\beta-k_2{}^\beta\right)(-p\cdot u+k_1\cdot u-k_2\cdot u)}{k_2{}^2.k_1{}^2.(\,k_1-p\,)^2.(\,-k_1+k_2+p\,)^{22}} + \frac{u^\beta}{k_2{}^2.k_1{}^2.(\,k_1-p\,)^2.(\,-k_1+k_2+p\,)^2}\right)$$

$$\tilde{\Pi}_{21}^{\mu\beta}(p,k_1,k_2) = \frac{i\,\mathrm{e}^2\,\lambda\,Q_1\,u^\beta\,(2\,k_1{}^\mu - p^\mu)}{k_1{}^2.k_2{}^2.(\,k_1-p\,)^{22}}$$

$$\tilde{\Pi}_{22}^{\mu\beta}(p,k_1,k_2) = -\frac{i\,\mathrm{e}^2\,\lambda\,Q_1\,u^\beta\,(2\,k_1{}^\mu - p^\mu)}{k_1{}^2.k_2{}^2.(\,k_1-p\,)^{22}}$$

$$\tilde{\Pi}_{23}^{\mu\beta}(p,k_1,k_2) = i\,\mathrm{e}^4\,Q_1\,u^\beta\,(2\,k_1{}^\mu - p^\mu)\left(\frac{D}{k_1{}^2.k_2{}^2.(\,k_1-p\,)^{22}} + \frac{(\xi-1)\,k_2{}^2}{k_1{}^2.\left(k_2{}^2\right)^2.(\,k_1-p\,)^{22}}\right)$$

$$\tilde{\Pi}_{24}^{\mu\beta}(p,k_1,k_2) = -i\,\mathrm{e}^4\,Q_1\,u^\beta\,(2\,k_1{}^\mu - p^\mu)\left(\frac{D}{k_1{}^2.k_2{}^2.(\,k_1-p\,)^{22}} + \frac{(\xi-1)\,k_2{}^2}{k_1{}^2.\left(k_2{}^2\right)^2.(\,k_1-p\,)^{22}}\right)$$

$$\tilde{\Pi}_{25}^{\mu\beta}(p,k_1,k_2) = -4\,i\,\mathrm{e}^4\,Q_1\,(k_1\cdot u)\left(\frac{g^{\mu\,\beta}}{k_1{}^2.k_2{}^2.k_1{}^2.(\,-k_1+k_2+p\,)^2} + \frac{(\xi-1)\left(-p^\beta+k_1{}^\beta-k_2{}^\beta\right)(-p^\mu+k_1{}^\mu-k_2{}^\mu)}{k_1{}^2.k_2{}^2.k_1{}^2.(\,-k_1+k_2+p\,)^{22}}\right)$$

$$\tilde{\Pi}_{26}^{\mu\beta}(p,k_1,k_2) = 4\,i\,\mathrm{e}^4\,Q_1\,(k_1\cdot u)\left(\frac{g^{\mu\,\beta}}{k_1{}^2.k_2{}^2.k_1{}^2.(\,-k_1+k_2+p\,)^2} + \frac{(\xi-1)\left(-p^\beta+k_1{}^\beta-k_2{}^\beta\right)(-p^\mu+k_1{}^\mu-k_2{}^\mu)}{k_1{}^2.k_2{}^2.k_1{}^2.(\,-k_1+k_2+p\,)^{22}}\right)$$

$$\tilde{\Pi}_{27}^{\mu\beta}(p,k_1,k_2) = \frac{8\,\mathrm{e}^4\,Q_2\,\epsilon^{\beta\,\mu\,b\,k_1}}{k_1{}^2.k_2{}^2.k_1{}^2.(\,-k_1+k_2+p\,)^2}$$

$$\tilde{\Pi}_{28}^{\mu\beta}(p,k_1,k_2) = -2\,i\,\mathrm{e}^4\,Q_1\left(p^\beta+2\,k_1{}^\beta\right)\left(\frac{(\xi-1)\,(k_1{}^\mu-k_2{}^\mu)\,(k_1\cdot u-k_2\cdot u)}{k_2{}^2.k_1{}^2.(\,k_1+p\,)^2.(\,k_2-k_1\,)^{22}} + \frac{u^\mu}{k_2{}^2.k_1{}^2.(\,k_1+p\,)^2.(\,k_2-k_1\,)^2}\right)$$

$$\tilde{\Pi}_{29}^{\mu\beta}(p,k_1,k_2) = 2\,i\,\mathrm{e}^4\,Q_1\left(p^\beta+2\,k_1{}^\beta\right)\left(\frac{(\xi-1)\,(k_1{}^\mu-k_2{}^\mu)\,(k_1\cdot u-k_2\cdot u)}{k_2{}^2.k_1{}^2.(\,k_1+p\,)^2.(\,k_2-k_1\,)^{22}} + \frac{u^\mu}{k_2{}^2.k_1{}^2.(\,k_1+p\,)^2.(\,k_2-k_1\,)^2}\right)$$

$$\tilde{\Pi}_{30}^{\mu\beta}(p,k_1,k_2) = -2\,i\,\mathrm{e}^4\,Q_1\,u^\beta\left(\frac{(\xi-1)\,k_2{}^\mu\left(2\,(k_1\cdot k_2)+k_2{}^2\right)}{\left(k_2{}^2\right)^2.k_1{}^2.(\,k_1+k_2\,)^2.(\,k_1+k_2+p\,)^2} + \frac{2\,k_1{}^\mu+k_2{}^\mu}{k_2{}^2.k_1{}^2.(\,k_1+k_2\,)^2.(\,k_1+k_2+p\,)^2}\right)$$

$$\tilde{\Pi}_{31}^{\mu\beta}(p,k_1,k_2) = 2\,i\,\mathrm{e}^4\,Q_1\,u^\beta\left(\frac{(\xi-1)\,k_2{}^\mu\left(2\,(k_1\cdot k_2)+k_2{}^2\right)}{\left(k_2{}^2\right)^2.k_1{}^2.(\,k_1+k_2\,)^2.(\,k_1+k_2+p\,)^2} + \frac{2\,k_1{}^\mu+k_2{}^\mu}{k_2{}^2.k_1{}^2.(\,k_1+k_2\,)^2.(\,k_1+k_2+p\,)^2}\right)$$

$$\tilde{\Pi}_{32}^{\mu\beta}(p,k_1,k_2) = \frac{2\,i\,\mathrm{e}^2\,\lambda\,Q_1\,g^{\mu\,\beta}\,(k_1\cdot u)}{\left(k_1{}^2\right)^3.k_2{}^2}$$

$$\tilde{\Pi}_{33}^{\mu\beta}(p,k_1,k_2) = -\frac{2\,i\,\mathrm{e}^2\,\lambda\,Q_1\,g^{\mu\,\beta}\,(k_1\cdot u)}{\left(k_1{}^2\right)^3.k_2{}^2}$$

$$\tilde{\Pi}_{34}^{\mu\beta}(p,k_1,k_2) = 2\,i\,\mathrm{e}^4\,Q_1\,g^{\mu\,\beta}\,(k_1\cdot u)\left(\frac{D}{\left(k_1{}^2\right)^3.k_2{}^2} + \frac{(\xi-1)\,k_2{}^2}{\left(k_1{}^2\right)^3.\left(k_2{}^2\right)^2}\right)$$

$$\tilde{\Pi}^{\mu\beta}_{35}(p,\, k_1,\, k_2) = -2\, i\, \mathrm{e}^4\, Q_1\, g^{\mu\,\beta}\, (k_1 \cdot u) \left( \frac{D}{(k_1{}^2)^3 . k_2{}^2} + \frac{(\xi - 1)\, k_2{}^2}{(k_1{}^2)^3 . (k_2{}^2)^2} \right)$$

$$\tilde{\Pi}^{\mu\beta}_{36}(p,\, k_1,\, k_2) = -2\, i\, \mathrm{e}^4\, Q_1\, g^{\mu\,\beta} \left( \frac{(\xi - 1)\left(2\,(k_1 \cdot k_2) + k_2{}^2\right)(k_2 \cdot u)}{(k_2{}^2)^2 . k_1{}^2 . (\,k_1 + k_2\,)^{22}} + \frac{2\,(k_1 \cdot u) + k_2 \cdot u}{k_2{}^2 . k_1{}^2 . (\,k_1 + k_2\,)^{22}} \right)$$

$$\tilde{\Pi}^{\mu\beta}_{37}(p,\, k_1,\, k_2) = 2\, i\, \mathrm{e}^4\, Q_1\, g^{\mu\,\beta} \left( \frac{(\xi - 1)\left(2\,(k_1 \cdot k_2) + k_2{}^2\right)(k_2 \cdot u)}{(k_2{}^2)^2 . k_1{}^2 . (\,k_1 + k_2\,)^{22}} + \frac{2\,(k_1 \cdot u) + k_2 \cdot u}{k_2{}^2 . k_1{}^2 . (\,k_1 + k_2\,)^{22}} \right)$$

$$\tilde{\Pi}^{\mu\beta}_{38}(p,\, k_1,\, k_2) = \frac{i\, \mathrm{e}^2\, \lambda\, Q_1\, u^\mu \left(p^\beta + 2\, k_1{}^\beta\right)}{k_1{}^2 . k_2{}^2 . (\,k_1 + p\,)^{22}}$$

$$\tilde{\Pi}^{\mu\beta}_{39}(p,\, k_1,\, k_2) = -\frac{i\, \mathrm{e}^2\, \lambda\, Q_1\, u^\mu \left(p^\beta + 2\, k_1{}^\beta\right)}{k_1{}^2 . k_2{}^2 . (\,k_1 + p\,)^{22}}$$

$$\tilde{\Pi}^{\mu\beta}_{40}(p,\, k_1,\, k_2) = i\, \mathrm{e}^4\, Q_1\, u^\mu \left(p^\beta + 2\, k_1{}^\beta\right) \left( \frac{D}{k_1{}^2 . k_2{}^2 . (\,k_1 + p\,)^{22}} + \frac{(\xi - 1)\, k_2{}^2}{k_1{}^2 . (k_2{}^2)^2 . (\,k_1 + p\,)^{22}} \right)$$

$$\tilde{\Pi}^{\mu\beta}_{41}(p,\, k_1,\, k_2) = -i\, \mathrm{e}^4\, Q_1\, u^\mu \left(p^\beta + 2\, k_1{}^\beta\right) \left( \frac{D}{k_1{}^2 . k_2{}^2 . (\,k_1 + p\,)^{22}} + \frac{(\xi - 1)\, k_2{}^2}{k_1{}^2 . (k_2{}^2)^2 . (\,k_1 + p\,)^{22}} \right)$$

$$\tilde{\Pi}^{\mu\beta}_{42}(p,\, k_1,\, k_2) = -2\, i\, \mathrm{e}^4\, Q_1\, u^\mu \left( \frac{(\xi - 1)\, k_2{}^\beta \left(2\,(k_1 \cdot k_2) + k_2{}^2\right)}{(k_2{}^2)^2 . k_1{}^2 . (\,k_1 + k_2\,)^2 . (\,k_1 + k_2 - p\,)^2} + \frac{2\, k_1{}^\beta + k_2{}^\beta}{k_2{}^2 . k_1{}^2 . (\,k_1 + k_2\,)^2 . (\,k_1 + k_2 - p\,)^2} \right)$$

$$\tilde{\Pi}^{\mu\beta}_{43}(p,\, k_1,\, k_2) = 2\, i\, \mathrm{e}^4\, Q_1\, u^\mu \left( \frac{(\xi - 1)\, k_2{}^\beta \left(2\,(k_1 \cdot k_2) + k_2{}^2\right)}{(k_2{}^2)^2 . k_1{}^2 . (\,k_1 + k_2\,)^2 . (\,k_1 + k_2 - p\,)^2} + \frac{2\, k_1{}^\beta + k_2{}^\beta}{k_2{}^2 . k_1{}^2 . (\,k_1 + k_2\,)^2 . (\,k_1 + k_2 - p\,)^2} \right)$$

$$\tilde{\Pi}^{\mu\beta}_{44}(p,\, k_1,\, k_2) = -\frac{i\, \mathrm{e}^2\, \lambda\, Q_1 \left(2\, k_1{}^\beta - p^\beta\right)(2\, k_1{}^\mu - p^\mu)\,(k_1 \cdot u)}{(k_1{}^2)^3 . k_2{}^2 . (\,k_1 - p\,)^2}$$

$$\tilde{\Pi}^{\mu\beta}_{45}(p,\, k_1,\, k_2) = \frac{i\, \mathrm{e}^2\, \lambda\, Q_1 \left(2\, k_1{}^\beta - p^\beta\right)(2\, k_1{}^\mu - p^\mu)\,(k_1 \cdot u)}{(k_1{}^2)^3 . k_2{}^2 . (\,k_1 - p\,)^2}$$

$$\tilde{\Pi}^{\mu\beta}_{46}(p,\, k_1,\, k_2) = -i\, \mathrm{e}^4\, Q_1 \left(2\, k_1{}^\beta - p^\beta\right)(2\, k_1{}^\mu - p^\mu)\,(k_1 \cdot u) \left( \frac{D}{(k_1{}^2)^3 . k_2{}^2 . (\,k_1 - p\,)^2} + \frac{(\xi - 1)\, k_2{}^2}{(k_1{}^2)^3 . (k_2{}^2)^2 . (\,k_1 - p\,)^2} \right)$$

$$\tilde{\Pi}^{\mu\beta}_{47}(p,\, k_1,\, k_2) = i\, \mathrm{e}^4\, Q_1 \left(2\, k_1{}^\beta - p^\beta\right)(2\, k_1{}^\mu - p^\mu)\,(k_1 \cdot u) \left( \frac{D}{(k_1{}^2)^3 . k_2{}^2 . (\,k_1 - p\,)^2} + \frac{(\xi - 1)\, k_2{}^2}{(k_1{}^2)^3 . (k_2{}^2)^2 . (\,k_1 - p\,)^2} \right)$$

$$\tilde{\Pi}^{\mu\beta}_{48}(p,\, k_1,\, k_2) = -\frac{i\, \mathrm{e}^2\, \lambda\, Q_1 \left(2\, k_1{}^\beta - p^\beta\right)(2\, k_1{}^\mu - p^\mu)\,(k_1 \cdot u)}{(k_1{}^2)^2 . k_2{}^2 . (\,k_1 - p\,)^{22}}$$

$$\tilde{\Pi}^{\mu\beta}_{49}(p,\, k_1,\, k_2) = \frac{i\, \mathrm{e}^2\, \lambda\, Q_1 \left(2\, k_1{}^\beta - p^\beta\right)(2\, k_1{}^\mu - p^\mu)\,(k_1 \cdot u)}{(k_1{}^2)^2 . k_2{}^2 . (\,k_1 - p\,)^{22}}$$

$$\tilde{\Pi}^{\mu\beta}_{50}(p,\, k_1,\, k_2) = -i\, \mathrm{e}^4\, Q_1 \left(2\, k_1{}^\beta - p^\beta\right)(2\, k_1{}^\mu - p^\mu)\,(k_1 \cdot u) \left( \frac{D}{(k_1{}^2)^2 . k_2{}^2 . (\,k_1 - p\,)^{22}} + \frac{(\xi - 1)\, k_2{}^2}{(k_1{}^2)^2 . (k_2{}^2)^2 . (\,k_1 - p\,)^{22}} \right)$$

$$\tilde{\Pi}^{\mu\beta}_{51}(p,\, k_1,\, k_2) = i\, \mathrm{e}^4\, Q_1 \left(2\, k_1{}^\beta - p^\beta\right)(2\, k_1{}^\mu - p^\mu)\,(k_1 \cdot u) \left( \frac{D}{(k_1{}^2)^2 . k_2{}^2 . (\,k_1 - p\,)^{22}} + \frac{(\xi - 1)\, k_2{}^2}{(k_1{}^2)^2 . (k_2{}^2)^2 . (\,k_1 - p\,)^{22}} \right)$$

$$\tilde{\Pi}^{\mu\beta}_{52}(p,\, k_1,\, k_2) = -\frac{i\, \mathrm{e}^2\, \lambda\, Q_1\, (2\, k_1{}^\mu - p^\mu) \left(p^\beta + 2\, k_2{}^\beta\right)(k_1 \cdot u)}{(k_1{}^2)^2 . k_2{}^2 . (\,k_1 - p\,)^2 . (\,k_2 + p\,)^2}$$

$$\tilde{\Pi}^{\mu\beta}_{53}(p,\, k_1,\, k_2) = -\frac{i\, \mathrm{e}^2\, \lambda\, Q_1\, (2\, k_1{}^\mu - p^\mu) \left(p^\beta + 2\, k_2{}^\beta\right)(k_1 \cdot u)}{(k_1{}^2)^2 . k_2{}^2 . (\,k_1 - p\,)^2 . (\,k_2 + p\,)^2}$$

$$\tilde{\Pi}^{\mu\beta}_{54}(p, k_1, k_2) = -\frac{i\, e^2\, \lambda\, Q_1 \left(2\, k_1{}^{\beta} - p^{\beta}\right) (2\, k_1{}^{\mu} - p^{\mu})\, (k_1 \cdot u - p \cdot u)}{k_1{}^2 . k_2{}^2 . (k_1 - p)^{23}}$$

$$\tilde{\Pi}^{\mu\beta}_{55}(p, k_1, k_2) = \frac{i\, e^2\, \lambda\, Q_1 \left(2\, k_1{}^{\beta} - p^{\beta}\right) (2\, k_1{}^{\mu} - p^{\mu})\, (k_1 \cdot u - p \cdot u)}{k_1{}^2 . k_2{}^2 . (k_1 - p)^{23}}$$

$$\tilde{\Pi}^{\mu\beta}_{56}(p, k_1, k_2) = -i\, e^4\, Q_1 \left(2\, k_1{}^{\beta} - p^{\beta}\right) (2\, k_1{}^{\mu} - p^{\mu})\, (k_1 \cdot u - p \cdot u) \left(\frac{D}{k_1{}^2 . k_2{}^2 . (k_1 - p)^{23}} + \frac{(\xi - 1)\, k_2{}^2}{k_1{}^2 . \left(k_2{}^2\right)^2 . (k_1 - p)^{23}}\right)$$

$$\tilde{\Pi}^{\mu\beta}_{57}(p, k_1, k_2) = i\, e^4\, Q_1 \left(2\, k_1{}^{\beta} - p^{\beta}\right) (2\, k_1{}^{\mu} - p^{\mu})\, (k_1 \cdot u - p \cdot u) \left(\frac{D}{k_1{}^2 . k_2{}^2 . (k_1 - p)^{23}} + \frac{(\xi - 1)\, k_2{}^2}{k_1{}^2 . \left(k_2{}^2\right)^2 . (k_1 - p)^{23}}\right)$$

$$\tilde{\Pi}^{\mu\beta}_{58}(p, k_1, k_2) = -\frac{i\, e^2\, \lambda\, Q_1 \left(2\, k_1{}^{\beta} - p^{\beta}\right) (2\, k_1{}^{\mu} - p^{\mu})\, (k_2 \cdot u)}{k_1{}^2 . \left(k_2{}^2\right)^2 . (k_1 - p)^{22}}$$

$$\tilde{\Pi}^{\mu\beta}_{59}(p, k_1, k_2) = -\frac{i\, e^2\, \lambda\, Q_1 \left(2\, k_1{}^{\beta} - p^{\beta}\right) (2\, k_1{}^{\mu} - p^{\mu})\, (k_2 \cdot u)}{k_1{}^2 . \left(k_2{}^2\right)^2 . (k_1 - p)^{22}}$$

$$\tilde{\Pi}^{\mu\beta}_{60}(p, k_1, k_2) = 0$$

$$\tilde{\Pi}^{\mu\beta}_{61}(p, k_1, k_2) = 0$$

$$\tilde{\Pi}^{\mu\beta}_{62}(p, k_1, k_2) = -\frac{i\, e^2\, \lambda\, Q_1\, (2\, k_1{}^{\mu} - p^{\mu}) \left(2\, k_2{}^{\beta} - p^{\beta}\right) (k_2 \cdot u)}{\left(k_2{}^2\right)^2 . k_1{}^2 . (k_2 - p)^2 . (k_1 - p)^2}$$

$$\tilde{\Pi}^{\mu\beta}_{63}(p, k_1, k_2) = -\frac{i\, e^2\, \lambda\, Q_1\, (2\, k_1{}^{\mu} - p^{\mu}) \left(2\, k_2{}^{\beta} - p^{\beta}\right) (k_2 \cdot u)}{\left(k_2{}^2\right)^2 . k_1{}^2 . (k_2 - p)^2 . (k_1 - p)^2}$$

$$\tilde{\Pi}^{\mu\beta}_{64}(p, k_1, k_2) = 2\, i\, e^4\, Q_1\, (2\, k_1{}^{\mu} - p^{\mu})\, (k_1 \cdot u) \left(\frac{(\xi - 1) \left(-p^{\beta} + k_1{}^{\beta} + k_2{}^{\beta}\right) \left(-2\, (k_1 \cdot p) + p^2 + k_1{}^2 - k_2{}^2\right)}{k_1{}^2 . k_2{}^2 . k_1{}^2 . (k_1 - p)^2 . (k_1 + k_2 - p)^{22}} + \frac{-p^{\beta} + k_1{}^{\beta} - k_2{}^{\beta}}{k_1{}^2 . k_2{}^2 . k_1{}^2 . (k_1 - p)^2 . (k_1 + k_2 - p)^2}\right)$$

$$\tilde{\Pi}^{\mu\beta}_{65}(p, k_1, k_2) = -2\, i\, e^4\, Q_1\, (2\, k_1{}^{\mu} - p^{\mu})\, (k_1 \cdot u) \left(\frac{(\xi - 1) \left(-p^{\beta} + k_1{}^{\beta} + k_2{}^{\beta}\right) \left(-2\, (k_1 \cdot p) + p^2 + k_1{}^2 - k_2{}^2\right)}{k_1{}^2 . k_2{}^2 . k_1{}^2 . (k_1 - p)^2 . (k_1 + k_2 - p)^{22}} + \frac{-p^{\beta} + k_1{}^{\beta} - k_2{}^{\beta}}{k_1{}^2 . k_2{}^2 . k_1{}^2 . (k_1 - p)^2 . (k_1 + k_2 - p)^2}\right)$$

$$\tilde{\Pi}^{\mu\beta}_{66}(p, k_1, k_2) = -2\, i\, e^4\, Q_1\, (2\, k_1{}^{\mu} - p^{\mu})\, (k_1 \cdot u) \left(\frac{(\xi - 1) \left(k_1{}^2 - k_2{}^2\right) \left(k_1{}^{\beta} - k_2{}^{\beta}\right)}{k_1{}^2 . k_2{}^2 . k_1{}^2 . (k_1 - p)^2 . (k_2 - k_1)^{22}} + \frac{k_1{}^{\beta} + k_2{}^{\beta}}{k_1{}^2 . k_2{}^2 . k_1{}^2 . (k_1 - p)^2 . (k_2 - k_1)^2}\right)$$

$$\tilde{\Pi}^{\mu\beta}_{67}(p, k_1, k_2) = 2\, i\, e^4\, Q_1\, (2\, k_1{}^{\mu} - p^{\mu})\, (k_1 \cdot u) \left(\frac{(\xi - 1) \left(k_1{}^2 - k_2{}^2\right) \left(k_1{}^{\beta} - k_2{}^{\beta}\right)}{k_1{}^2 . k_2{}^2 . k_1{}^2 . (k_1 - p)^2 . (k_2 - k_1)^{22}} + \frac{k_1{}^{\beta} + k_2{}^{\beta}}{k_1{}^2 . k_2{}^2 . k_1{}^2 . (k_1 - p)^2 . (k_2 - k_1)^2}\right)$$

$$\tilde{\Pi}^{\mu\beta}_{68}(p, k_1, k_2) = i\, e^4\, Q_1 \left(2\, k_1{}^{\beta} - p^{\beta}\right) (2\, k_1{}^{\mu} - p^{\mu}) \left(\frac{(\xi - 1) \left(-2\, (k_1 \cdot p) + p^2 + k_1{}^2 - k_2{}^2\right) (-p \cdot u + k_1 \cdot u + k_2 \cdot u)}{k_2{}^2 . k_1{}^2 . (k_1 - p)^{22} . (k_1 + k_2 - p)^{22}} + \frac{-p \cdot u + k_1 \cdot u - k_2 \cdot u}{k_2{}^2 . k_1{}^2 . (k_1 - p)^{22} . (k_1 + k_2 - p)^2}\right)$$

$$\tilde{\Pi}^{\mu\beta}_{69}(p, k_1, k_2) = -i\, e^4\, Q_1 \left(2\, k_1{}^{\beta} - p^{\beta}\right) (2\, k_1{}^{\mu} - p^{\mu}) \left(\frac{(\xi - 1) \left(-2\, (k_1 \cdot p) + p^2 + k_1{}^2 - k_2{}^2\right) (-p \cdot u + k_1 \cdot u + k_2 \cdot u)}{k_2{}^2 . k_1{}^2 . (k_1 - p)^{22} . (k_1 + k_2 - p)^{22}} + \frac{-p \cdot u + k_1 \cdot u - k_2 \cdot u}{k_2{}^2 . k_1{}^2 . (k_1 - p)^{22} . (k_1 + k_2 - p)^2}\right)$$

$$\tilde{\Pi}^{\mu\beta}_{70}(p, k_1, k_2) = -i\, e^4\, Q_1 \left(2\, k_1{}^{\beta} - p^{\beta}\right) (2\, k_1{}^{\mu} - p^{\mu}) \left(\frac{(\xi - 1) \left(-2\, (k_1 \cdot p) + p^2 + k_1{}^2 - k_2{}^2\right) (-p \cdot u + k_1 \cdot u - k_2 \cdot u)}{k_2{}^2 . k_1{}^2 . (k_1 - p)^{22} . (-k_1 + k_2 + p)^{22}} + \frac{-p \cdot u + k_1 \cdot u + k_2 \cdot u}{k_2{}^2 . k_1{}^2 . (k_1 - p)^{22} . (-k_1 + k_2 + p)^2}\right)$$

$$\tilde{\Pi}^{\mu\beta}_{71}(p, k_1, k_2) = i\, e^4\, Q_1 \left(2\, k_1{}^{\beta} - p^{\beta}\right) (2\, k_1{}^{\mu} - p^{\mu}) \left(\frac{(\xi - 1) \left(-2\, (k_1 \cdot p) + p^2 + k_1{}^2 - k_2{}^2\right) (-p \cdot u + k_1 \cdot u - k_2 \cdot u)}{k_2{}^2 . k_1{}^2 . (k_1 - p)^{22} . (-k_1 + k_2 + p)^{22}} + \frac{-p \cdot u + k_1 \cdot u + k_2 \cdot u}{k_2{}^2 . k_1{}^2 . (k_1 - p)^{22} . (-k_1 + k_2 + p)^2}\right)$$

$$\tilde{\Pi}^{\mu\beta}_{72}(p, k_1, k_2) = i\,\mathrm{e}^4\, Q_1\, u^\beta\, (p^\mu + 2\,k_1{}^\mu) \left( \frac{(\xi - 1)\left(k_1{}^2 - k_2{}^2\right)^2}{k_2{}^2.\left(k_1{}^2\right)^2.(\,k_1 + p\,)^2.(\,k_2 - k_1\,)^{22}} + \frac{2\,(k_1 \cdot k_2) + k_1{}^2 + k_2{}^2}{k_2{}^2.\left(k_1{}^2\right)^2.(\,k_1 + p\,)^2.(\,k_2 - k_1\,)^2} \right)$$

$$\tilde{\Pi}^{\mu\beta}_{73}(p, k_1, k_2) = -i\,\mathrm{e}^4\, Q_1\, u^\beta\, (p^\mu + 2\,k_1{}^\mu) \left( \frac{(\xi - 1)\left(k_1{}^2 - k_2{}^2\right)^2}{k_2{}^2.\left(k_1{}^2\right)^2.(\,k_1 + p\,)^2.(\,k_2 - k_1\,)^{22}} + \frac{2\,(k_1 \cdot k_2) + k_1{}^2 + k_2{}^2}{k_2{}^2.\left(k_1{}^2\right)^2.(\,k_1 + p\,)^2.(\,k_2 - k_1\,)^2} \right)$$

$$\tilde{\Pi}^{\mu\beta}_{74}(p, k_1, k_2) =$$
$$-i\,\mathrm{e}^4\, Q_1\, u^\beta\, (p^\mu + 2\,k_1{}^\mu) \left( \frac{(\xi - 1)\left(2\,(k_1 \cdot k_2) - k_2{}^2\right)\left(2\,(k_2 \cdot p) + 2\,(k_1 \cdot k_2) - k_2{}^2\right)}{\left(k_2{}^2\right)^2.k_1{}^2.(\,k_1 + p\,)^2.(\,k_1 - k_2\,)^2.(\,-k_1 + k_2 - p\,)^2} + \frac{4\,(k_1 \cdot p) - 2\,(k_2 \cdot p) - 4\,(k_1 \cdot k_2) + 4\,k_1{}^2 + k_2{}^2}{k_2{}^2.k_1{}^2.(\,k_1 + p\,)^2.(\,k_1 - k_2\,)^2.(\,-k_1 + k_2 - p\,)^2} \right)$$

$$\tilde{\Pi}^{\mu\beta}_{75}(p, k_1, k_2) = 2\,i\,\mathrm{e}^4\, Q_1 \left(2\,k_1{}^\beta - p^\beta\right)(k_1 \cdot u) \left( \frac{(\xi - 1)\left(k_1{}^2 - k_2{}^2\right)(k_1{}^\mu + k_2{}^\mu)}{k_1{}^2.k_2{}^2.k_1{}^2.(\,k_1 - p\,)^2.(\,k_1 + k_2\,)^{22}} + \frac{k_1{}^\mu - k_2{}^\mu}{k_1{}^2.k_2{}^2.k_1{}^2.(\,k_1 - p\,)^2.(\,k_1 + k_2\,)^2} \right)$$

$$\tilde{\Pi}^{\mu\beta}_{76}(p, k_1, k_2) = -2\,i\,\mathrm{e}^4\, Q_1 \left(2\,k_1{}^\beta - p^\beta\right)(k_1 \cdot u) \left( \frac{(\xi - 1)\left(k_1{}^2 - k_2{}^2\right)(k_1{}^\mu + k_2{}^\mu)}{k_1{}^2.k_2{}^2.k_1{}^2.(\,k_1 - p\,)^2.(\,k_1 + k_2\,)^{22}} + \frac{k_1{}^\mu - k_2{}^\mu}{k_1{}^2.k_2{}^2.k_1{}^2.(\,k_1 - p\,)^2.(\,k_1 + k_2\,)^2} \right)$$

$$\tilde{\Pi}^{\mu\beta}_{77}(p, k_1, k_2) =$$
$$-2\,i\,\mathrm{e}^4\, Q_1 \left(2\,k_1{}^\beta - p^\beta\right)(k_1 \cdot u) \left( \frac{(\xi - 1)\,(-p^\mu + k_1{}^\mu - k_2{}^\mu)\left(-2\,(k_1 \cdot p) + p^2 + k_1{}^2 - k_2{}^2\right)}{k_1{}^2.k_2{}^2.k_1{}^2.(\,k_1 - p\,)^2.(\,-k_1 + k_2 + p\,)^{22}} + \frac{-p^\mu + k_1{}^\mu + k_2{}^\mu}{k_1{}^2.k_2{}^2.k_1{}^2.(\,k_1 - p\,)^2.(\,-k_1 + k_2 + p\,)^2} \right)$$

$$\tilde{\Pi}^{\mu\beta}_{78}(p, k_1, k_2) = 2\,i\,\mathrm{e}^4\, Q_1 \left(2\,k_1{}^\beta - p^\beta\right)(k_1 \cdot u)$$
$$\left( \frac{(\xi - 1)\,(-p^\mu + k_1{}^\mu - k_2{}^\mu)\left(-2\,(k_1 \cdot p) + p^2 + k_1{}^2 - k_2{}^2\right)}{k_1{}^2.k_2{}^2.k_1{}^2.(\,k_1 - p\,)^2.(\,-k_1 + k_2 + p\,)^{22}} + \frac{-p^\mu + k_1{}^\mu + k_2{}^\mu}{k_1{}^2.k_2{}^2.k_1{}^2.(\,k_1 - p\,)^2.(\,-k_1 + k_2 + p\,)^2} \right)$$

$$\tilde{\Pi}^{\mu\beta}_{79}(p, k_1, k_2) = 2\,i\,\mathrm{e}^4\, Q_1\, g^{\mu\,\beta}\, (k_1 \cdot u) \left( \frac{(\xi - 1)\left(k_1{}^2 - k_2{}^2\right)^2}{k_1{}^2.k_2{}^2.\left(k_1{}^2\right)^2.(\,k_2 - k_1\,)^{22}} + \frac{2\,(k_1 \cdot k_2) + k_1{}^2 + k_2{}^2}{k_1{}^2.k_2{}^2.\left(k_1{}^2\right)^2.(\,k_2 - k_1\,)^2} \right)$$

$$\tilde{\Pi}^{\mu\beta}_{80}(p, k_1, k_2) = -2\,i\,\mathrm{e}^4\, Q_1\, g^{\mu\,\beta}\, (k_1 \cdot u) \left( \frac{(\xi - 1)\left(k_1{}^2 - k_2{}^2\right)^2}{k_1{}^2.k_2{}^2.\left(k_1{}^2\right)^2.(\,k_2 - k_1\,)^{22}} + \frac{2\,(k_1 \cdot k_2) + k_1{}^2 + k_2{}^2}{k_1{}^2.k_2{}^2.\left(k_1{}^2\right)^2.(\,k_2 - k_1\,)^2} \right)$$

$$\tilde{\Pi}^{\mu\beta}_{81}(p, k_1, k_2) = -2\,i\,\mathrm{e}^4\, Q_1\, g^{\mu\,\beta}\, (k_1 \cdot u) \left( \frac{(\xi - 1)\left(k_2{}^2 - 2\,(k_1 \cdot k_2)\right)^2}{k_1{}^2.\left(k_2{}^2\right)^2.k_1{}^2.(\,k_2 - k_1\,)^2.(\,k_1 - k_2\,)^2} + \frac{-4\,(k_1 \cdot k_2) + 4\,k_1{}^2 + k_2{}^2}{k_1{}^2.k_2{}^2.k_1{}^2.(\,k_2 - k_1\,)^2.(\,k_1 - k_2\,)^2} \right)$$

$$\tilde{\Pi}^{\mu\beta}_{82}(p, k_1, k_2) = 0$$

$$\tilde{\Pi}^{\mu\beta}_{83}(p, k_1, k_2) = i\,\mathrm{e}^4\, Q_1\, u^\mu \left(2\,k_1{}^\beta - p^\beta\right) \left( \frac{(\xi - 1)\left(k_1{}^2 - k_2{}^2\right)^2}{k_2{}^2.\left(k_1{}^2\right)^2.(\,k_1 - p\,)^2.(\,k_2 - k_1\,)^{22}} + \frac{2\,(k_1 \cdot k_2) + k_1{}^2 + k_2{}^2}{k_2{}^2.\left(k_1{}^2\right)^2.(\,k_1 - p\,)^2.(\,k_2 - k_1\,)^2} \right)$$

$$\tilde{\Pi}^{\mu\beta}_{84}(p, k_1, k_2) = -i\,\mathrm{e}^4\, Q_1\, u^\mu \left(2\,k_1{}^\beta - p^\beta\right) \left( \frac{(\xi - 1)\left(k_1{}^2 - k_2{}^2\right)^2}{k_2{}^2.\left(k_1{}^2\right)^2.(\,k_1 - p\,)^2.(\,k_2 - k_1\,)^{22}} + \frac{2\,(k_1 \cdot k_2) + k_1{}^2 + k_2{}^2}{k_2{}^2.\left(k_1{}^2\right)^2.(\,k_1 - p\,)^2.(\,k_2 - k_1\,)^2} \right)$$

$$\tilde{\Pi}^{\mu\beta}_{85}(p, k_1, k_2) = -i\,\mathrm{e}^4\, Q_1\, u^\mu \left(2\,k_1{}^\beta - p^\beta\right)$$
$$\left( \frac{(\xi - 1)\left(2\,(k_1 \cdot k_2) - k_2{}^2\right)\left(-2\,(k_2 \cdot p) + 2\,(k_1 \cdot k_2) - k_2{}^2\right)}{\left(k_2{}^2\right)^2.k_1{}^2.(\,k_1 - p\,)^2.(\,k_1 - k_2\,)^2.(\,-k_1 + k_2 + p\,)^2} + \frac{-4\,(k_1 \cdot p) + 2\,(k_2 \cdot p) - 4\,(k_1 \cdot k_2) + 4\,k_1{}^2 + k_2{}^2}{k_2{}^2.k_1{}^2.(\,k_1 - p\,)^2.(\,k_1 - k_2\,)^2.(\,-k_1 + k_2 + p\,)^2} \right)$$

$$\tilde{\Pi}^{\mu\beta}_{86}(p, k_1, k_2) = \frac{8\,\mathrm{e}^4\, Q_2\, (p^\mu + 2\,k_1{}^\mu)\left(p^\beta + 2\,k_1{}^\beta + 2\,k_2{}^\beta\right)\epsilon^{b\,k_1\,k_2\,p}}{\left(k_2{}^2\right)^2.k_1{}^2.(\,k_1 + p\,)^2.(\,k_1 + k_2\,)^2.(\,k_1 + k_2 + p\,)^2}$$

$$\tilde{\Pi}^{\mu\beta}_{87}(p, k_1, k_2) = -i\,\mathrm{e}^4\, Q_1 \left(2\,k_1{}^\beta - p^\beta\right)(2\,k_1{}^\mu - p^\mu)\,(k_1 \cdot u)$$
$$\left( \frac{(\xi - 1)\left(-2\,(k_1 \cdot p) + p^2 + k_1{}^2 - k_2{}^2\right)^2}{k_1{}^2.k_2{}^2.k_1{}^2.(\,k_1 - p\,)^{22}.(\,-k_1 + k_2 + p\,)^{22}} + \frac{-2\,(k_1 \cdot p) - 2\,(k_2 \cdot p) + p^2 + 2\,(k_1 \cdot k_2) + k_1{}^2 + k_2{}^2}{k_1{}^2.k_2{}^2.k_1{}^2.(\,k_1 - p\,)^{22}.(\,-k_1 + k_2 + p\,)^2} \right)$$

$$\tilde{\Pi}^{\mu\beta}_{88}(p, k_1, k_2) = i\,\mathrm{e}^4\, Q_1 \left(2\,k_1{}^\beta - p^\beta\right)(2\,k_1{}^\mu - p^\mu)\,(k_1 \cdot u)$$
$$\left( \frac{(\xi - 1)\left(-2\,(k_1 \cdot p) + p^2 + k_1{}^2 - k_2{}^2\right)^2}{k_1{}^2.k_2{}^2.k_1{}^2.(\,k_1 - p\,)^{22}.(\,-k_1 + k_2 + p\,)^{22}} + \frac{-2\,(k_1 \cdot p) - 2\,(k_2 \cdot p) + p^2 + 2\,(k_1 \cdot k_2) + k_1{}^2 + k_2{}^2}{k_1{}^2.k_2{}^2.k_1{}^2.(\,k_1 - p\,)^{22}.(\,-k_1 + k_2 + p\,)^2} \right)$$

$$\tilde{\Pi}^{\mu\beta}_{89}(p,k_1,k_2) = i\,\mathrm{e}^4\,Q_1\left(2\,k_1{}^{\beta}-p^{\beta}\right)(2\,k_1{}^{\mu}-p^{\mu})\,(k_1\cdot u)$$
$$\left(\frac{(\xi-1)\left(k_1{}^2-k_2{}^2\right)^2}{\left(k_1{}^2\right)^2.k_2{}^2.k_1{}^2.(\,k_1-p\,)^2.(\,k_1+k_2\,)^{22}}+\frac{-2\,(k_1\cdot k_2)+k_1{}^2+k_2{}^2}{\left(k_1{}^2\right)^2.k_2{}^2.k_1{}^2.(\,k_1-p\,)^2.(\,k_1+k_2\,)^2}\right)$$
$$\tilde{\Pi}^{\mu\beta}_{90}(p,k_1,k_2) = -i\,\mathrm{e}^4\,Q_1\,(b\cdot k_1)\left(2\,k_1{}^{\beta}-p^{\beta}\right)(2\,k_1{}^{\mu}-p^{\mu})$$
$$\left(\frac{(\xi-1)\left(k_1{}^2-k_2{}^2\right)^2}{\left(k_1{}^2\right)^2.k_2{}^2.k_1{}^2.(\,k_1-p\,)^2.(\,k_1+k_2\,)^{22}}+\frac{-2\,(k_1\cdot k_2)+k_1{}^2+k_2{}^2}{\left(k_1{}^2\right)^2.k_2{}^2.k_1{}^2.(\,k_1-p\,)^2.(\,k_1+k_2\,)^2}\right)$$
$$\tilde{\Pi}^{\mu\beta}_{91}(p,k_1,k_2) = -i\,\mathrm{e}^4\,Q_1\left(2\,k_1{}^{\beta}-p^{\beta}\right)(2\,k_1{}^{\mu}-p^{\mu})\,(k_1\cdot u-p\cdot u)$$
$$\left(\frac{(\xi-1)\left(-2\,(k_1\cdot p)+p^2+k_1{}^2-k_2{}^2\right)^2}{k_2{}^2.k_1{}^2.(\,k_1-p\,)^{23}.(\,-k_1+k_2+p\,)^{22}}+\frac{-2\,(k_1\cdot p)-2\,(k_2\cdot p)+p^2+2\,(k_1\cdot k_2)+k_1{}^2+k_2{}^2}{k_2{}^2.k_1{}^2.(\,k_1-p\,)^{23}.(\,-k_1+k_2+p\,)^2}\right)$$
$$\tilde{\Pi}^{\mu\beta}_{92}(p,k_1,k_2) = i\,\mathrm{e}^4\,Q_1\left(2\,k_1{}^{\beta}-p^{\beta}\right)(2\,k_1{}^{\mu}-p^{\mu})\,(k_1\cdot u-p\cdot u)$$
$$\left(\frac{(\xi-1)\left(-2\,(k_1\cdot p)+p^2+k_1{}^2-k_2{}^2\right)^2}{k_2{}^2.k_1{}^2.(\,k_1-p\,)^{23}.(\,-k_1+k_2+p\,)^{22}}+\frac{-2\,(k_1\cdot p)-2\,(k_2\cdot p)+p^2+2\,(k_1\cdot k_2)+k_1{}^2+k_2{}^2}{k_2{}^2.k_1{}^2.(\,k_1-p\,)^{23}.(\,-k_1+k_2+p\,)^2}\right)$$
$$\tilde{\Pi}^{\mu\beta}_{93}(p,k_1,k_2) = \frac{i\,\mathrm{e}^2\,\lambda\,Q_1\,u^{\beta}\,(2\,k_1{}^{\mu}-p^{\mu})}{k_2{}^2.k_1{}^2.(\,k_2+p\,)^2.(\,k_1-p\,)^2}$$
$$\tilde{\Pi}^{\mu\beta}_{94}(p,k_1,k_2) = \frac{2\,i\,\mathrm{e}^2\,\lambda\,Q_1\,g^{\mu\,\beta}\,(k_1\cdot u)}{\left(k_2{}^2\right)^2.\left(k_1{}^2\right)^2}$$
$$\tilde{\Pi}^{\mu\beta}_{95}(p,k_1,k_2) = 0$$
$$\tilde{\Pi}^{\mu\beta}_{96}(p,k_1,k_2) = \frac{i\,\mathrm{e}^2\,\lambda\,Q_1\,u^{\mu}\left(p^{\beta}+2\,k_1{}^{\beta}\right)}{k_2{}^2.k_1{}^2.(\,k_2-p\,)^2.(\,k_1+p\,)^2}$$

where $\epsilon^{\alpha\beta\sigma \mathrm{k}_1}$ stands for a contraction of the Levi−Civita tensor
with a momentum $k_1$ as $\epsilon^{\alpha\beta\sigma \mathrm{k}_1}=\epsilon^{\alpha\beta\sigma\delta}\,k_{1\delta}$ and $D$ is the dimension of the spacetime.

We simplify the integrals into a set of fundamental ones
by employing the TARCER Mathematica package. Our results are as follows :

$$(4\,\pi)^D\,\Pi^{\mu\beta}_1(p,k_1,k_2) = \frac{1}{3\,(D-6)\,p^4}\,i\,\mathrm{e}^4\,Q_1\,\mathbf{J}^{(D)}_{\{1,0\}\,\{1,0\}\,\{1,0\}}$$
$$\left(p^{\mu}\left(-2\left(D^2-7\,D+12\right)(D\,(\xi-1)-5\,\xi+2)\,p^{\beta}\,(p\cdot u)-(D-6)\,p^2\,(D\,(\xi-1)-2\,\xi+5)\,u^{\beta}\right)+\right.$$
$$\left.2\,(D-3)\,p^2\,(D\,(\xi-1)-5\,\xi+2)\,g^{\mu\,\beta}\,(p\cdot u)+2\,(D-3)\,p^2\,(D\,(\xi-1)-5\,\xi+2)\,p^{\beta}\,u^{\mu}\right)$$
$$(4\,\pi)^D\,\Pi^{\mu\beta}_2(p,k_1,k_2) = \frac{1}{3\,(D-6)\,p^4}\,i\,\mathrm{e}^4\,Q_1\,\mathbf{J}^{(D)}_{\{1,0\}\,\{1,0\}\,\{1,0\}}$$
$$\left(p^{\mu}\left(2\left(D^2-7\,D+12\right)(D\,(\xi-1)-5\,\xi+2)\,p^{\beta}\,(p\cdot u)+(D-6)\,p^2\,(D\,(\xi-1)-2\,\xi+5)\,u^{\beta}\right)-\right.$$
$$\left.2\,(D-3)\,p^2\,(D\,(\xi-1)-5\,\xi+2)\,g^{\mu\,\beta}\,(p\cdot u)-2\,(D-3)\,p^2\,(D\,(\xi-1)-5\,\xi+2)\,p^{\beta}\,u^{\mu}\right)$$
$$(4\,\pi)^D\,\Pi^{\mu\beta}_3(p,k_1,k_2) = 0$$
$$(4\,\pi)^D\,\Pi^{\mu\beta}_4(p,k_1,k_2) = 0$$
$$(4\,\pi)^D\,\Pi^{\mu\beta}_5(p,k_1,k_2) = \frac{1}{3\,(D-6)\,(D-4)^2\,(D-1)\,p^4}\,2\,i\,\mathrm{e}^4\,Q_1$$
$$\left(p^2\left(g^{\mu\,\beta}\,(p\cdot u)\left(-3\left(D^2-10\,D+24\right)p^2\left(\mathbf{B}^{(D)}_{\{1,0\}\,\{1,0\}}\right)^2-2\,(D-3)\left(D^3\,(\xi-1)+D^2\,(6-9\,\xi)+6\,D\,(4\,\xi-1)-16\,(\xi-1)\right)\right.\right.\right.$$
$$\left.\left.\mathbf{J}^{(D)}_{\{1,0\}\,\{1,0\}\,\{1,0\}}\right)+\left(D^2-4\,D+3\right)(D-4)^2\,(\xi-1)\,p^{\beta}\,u^{\mu}\,\mathbf{J}^{(D)}_{\{1,0\}\,\{1,0\}\,\{1,0\}}\right)+$$
$$p^{\mu}\left((D-6)\,p^{\beta}\,(p\cdot u)\left(3\,(D-4)\,p^2\left(\mathbf{B}^{(D)}_{\{1,0\}\,\{1,0\}}\right)^2+\left(D^4\,(-(\xi-1))+D^3\,(13\,\xi-10)+D^2\,(27-60\,\xi)+\right.\right.\right.$$
$$\left.\left.\left.\left.2\,D\,(56\,\xi-11)-64\,\xi+16\right)\mathbf{J}^{(D)}_{\{1,0\}\,\{1,0\}\,\{1,0\}}\right)+\left(D^2-4\,D+3\right)(D-4)^2\,(\xi-1)\,p^2\,u^{\beta}\,\mathbf{J}^{(D)}_{\{1,0\}\,\{1,0\}\,\{1,0\}}\right)\right)$$
$$(4\,\pi)^D\,\Pi^{\mu\beta}_6(p,k_1,k_2) = \frac{1}{3\,(D-6)\,(D-4)^2\,(D-1)\,p^4}$$

2

$i$

$\mathrm{e}^4$

$Q_1$

$$\Big(p^2 \Big(g^{\mu\beta} (p\cdot u) \Big(3 \left(D^2 - 10 D + 24\right) p^2 \left(\mathbf{B}^{(D)}_{\{1,0\}\{1,0\}}\right)^2 + 2 (D-3) \left(D^3 (\xi - 1) + D^2 (6 - 9\xi) + 6 D (4\xi - 1) - 16 (\xi - 1)\right) \mathbf{J}^{(D)}_{\{1,0\}\{1,0\}\{1,0\}}\Big) - (D-4)^2 \left(D^2 - 4D + 3\right) (\xi - 1) p^\beta u^\mu \mathbf{J}^{(D)}_{\{1,0\}\{1,0\}\{1,0\}}\Big) + p^\mu \Big((D-6) p^\beta (p\cdot u) \Big(\left(D^4 (\xi - 1) + D^3 (10 - 13\xi) + 3 D^2 (20\xi - 9) + D (22 - 112\xi) + 64\xi - 16\right) \mathbf{J}^{(D)}_{\{1,0\}\{1,0\}\{1,0\}} - 3 (D-4) p^2 \left(\mathbf{B}^{(D)}_{\{1,0\}\{1,0\}}\right)^2\Big) - (D-4)^2 \left(D^2 - 4D + 3\right) (\xi - 1) p^2 u^\beta \mathbf{J}^{(D)}_{\{1,0\}\{1,0\}\{1,0\}}\Big)\Big)$$

$$(4\pi)^D \Pi^{\mu\beta}_7(p, k_1, k_2) = -\frac{1}{3(D-6) p^4} i\, e^4 Q_1 \mathbf{J}^{(D)}_{\{1,0\}\{1,0\}\{1,0\}} \Big((D-6) p^2 (D(\xi - 1) - 2\xi + 5) p^\beta u^\mu - 2 (D-3) (D(\xi - 1) - 5\xi + 2) \left(p^\mu \left(p^2 u^\beta - (D-4) p^\beta (p\cdot u)\right) + p^2 g^{\mu\beta} (p\cdot u)\right)\Big)$$

$$(4\pi)^D \Pi^{\mu\beta}_8(p, k_1, k_2) = \frac{1}{3(D-6) p^4} i\, e^4 Q_1 \mathbf{J}^{(D)}_{\{1,0\}\{1,0\}\{1,0\}} \Big((D-6) p^2 (D(\xi - 1) - 2\xi + 5) p^\beta u^\mu - 2 (D-3) (D(\xi - 1) - 5\xi + 2) \left(p^\mu \left(p^2 u^\beta - (D-4) p^\beta (p\cdot u)\right) + p^2 g^{\mu\beta} (p\cdot u)\right)\Big)$$

$$(4\pi)^D \Pi^{\mu\beta}_9(p, k_1, k_2) = 0$$

$$(4\pi)^D \Pi^{\mu\beta}_{10}(p, k_1, k_2) = 0$$

$$(4\pi)^D \Pi^{\mu\beta}_{11}(p, k_1, k_2) = \frac{1}{3(D-6)(D-4)^2 (D-1) p^4} i\, e^4 Q_1 \Big(p^2 g^{\mu\beta} (p\cdot u) \Big(3 \left(-2 D^3 + 27 D^2 - 118 D + 168\right) p^2 \left(\mathbf{B}^{(D)}_{\{1,0\}\{1,0\}}\right)^2 - 2 (D-3) \left(D^4 (\xi - 1) - 2 D^3 (7\xi - 5) + 5 D^2 (13\xi - 6) - 58 D (2\xi - 1) + 16 (4\xi - 7)\right) \mathbf{J}^{(D)}_{\{1,0\}\{1,0\}\{1,0\}}\Big) + p^2 p^\beta u^\mu \Big(6 \left(D^2 - 10 D + 24\right) p^2 \left(\mathbf{B}^{(D)}_{\{1,0\}\{1,0\}}\right)^2 + (D-3) \left(D^4 (\xi - 1) + D^3 (7 - 11\xi) + 2 D^2 (19\xi - 9) + D (40 - 44\xi) + 16 (\xi + 2)\right) \mathbf{J}^{(D)}_{\{1,0\}\{1,0\}\{1,0\}}\Big) + p^\mu \Big((D-6) p^\beta (p\cdot u) \Big(3 \left(2 D^2 - 17 D + 36\right) p^2 \left(\mathbf{B}^{(D)}_{\{1,0\}\{1,0\}}\right)^2 + \big(D^5 (-(\xi - 1)) + D^4 (21\xi - 17) + D^3 (97 - 160\xi) + D^2 (556\xi - 235) + D (278 - 864\xi) + 448\xi - 208\big) \mathbf{J}^{(D)}_{\{1,0\}\{1,0\}\{1,0\}}\Big) - 2 \left(D^3 - 8 D^2 + 19 D - 12\right) p^2 \left(D^2 (\xi - 1) + D (5 - 9\xi) + 22\xi - 4\right) u^\beta \mathbf{J}^{(D)}_{\{1,0\}\{1,0\}\{1,0\}}\Big)\Big)$$

$$(4\pi)^D \Pi^{\mu\beta}_{12}(p, k_1, k_2) = \frac{1}{3(D-6)(D-4)^2 (D-1) p^4} i\, e^4 Q_1 \Big(p^2 g^{\mu\beta} (p\cdot u) \Big(3 \left(2 D^3 - 27 D^2 + 118 D - 168\right) p^2 \left(\mathbf{B}^{(D)}_{\{1,0\}\{1,0\}}\right)^2 + 2 (D-3) \left(D^4 (\xi - 1) - 2 D^3 (7\xi - 5) + 5 D^2 (13\xi - 6) - 58 D (2\xi - 1) + 16 (4\xi - 7)\right) \mathbf{J}^{(D)}_{\{1,0\}\{1,0\}\{1,0\}}\Big) + p^2 p^\beta u^\mu \Big(-6 \left(D^2 - 10 D + 24\right) p^2 \left(\mathbf{B}^{(D)}_{\{1,0\}\{1,0\}}\right)^2 - (D-3) \left(D^4 (\xi - 1) + D^3 (7 - 11\xi) + 2 D^2 (19\xi - 9) + D (40 - 44\xi) + 16 (\xi + 2)\right) \mathbf{J}^{(D)}_{\{1,0\}\{1,0\}\{1,0\}}\Big) + p^\mu \Big((D-6) p^\beta (p\cdot u) \Big(\left(D^5 (\xi - 1) + D^4 (17 - 21\xi) + D^3 (160\xi - 97) + D^2 (235 - 556\xi) + D (864\xi - 278) - 448\xi + 208\right) \mathbf{J}^{(D)}_{\{1,0\}\{1,0\}\{1,0\}} - 3 \left(2 D^2 - 17 D + 36\right) p^2 \left(\mathbf{B}^{(D)}_{\{1,0\}\{1,0\}}\right)^2\Big) + 2 \left(D^3 - 8 D^2 + 19 D - 12\right) p^2 \left(D^2 (\xi - 1) + D (5 - 9\xi) + 22\xi - 4\right) u^\beta \mathbf{J}^{(D)}_{\{1,0\}\{1,0\}\{1,0\}}\Big)\Big)$$

$$(4\pi)^D \Pi^{\mu\beta}_{13}(p, k_1, k_2) = \frac{1}{3(D-6)(D-4)^2 (D-1) p^4} i\, e^4 Q_1 \Big(p^2 \Big(g^{\mu\beta} (p\cdot u) \Big(3 \left(2 D^3 - 27 D^2 + 118 D - 168\right) p^2 \left(\mathbf{B}^{(D)}_{\{1,0\}\{1,0\}}\right)^2 + 2 (D-3) \left(D^4 (\xi - 1) - 2 D^3 (7\xi - 5) + 5 D^2 (13\xi - 6) - 58 D (2\xi - 1) + 16 (4\xi - 7)\right) \mathbf{J}^{(D)}_{\{1,0\}\{1,0\}\{1,0\}}\Big) + 2 \left(D^3 - 8 D^2 + 19 D - 12\right) \left(D^2 (\xi - 1) + D (5 - 9\xi) + 22\xi - 4\right) p^\beta u^\mu \mathbf{J}^{(D)}_{\{1,0\}\{1,0\}\{1,0\}}\Big) + p^\mu \Big(p^2 u^\beta \Big(-6 \left(D^2 - 10 D + 24\right) p^2 \left(\mathbf{B}^{(D)}_{\{1,0\}\{1,0\}}\right)^2 - (D-3) \left(D^4 (\xi - 1) + D^3 (7 - 11\xi) + 2 D^2 (19\xi - 9) + D (40 - 44\xi) + 16 (\xi + 2)\right) \mathbf{J}^{(D)}_{\{1,0\}\{1,0\}\{1,0\}}\Big) + (D-6) p^\beta (p\cdot u) \Big(\left(D^5 (\xi - 1) + D^4 (17 - 21\xi) + D^3 (160\xi - 97) + D^2 (235 - 556\xi) + D (864\xi - 278) - 448\xi + 208\right) \mathbf{J}^{(D)}_{\{1,0\}\{1,0\}\{1,0\}} - 3 \left(2 D^2 - 17 D + 36\right) p^2 \left(\mathbf{B}^{(D)}_{\{1,0\}\{1,0\}}\right)^2\Big)\Big)\Big)$$

$$(4\pi)^D \Pi^{\mu\beta}_{14}(p, k_1, k_2) = \frac{1}{3(D-6)(D-4)^2 (D-1) p^4}$$

$i$

$e^4$

$Q_1$

$$\Big(p^2 \Big(g^{\mu\beta}(p\cdot u)\Big(3\left(-2D^3+27D^2-118D+168\right)p^2\left(\mathbf{B}^{(D)}_{\{1,0\}\{1,0\}}\right)^2-2(D-3)$$
$$\left(D^4(\xi-1)-2D^3(7\xi-5)+5D^2(13\xi-6)-58D(2\xi-1)+16(4\xi-7)\right)\mathbf{J}^{(D)}_{\{1,0\}\{1,0\}\{1,0\}}\Big)-$$
$$2\left(D^3-8D^2+19D-12\right)\left(D^2(\xi-1)+D(5-9\xi)+22\xi-4\right)p^\beta u^\mu \mathbf{J}^{(D)}_{\{1,0\}\{1,0\}\{1,0\}}\Big)+$$
$$p^\mu\Big(p^2 u^\beta\Big(6\left(D^2-10D+24\right)p^2\left(\mathbf{B}^{(D)}_{\{1,0\}\{1,0\}}\right)^2+(D-3)\left(D^4(\xi-1)+D^3(7-11\xi)+2D^2(19\xi-9)+D(40-44\xi)+\right.$$
$$\left.16(\xi+2)\right)\mathbf{J}^{(D)}_{\{1,0\}\{1,0\}\{1,0\}}\Big)+(D-6)p^\beta(p\cdot u)\Big(3\left(2D^2-17D+36\right)p^2\left(\mathbf{B}^{(D)}_{\{1,0\}\{1,0\}}\right)^2+\left(D^5(-(\xi-1))+\right.$$
$$\left.D^4(21\xi-17)+D^3(97-160\xi)+D^2(556\xi-235)+D(278-864\xi)+448\xi-208\right)\mathbf{J}^{(D)}_{\{1,0\}\{1,0\}\{1,0\}}\Big)\Big)\Big)$$

$$(4\pi)^D\,\Pi^{\mu\beta}_{15}(p,k_1,k_2)=\frac{1}{3(D-6)(D-4)p^4} i\,e^4 Q_1\left(D^2(\xi-1)+D(5-7\xi)+14\xi-4\right)\mathbf{J}^{(D)}_{\{1,0\}\{1,0\}\{1,0\}}$$
$$\left(4(D-3)p^2 g^{\mu\beta}(p\cdot u)+(D-6)p^2p^\beta u^\mu+p^\mu\left((D-6)p^2u^\beta-(D-4)D\,p^\beta(p\cdot u)\right)\right)$$

$$(4\pi)^D\,\Pi^{\mu\beta}_{16}(p,k_1,k_2)=\frac{1}{3(D-6)(D-4)p^4} i\,e^4 Q_1\left(D^2(\xi-1)+D(5-7\xi)+14\xi-4\right)\mathbf{J}^{(D)}_{\{1,0\}\{1,0\}\{1,0\}}$$
$$\left(-4(D-3)p^2 g^{\mu\beta}(p\cdot u)-(D-6)p^2p^\beta u^\mu+p^\mu\left((D-4)D\,p^\beta(p\cdot u)-(D-6)p^2u^\beta\right)\right)$$

$$(4\pi)^D\,\Pi^{\mu\beta}_{17}(p,k_1,k_2)=0$$
$$(4\pi)^D\,\Pi^{\mu\beta}_{18}(p,k_1,k_2)=0$$

$$(4\pi)^D\,\Pi^{\mu\beta}_{19}(p,k_1,k_2)=\frac{1}{3(D-6)p^4}2\,i\,e^4 Q_1\,\mathbf{J}^{(D)}_{\{1,0\}\{1,0\}\{1,0\}}$$
$$\left(p^\mu\left((D-6)(\xi+2)p^2u^\beta-\left(D^2-7D+12\right)(\xi-1)p^\beta(p\cdot u)\right)+(D-3)(\xi-1)p^2g^{\mu\beta}(p\cdot u)+(D-3)(\xi-1)p^2p^\beta u^\mu\right)$$

$$(4\pi)^D\,\Pi^{\mu\beta}_{20}(p,k_1,k_2)=-\frac{1}{3(D-6)p^4}2\,i\,e^4 Q_1\,\mathbf{J}^{(D)}_{\{1,0\}\{1,0\}\{1,0\}}$$
$$\left(p^\mu\left((D-6)(\xi+2)p^2u^\beta-\left(D^2-7D+12\right)(\xi-1)p^\beta(p\cdot u)\right)+(D-3)(\xi-1)p^2g^{\mu\beta}(p\cdot u)+(D-3)(\xi-1)p^2p^\beta u^\mu\right)$$

$$(4\pi)^D\,\Pi^{\mu\beta}_{21}(p,k_1,k_2)=0$$
$$(4\pi)^D\,\Pi^{\mu\beta}_{22}(p,k_1,k_2)=0$$
$$(4\pi)^D\,\Pi^{\mu\beta}_{23}(p,k_1,k_2)=0$$
$$(4\pi)^D\,\Pi^{\mu\beta}_{24}(p,k_1,k_2)=0$$

$$(4\pi)^D\,\Pi^{\mu\beta}_{25}(p,k_1,k_2)=$$
$$-\frac{2\,i(D-3)e^4Q_1\mathbf{J}^{(D)}_{\{1,0\}\{1,0\}\{1,0\}}\left((\xi-1)p^\mu\left(2(D-4)p^\beta(p\cdot u)+p^2u^\beta\right)-2(\xi+2)p^2g^{\mu\beta}(p\cdot u)+(\xi-1)p^2p^\beta u^\mu\right)}{3p^4}$$

$$(4\pi)^D\,\Pi^{\mu\beta}_{26}(p,k_1,k_2)=$$
$$\frac{2\,i(D-3)e^4Q_1\mathbf{J}^{(D)}_{\{1,0\}\{1,0\}\{1,0\}}\left((\xi-1)p^\mu\left(2(D-4)p^\beta(p\cdot u)+p^2u^\beta\right)-2(\xi+2)p^2g^{\mu\beta}(p\cdot u)+(\xi-1)p^2p^\beta u^\mu\right)}{3p^4}$$

$$(4\pi)^D\,\Pi^{\mu\beta}_{27}(p,k_1,k_2)=-\frac{8(D-3)e^4Q_2\,\epsilon^{\beta\mu b p}\,\mathbf{J}^{(D)}_{\{1,0\}\{1,0\}\{1,0\}}}{p^2}$$

$$(4\pi)^D\,\Pi^{\mu\beta}_{28}(p,k_1,k_2)=$$
$$\frac{2\,i\,e^4Q_1\mathbf{J}^{(D)}_{\{1,0\}\{1,0\}\{1,0\}}\left((D-3)(\xi-1)\left(p^\mu\left(p^2u^\beta-(D-4)p^\beta(p\cdot u)\right)+p^2g^{\mu\beta}(p\cdot u)\right)+(D-6)(\xi+2)p^2p^\beta u^\mu\right)}{3(D-6)p^4}$$

$$(4\pi)^D\,\Pi^{\mu\beta}_{29}(p,k_1,k_2)=$$
$$-\frac{2\,i\,e^4Q_1\mathbf{J}^{(D)}_{\{1,0\}\{1,0\}\{1,0\}}\left((D-3)(\xi-1)\left(p^\mu\left(p^2u^\beta-(D-4)p^\beta(p\cdot u)\right)+p^2g^{\mu\beta}(p\cdot u)\right)+(D-6)(\xi+2)p^2p^\beta u^\mu\right)}{3(D-6)p^4}$$

$$(4\pi)^D\,\Pi^{\mu\beta}_{30}(p,k_1,k_2)=-\frac{2\,i(D-3)e^4Q_1\left(D(\xi-1)-4\xi+1\right)p^\mu u^\beta\,\mathbf{J}^{(D)}_{\{1,0\}\{1,0\}\{1,0\}}}{(D-4)p^2}$$

$$(4\pi)^D\,\Pi^{\mu\beta}_{31}(p,k_1,k_2)=\frac{2\,i(D-3)e^4Q_1\left(D(\xi-1)-4\xi+1\right)p^\mu u^\beta\,\mathbf{J}^{(D)}_{\{1,0\}\{1,0\}\{1,0\}}}{(D-4)p^2}$$

$$(4\pi)^D\,\Pi^{\mu\beta}_{32}(p,k_1,k_2)=0$$
$$(4\pi)^D\,\Pi^{\mu\beta}_{33}(p,k_1,k_2)=0$$

$$(4\pi)^D\,\Pi^{\mu\beta}_{34}(p,k_1,k_2)=0$$
$$(4\pi)^D\,\Pi^{\mu\beta}_{35}(p,k_1,k_2)=0$$
$$(4\pi)^D\,\Pi^{\mu\beta}_{36}(p,k_1,k_2)=0$$
$$(4\pi)^D\,\Pi^{\mu\beta}_{37}(p,k_1,k_2)=0$$
$$(4\pi)^D\,\Pi^{\mu\beta}_{38}(p,k_1,k_2)=0$$
$$(4\pi)^D\,\Pi^{\mu\beta}_{39}(p,k_1,k_2)=0$$
$$(4\pi)^D\,\Pi^{\mu\beta}_{40}(p,k_1,k_2)=0$$
$$(4\pi)^D\,\Pi^{\mu\beta}_{41}(p,k_1,k_2)=0$$
$$(4\pi)^D\,\Pi^{\mu\beta}_{42}(p,k_1,k_2)=\frac{2\,i\,(D-3)\,e^4\,Q_1\,(D\,(\xi-1)-4\,\xi+1)\,p^\beta\,u^\mu\,\mathbf{J}^{(D)}_{\{1,0\}\,\{1,0\}\,\{1,0\}}}{(D-4)\,p^2}$$
$$(4\pi)^D\,\Pi^{\mu\beta}_{43}(p,k_1,k_2)=-\frac{2\,i\,(D-3)\,e^4\,Q_1\,(D\,(\xi-1)-4\,\xi+1)\,p^\beta\,u^\mu\,\mathbf{J}^{(D)}_{\{1,0\}\,\{1,0\}\,\{1,0\}}}{(D-4)\,p^2}$$
$$(4\pi)^D\,\Pi^{\mu\beta}_{44}(p,k_1,k_2)=0$$
$$(4\pi)^D\,\Pi^{\mu\beta}_{45}(p,k_1,k_2)=0$$
$$(4\pi)^D\,\Pi^{\mu\beta}_{46}(p,k_1,k_2)=0$$
$$(4\pi)^D\,\Pi^{\mu\beta}_{47}(p,k_1,k_2)=0$$
$$(4\pi)^D\,\Pi^{\mu\beta}_{48}(p,k_1,k_2)=0$$
$$(4\pi)^D\,\Pi^{\mu\beta}_{49}(p,k_1,k_2)=0$$
$$(4\pi)^D\,\Pi^{\mu\beta}_{50}(p,k_1,k_2)=0$$
$$(4\pi)^D\,\Pi^{\mu\beta}_{51}(p,k_1,k_2)=0$$
$$(4\pi)^D\,\Pi^{\mu\beta}_{52}(p,k_1,k_2)=0$$
$$(4\pi)^D\,\Pi^{\mu\beta}_{53}(p,k_1,k_2)=0$$
$$(4\pi)^D\,\Pi^{\mu\beta}_{54}(p,k_1,k_2)=0$$
$$(4\pi)^D\,\Pi^{\mu\beta}_{55}(p,k_1,k_2)=0$$
$$(4\pi)^D\,\Pi^{\mu\beta}_{56}(p,k_1,k_2)=0$$
$$(4\pi)^D\,\Pi^{\mu\beta}_{57}(p,k_1,k_2)=0$$
$$(4\pi)^D\,\Pi^{\mu\beta}_{58}(p,k_1,k_2)=0$$
$$(4\pi)^D\,\Pi^{\mu\beta}_{59}(p,k_1,k_2)=0$$
$$(4\pi)^D\,\Pi^{\mu\beta}_{60}(p,k_1,k_2)=0$$
$$(4\pi)^D\,\Pi^{\mu\beta}_{61}(p,k_1,k_2)=0$$
$$(4\pi)^D\,\Pi^{\mu\beta}_{62}(p,k_1,k_2)=0$$
$$(4\pi)^D\,\Pi^{\mu\beta}_{63}(p,k_1,k_2)=0$$
$$(4\pi)^D\,\Pi^{\mu\beta}_{64}(p,k_1,k_2)=$$
$$\frac{i\,(D-3)\,e^4\,Q_1\,(D\,(\xi-1)-4\,\xi+1)\,\mathbf{J}^{(D)}_{\{1,0\}\,\{1,0\}\,\{1,0\}}\left(p^\mu\left(2\,(D-4)\,p^\beta\,(p\cdot u)+p^2\,u^\beta\right)-2\,p^2\,g^{\mu\,\beta}\,(p\cdot u)+4\,p^2\,p^\beta\,u^\mu\right)}{3\,(D-4)\,p^4}$$
$$(4\pi)^D\,\Pi^{\mu\beta}_{65}(p,k_1,k_2)=$$
$$-\frac{i\,(D-3)\,e^4\,Q_1\,(D\,(\xi-1)-4\,\xi+1)\,\mathbf{J}^{(D)}_{\{1,0\}\,\{1,0\}\,\{1,0\}}\left(p^\mu\left(2\,(D-4)\,p^\beta\,(p\cdot u)+p^2\,u^\beta\right)-2\,p^2\,g^{\mu\,\beta}\,(p\cdot u)+4\,p^2\,p^\beta\,u^\mu\right)}{3\,(D-4)\,p^4}$$
$$(4\pi)^D\,\Pi^{\mu\beta}_{66}(p,k_1,k_2)=\frac{1}{3\,(D-6)\,(D-4)\,p^4}i\,e^4\,Q_1\,(D\,(\xi-1)-4\,\xi+1)\,\mathbf{J}^{(D)}_{\{1,0\}\,\{1,0\}\,\{1,0\}}$$
$$\left(p^\mu\left(4\left(D^2-7\,D+12\right)p^\beta\,(p\cdot u)-(D-6)\,p^2\,u^\beta\right)-4\,(D-3)\,p^2\,g^{\mu\,\beta}\,(p\cdot u)-4\,(D-3)\,p^2\,p^\beta\,u^\mu\right)$$
$$(4\pi)^D\,\Pi^{\mu\beta}_{67}(p,k_1,k_2)=\frac{1}{3\,(D-6)\,(D-4)\,p^4}i\,e^4\,Q_1\,(D\,(\xi-1)-4\,\xi+1)\,\mathbf{J}^{(D)}_{\{1,0\}\,\{1,0\}\,\{1,0\}}$$
$$\left(p^\mu\left((D-6)\,p^2\,u^\beta-4\left(D^2-7\,D+12\right)p^\beta\,(p\cdot u)\right)+4\,(D-3)\,p^2\,g^{\mu\,\beta}\,(p\cdot u)+4\,(D-3)\,p^2\,p^\beta\,u^\mu\right)$$
$$(4\pi)^D\,\Pi^{\mu\beta}_{68}(p,k_1,k_2)=$$

$$\frac{i\,e^4\,Q_1\,(D\,(\xi-1)-4\,\xi+1)\,\mathbf{J}^{(D)}_{\{1,0\}\,\{1,0\}\,\{1,0\}}\left(-4\,(D-3)\,p^2\,g^{\mu\,\beta}\,(p\cdot u)-(D-6)\,p^2\,p^\beta\,u^\mu+p^\mu\left((D-4)\,D\,p^\beta\,(p\cdot u)-(D-6)\,p^2\,u^\beta\right)\right)}{3\,(D-6)\,(D-4)\,p^4}$$

$$(4\,\pi)^D\,\Pi^{\mu\beta}_{69}(p,\,k_1,\,k_2)=\frac{i\,e^4\,Q_1\,(D\,(\xi-1)-4\,\xi+1)\,\mathbf{J}^{(D)}_{\{1,0\}\,\{1,0\}\,\{1,0\}}\left(4\,(D-3)\,p^2\,g^{\mu\,\beta}\,(p\cdot u)+(D-6)\,p^2\,p^\beta\,u^\mu+p^\mu\left((D-6)\,p^2\,u^\beta-(D-4)\,D\,p^\beta\,(p\cdot u)\right)\right)}{3\,(D-6)\,(D-4)\,p^4}$$

$$(4\,\pi)^D\,\Pi^{\mu\beta}_{70}(p,\,k_1,\,k_2)=\frac{i\,e^4\,Q_1\,(D\,(\xi-1)-4\,\xi+1)\,\mathbf{J}^{(D)}_{\{1,0\}\,\{1,0\}\,\{1,0\}}\left(4\,(D-3)\,p^2\,g^{\mu\,\beta}\,(p\cdot u)+(D-6)\,p^2\,p^\beta\,u^\mu+p^\mu\left((D-6)\,p^2\,u^\beta-(D-4)\,D\,p^\beta\,(p\cdot u)\right)\right)}{3\,(D-6)\,(D-4)\,p^4}$$

$$(4\,\pi)^D\,\Pi^{\mu\beta}_{71}(p,\,k_1,\,k_2)=\frac{i\,e^4\,Q_1\,(D\,(\xi-1)-4\,\xi+1)\,\mathbf{J}^{(D)}_{\{1,0\}\,\{1,0\}\,\{1,0\}}\left(-4\,(D-3)\,p^2\,g^{\mu\,\beta}\,(p\cdot u)-(D-6)\,p^2\,p^\beta\,u^\mu+p^\mu\left((D-4)\,D\,p^\beta\,(p\cdot u)-(D-6)\,p^2\,u^\beta\right)\right)}{3\,(D-6)\,(D-4)\,p^4}$$

$$(4\,\pi)^D\,\Pi^{\mu\beta}_{72}(p,\,k_1,\,k_2)=\frac{i\,e^4\,Q_1\,(D\,(\xi-1)-3\,\xi+1)\,p^\mu\,u^\beta\,\mathbf{J}^{(D)}_{\{1,0\}\,\{1,0\}\,\{1,0\}}}{p^2}$$

$$(4\,\pi)^D\,\Pi^{\mu\beta}_{73}(p,\,k_1,\,k_2)=-\frac{i\,e^4\,Q_1\,(D\,(\xi-1)-3\,\xi+1)\,p^\mu\,u^\beta\,\mathbf{J}^{(D)}_{\{1,0\}\,\{1,0\}\,\{1,0\}}}{p^2}$$

$$(4\,\pi)^D\,\Pi^{\mu\beta}_{74}(p,\,k_1,\,k_2)=0$$

$$(4\,\pi)^D\,\Pi^{\mu\beta}_{75}(p,\,k_1,\,k_2)=\frac{i\,e^4\,Q_1\,(D\,(\xi-1)-4\,\xi+1)\,\mathbf{J}^{(D)}_{\{1,0\}\,\{1,0\}\,\{1,0\}}\left(4\,(D-3)\left(p^\mu\left(p^2\,u^\beta-(D-4)\,p^\beta\,(p\cdot u)\right)+p^2\,g^{\mu\,\beta}\,(p\cdot u)\right)+(D-6)\,p^2\,p^\beta\,u^\mu\right)}{3\,(D-6)\,(D-4)\,p^4}$$

$$(4\,\pi)^D\,\Pi^{\mu\beta}_{76}(p,\,k_1,\,k_2)=\frac{i\,e^4\,Q_1\,(D\,(\xi-1)-4\,\xi+1)\,\mathbf{J}^{(D)}_{\{1,0\}\,\{1,0\}\,\{1,0\}}\left(-4\,(D-3)\left(p^\mu\left(p^2\,u^\beta-(D-4)\,p^\beta\,(p\cdot u)\right)+p^2\,g^{\mu\,\beta}\,(p\cdot u)\right)-(D-6)\,p^2\,p^\beta\,u^\mu\right)}{3\,(D-6)\,(D-4)\,p^4}$$

$$(4\,\pi)^D\,\Pi^{\mu\beta}_{77}(p,\,k_1,\,k_2)=-\frac{i\,(D-3)\,e^4\,Q_1\,(D\,(\xi-1)-4\,\xi+1)\,\mathbf{J}^{(D)}_{\{1,0\}\,\{1,0\}\,\{1,0\}}\left(2\,p^\mu\left((D-4)\,p^\beta\,(p\cdot u)+2\,p^2\,u^\beta\right)-2\,p^2\,g^{\mu\,\beta}\,(p\cdot u)+p^2\,p^\beta\,u^\mu\right)}{3\,(D-4)\,p^4}$$

$$(4\,\pi)^D\,\Pi^{\mu\beta}_{78}(p,\,k_1,\,k_2)=\frac{i\,(D-3)\,e^4\,Q_1\,(D\,(\xi-1)-4\,\xi+1)\,\mathbf{J}^{(D)}_{\{1,0\}\,\{1,0\}\,\{1,0\}}\left(2\,p^\mu\left((D-4)\,p^\beta\,(p\cdot u)+2\,p^2\,u^\beta\right)-2\,p^2\,g^{\mu\,\beta}\,(p\cdot u)+p^2\,p^\beta\,u^\mu\right)}{3\,(D-4)\,p^4}$$

$$(4\,\pi)^D\,\Pi^{\mu\beta}_{79}(p,\,k_1,\,k_2)=0$$

$$(4\,\pi)^D\,\Pi^{\mu\beta}_{80}(p,\,k_1,\,k_2)=0$$

$$(4\,\pi)^D\,\Pi^{\mu\beta}_{81}(p,\,k_1,\,k_2)=0$$

$$(4\,\pi)^D\,\Pi^{\mu\beta}_{82}(p,\,k_1,\,k_2)=0$$

$$(4\,\pi)^D\,\Pi^{\mu\beta}_{83}(p,\,k_1,\,k_2)=-\frac{i\,e^4\,Q_1\,(D\,(\xi-1)-3\,\xi+1)\,p^\beta\,u^\mu\,\mathbf{J}^{(D)}_{\{1,0\}\,\{1,0\}\,\{1,0\}}}{p^2}$$

$$(4\,\pi)^D\,\Pi^{\mu\beta}_{84}(p,\,k_1,\,k_2)=\frac{i\,e^4\,Q_1\,(D\,(\xi-1)-3\,\xi+1)\,p^\beta\,u^\mu\,\mathbf{J}^{(D)}_{\{1,0\}\,\{1,0\}\,\{1,0\}}}{p^2}$$

$$(4\,\pi)^D\,\Pi^{\mu\beta}_{85}(p,\,k_1,\,k_2)=0$$

$$(4\,\pi)^D\,\Pi^{\mu\beta}_{86}(p,\,k_1,\,k_2)=-\frac{8\,e^4\,Q_2\,\epsilon^{\beta\,\mu\,b\,p}\left((D-4)\,p^2\left(\mathbf{B}^{(D)}_{\{1,0\}\,\{1,0\}}\right)^2-2\,(D-3)\,D\,\mathbf{J}^{(D)}_{\{1,0\}\,\{1,0\}\,\{1,0\}}\right)}{(D-4)^2\,(D-1)\,p^2}$$

$$(4\,\pi)^D\,\Pi^{\mu\beta}_{87}(p,\,k_1,\,k_2)=-\frac{1}{3\,(D-4)\,p^4}i\,e^4\,Q_1\,(D\,(\xi-1)-3\,\xi+1)\,\mathbf{J}^{(D)}_{\{1,0\}\,\{1,0\}\,\{1,0\}}$$
$$\left(-4\,(D-3)\,p^2\,g^{\mu\,\beta}\,(p\cdot u)+2\,(D-3)\,p^2\,p^\beta\,u^\mu+p^\mu\left(2\,(D-3)\,p^2\,u^\beta+(D-4)\,D\,p^\beta\,(p\cdot u)\right)\right)$$

$$(4\,\pi)^D\,\Pi^{\mu\beta}_{88}(p,\,k_1,\,k_2) = \frac{1}{3\,(D-4)\,p^4} i\,\mathrm{e}^4\,Q_1\,(D\,(\xi-1)-3\,\xi+1)\,\mathbf{J}^{(D)}_{\{1,0\}\,\{1,0\}\,\{1,0\}}$$
$$\left(-4\,(D-3)\,p^2\,g^{\mu\,\beta}\,(p\cdot u)+2\,(D-3)\,p^2\,p^\beta\,u^\mu+p^\mu\left(2\,(D-3)\,p^2\,u^\beta+(D-4)\,D\,p^\beta\,(p\cdot u)\right)\right)$$
$$(4\,\pi)^D\,\Pi^{\mu\beta}_{89}(p,\,k_1,\,k_2) =$$
$$\frac{2\,i\,\mathrm{e}^4\,Q_1\,(D\,(\xi-1)-3\,\xi+1)\,\mathbf{J}^{(D)}_{\{1,0\}\,\{1,0\}\,\{1,0\}}\left(4\,(D-3)\,p^2\,g^{\mu\,\beta}\,(p\cdot u)+(D-6)\,p^2\,p^\beta\,u^\mu+p^\mu\left((D-6)\,p^2\,u^\beta-(D-4)\,D\,p^\beta\,(p\cdot u)\right)\right)}{3\,(D-6)\,(D-4)\,p^4}$$
$$(4\,\pi)^D\,\Pi^{\mu\beta}_{90}(p,\,k_1,\,k_2) = \frac{1}{3\,(D-6)\,(D-4)\,p^4} 2\,i\,\mathrm{e}^4\,Q_1\,(D\,(\xi-1)-3\,\xi+1)\,\mathbf{J}^{(D)}_{\{1,0\}\,\{1,0\}\,\{1,0\}}$$
$$\left(-4\,(D-3)\,p^2\,g^{\mu\,\beta}\,(p\cdot u)-(D-6)\,p^2\,p^\beta\,u^\mu+p^\mu\left((D-4)\,D\,p^\beta\,(p\cdot u)-(D-6)\,p^2\,u^\beta\right)\right)$$
$$(4\,\pi)^D\,\Pi^{\mu\beta}_{91}(p,\,k_1,\,k_2) =$$
$$\frac{2\,i\,\mathrm{e}^4\,Q_1\,(D\,(\xi-1)-3\,\xi+1)\,\mathbf{J}^{(D)}_{\{1,0\}\,\{1,0\}\,\{1,0\}}\left(4\,(D-3)\,p^2\,g^{\mu\,\beta}\,(p\cdot u)+(D-6)\,p^2\,p^\beta\,u^\mu+p^\mu\left((D-6)\,p^2\,u^\beta-(D-4)\,D\,p^\beta\,(p\cdot u)\right)\right)}{3\,(D-6)\,(D-4)\,p^4}$$
$$(4\,\pi)^D\,\Pi^{\mu\beta}_{92}(p,\,k_1,\,k_2) = \frac{1}{3\,(D-6)\,(D-4)\,p^4} 2\,i\,\mathrm{e}^4\,Q_1\,(D\,(\xi-1)-3\,\xi+1)\,\mathbf{J}^{(D)}_{\{1,0\}\,\{1,0\}\,\{1,0\}}$$
$$\left(-4\,(D-3)\,p^2\,g^{\mu\,\beta}\,(p\cdot u)-(D-6)\,p^2\,p^\beta\,u^\mu+p^\mu\left((D-4)\,D\,p^\beta\,(p\cdot u)-(D-6)\,p^2\,u^\beta\right)\right)$$
$$(4\,\pi)^D\,\Pi^{\mu\beta}_{93}(p,\,k_1,\,k_2) = 0$$
$$(4\,\pi)^D\,\Pi^{\mu\beta}_{94}(p,\,k_1,\,k_2) = 0$$
$$(4\,\pi)^D\,\Pi^{\mu\beta}_{95}(p,\,k_1,\,k_2) = 0$$
$$(4\,\pi)^D\,\Pi^{\mu\beta}_{96}(p,\,k_1,\,k_2) = 0$$

The diagrams shown in Figure 3 follow the format $\Sigma_i(p) = \int \frac{d^D k_1}{(2\pi)^D}\,\frac{d^D k_2}{(2\pi)^D}\,\tilde{\Sigma}_i(p, k_1, k_2)$,

and each individual contribution can be expresed as :

$$\tilde{\Sigma}_1(p, k_1, k_2) = -i\, e^2\, \lambda\, Q1\, (k_2\cdot u)\left(\frac{(\xi_{V(1)}-1)\left(2(k_1\cdot p)+k_1^2\right)\left(2(k_1\cdot k_2)+k_1^2\right)}{(k_2^2)^2.(k_1^2)^2.(k_1+p)^2.(k_1+k_2)^2} + \frac{2(k_1\cdot p + 2(k_2\cdot p) + k_1\cdot k_2) + k_1^2}{(k_2^2)^2.k_1^2.(k_1+p)^2.(k_1+k_2)^2}\right)$$

$$\tilde{\Sigma}_2(p, k_1, k_2) = -i\, e^2\, \lambda\, Q1\, (k_2\cdot u)\left(\frac{(\xi_{V(1)}-1)\left(2(k_1\cdot p)+k_1^2\right)\left(2(k_1\cdot k_2)+k_1^2\right)}{(k_2^2)^2.(k_1^2)^2.(k_1+p)^2.(k_1+k_2)^2} + \frac{2(k_1\cdot p + 2(k_2\cdot p) + k_1\cdot k_2) + k_1^2}{(k_2^2)^2.k_1^2.(k_1+p)^2.(k_1+k_2)^2}\right)$$

$$\tilde{\Sigma}_3(p, k_1, k_2) = -2\, i\, e^4\, Q1\, (k_2\cdot u)$$

$$\left((\xi_{V(1)}-1)\left((k_1^2-p^2)\left(\frac{(k_1^2-k_2^2)(\xi_{V(1)}-1)\left(k_1\cdot p + k_2\cdot p + k_1\cdot k_2 + k_1^2\right)}{(k_2^2)^2.k_1^2.(k_1+p)^{22}.(k_1+k_2)^{22}} + \frac{k_1\cdot p - k_2\cdot p - k_1\cdot k_2 + k_1^2}{(k_2^2)^2.k_1^2.(k_1+p)^{22}.(k_1+k_2)^2}\right) + \frac{(k_1^2-k_2^2)\left(-k_1\cdot p - k_2\cdot p + k_1\cdot k_2 + k_1^2\right)}{(k_2^2)^2.k_1^2.(k_1+p)^2.(k_1+k_2)^{22}}\right) + \frac{-k_1\cdot p + k_2\cdot p - k_1\cdot k_2 + k_1^2}{(k_2^2)^2.k_1^2.(k_1+p)^2.(k_1+k_2)^2}\right)$$

$$\tilde{\Sigma}_4(p, k_1, k_2) = -8\, e^4\, Q2\, \epsilon^{b\, k_1\, k_2\, p}\left(\frac{1}{(k_2^2)^2.k_1^2.(k_1+p)^2.(k_1+k_2)^2} - \frac{(k_1^2-p^2)(\xi_{V(1)}-1)}{(k_2^2)^2.k_1^2.(k_1+p)^{22}.(k_1+k_2)^2}\right)$$

$$\tilde{\Sigma}_5(p, k_1, k_2) = -i\, e^4\, Q1\left((\xi_{V(1)}-1)\right.$$

$$\left((k_2^2-p^2)(k_2\cdot u - p\cdot u)\left(\frac{(\xi_{V(1)}-1)\left(2(k_1\cdot p)+k_1^2\right)\left(2(k_1\cdot k_2)+k_1^2\right)}{k_2^2.(k_1^2)^2.(k_1+p)^2.(k_2-p)^{22}.(k_1+k_2)^2} + \frac{2(k_1\cdot p + 2(k_2\cdot p) + k_1\cdot k_2) + k_1^2}{k_2^2.k_1^2.(k_1+p)^2.(k_2-p)^{22}.(k_1+k_2)^2}\right) + \right.$$

$$\left.\left.\frac{\left(2(k_1\cdot p)+k_1^2\right)\left(2(k_1\cdot k_2)+k_1^2\right)(p\cdot u + k_2\cdot u)}{k_2^2.(k_1^2)^2.(k_1+p)^2.(k_2-p)^2.(k_1+k_2)^2}\right) + \frac{\left(2(k_1\cdot p + 2(k_2\cdot p) + k_1\cdot k_2) + k_1^2\right)(p\cdot u + k_2\cdot u)}{k_2^2.k_1^2.(k_1+p)^2.(k_2-p)^2.(k_1+k_2)^2}\right)$$

$$\tilde{\Sigma}_6(p, k_1, k_2) = i\, e^4\, Q1\left((\xi_{V(1)}-1)\left(\left(k_2^2 - 2(k_2\cdot p)\right)\left(2(k_1\cdot k_2)+k_2^2\right)\right.\right.$$

$$\left(\frac{(k_1^2-p^2)(\xi_{V(1)}-1)(p\cdot u + k_1\cdot u)}{(k_2^2)^2.k_1^2.(k_1+p)^{22}.(k_2-p)^2.(k_1+k_2)^2} + \frac{k_1\cdot u - p\cdot u}{(k_2^2)^2.k_1^2.(k_1+p)^2.(k_2-p)^2.(k_1+k_2)^2}\right) +$$

$$\left.\frac{(k_1^2-p^2)\left(-4(k_1\cdot p) - 2(k_2\cdot p) + 2(k_1\cdot k_2) + k_2^2\right)(p\cdot u + k_1\cdot u)}{k_2^2.k_1^2.(k_1+p)^{22}.(k_2-p)^2.(k_1+k_2)^2}\right) +$$

$$\left.\frac{\left(-4(k_1\cdot p) - 2(k_2\cdot p) + 2(k_1\cdot k_2) + k_2^2\right)(k_1\cdot u - p\cdot u)}{k_2^2.k_1^2.(k_1+p)^2.(k_2-p)^2.(k_1+k_2)^2}\right)$$

$$\tilde{\Sigma}_7(p, k_1, k_2) = i\, e^2\, \lambda\, Q1\, (k_1\cdot u)\left(\frac{(\xi_{V(1)}-1)\left(k_2^2 - 2(k_2\cdot p)\right)\left(2(k_1\cdot k_2)+k_2^2\right)}{k_1^2.(k_2^2)^2.k_1^2.(k_2-p)^2.(k_1+k_2)^2} + \frac{-4(k_1\cdot p) - 2(k_2\cdot p) + 2(k_1\cdot k_2) + k_2^2}{k_1^2.k_2^2.k_1^2.(k_2-p)^2.(k_1+k_2)^2}\right)$$

$$\tilde{\Sigma}_8(p, k_1, k_2) = i\, e^2\, \lambda\, Q1\, (k_1\cdot u)\left(\frac{(\xi_{V(1)}-1)\left(k_2^2 - 2(k_2\cdot p)\right)\left(2(k_1\cdot k_2)+k_2^2\right)}{k_1^2.(k_2^2)^2.k_1^2.(k_2-p)^2.(k_1+k_2)^2} + \frac{-4(k_1\cdot p) - 2(k_2\cdot p) + 2(k_1\cdot k_2) + k_2^2}{k_1^2.k_2^2.k_1^2.(k_2-p)^2.(k_1+k_2)^2}\right)$$

$$\tilde{\Sigma}_9(p, k_1, k_2) = -2\, i\, e^4\, Q1\, (k_1\cdot u)$$

$$\left((\xi_{V(1)}-1)\left((k_2^2-p^2)\left(\frac{(k_1^2-k_2^2)(\xi_{V(1)}-1)\left(-k_1\cdot p - k_2\cdot p + k_1\cdot k_2 + k_2^2\right)}{k_1^2.k_2^2.k_1^2.(k_2-p)^{22}.(k_1+k_2)^{22}} + \frac{-k_1\cdot p + k_2\cdot p + k_1\cdot k_2 - k_2^2}{k_1^2.k_2^2.k_1^2.(k_2-p)^{22}.(k_1+k_2)^2}\right) + \frac{(k_1^2-k_2^2)\left(k_1\cdot p + k_2\cdot p + k_1\cdot k_2 + k_2^2\right)}{k_1^2.k_2^2.k_1^2.(k_2-p)^2.(k_1+k_2)^{22}}\right) + \frac{k_1\cdot p - k_2\cdot p + k_1\cdot k_2 - k_2^2}{k_1^2.k_2^2.k_1^2.(k_2-p)^2.(k_1+k_2)^2}\right)$$

$$\tilde{\Sigma}_{10}(p, k_1, k_2) = -8\, e^4\, Q2\, \epsilon^{b\, k_1\, k_2\, p}\left(\frac{1}{k_1^2.k_2^2.k_1^2.(k_2-p)^2.(k_1+k_2)^2} - \frac{(k_2^2-p^2)(\xi_{V(1)}-1)}{k_1^2.k_2^2.k_1^2.(k_2-p)^{22}.(k_1+k_2)^2}\right)$$

$$\tilde{\Sigma}_{11}(p, k_1, k_2) = -i\, e^4\, Q1\, (k_2 \cdot u - p \cdot u) \Bigg( (\xi_{V(1)} - 1) \Bigg( \left(k_2{}^2 - 2\,(k_2 \cdot p)\right) \left(2\,(k_1 \cdot k_2) + k_2{}^2\right)$$

$$\Bigg( \frac{\left(k_1{}^2 - p^2\right)(\xi_{V(1)} - 1)\left(2\,(k_2 \cdot p) - p^2 + 2\,(k_1 \cdot k_2) + k_1{}^2\right)}{\left(k_2{}^2\right)^2 . k_1{}^2 .(k_1 + p)^{22} .(k_2 - p)^{22} .(k_1 + k_2)^2} + \frac{-2\,(k_1 \cdot p) - 2\,(k_2 \cdot p) + p^2 + 2\,(k_1 \cdot k_2) + k_1{}^2}{\left(k_2{}^2\right)^2 . k_1{}^2 .(k_1 + p)^2 .(k_2 - p)^{22} .(k_1 + k_2)^2} \Bigg) +$$

$$\frac{\left(k_1{}^2 - p^2\right)\left(-4\,(k_1 \cdot p) - 2\,(k_2 \cdot p) + 2\,(k_1 \cdot k_2) + k_2{}^2\right)\left(2\,(k_2 \cdot p) - p^2 + 2\,(k_1 \cdot k_2) + k_1{}^2\right)}{k_2{}^2 . k_1{}^2 .(k_1 + p)^{22} .(k_2 - p)^{22} .(k_1 + k_2)^2} \Bigg) +$$

$$\frac{\left(-4\,(k_1 \cdot p) - 2\,(k_2 \cdot p) + 2\,(k_1 \cdot k_2) + k_2{}^2\right)\left(-2\,(k_1 \cdot p) - 2\,(k_2 \cdot p) + p^2 + 2\,(k_1 \cdot k_2) + k_1{}^2\right)}{k_2{}^2 . k_1{}^2 .(k_1 + p)^2 .(k_2 - p)^{22} .(k_1 + k_2)^2} \Bigg)$$

$$\tilde{\Sigma}_{12}(p, k_1, k_2) = 8\, e^4\, Q2\, \epsilon^{b\, k_1\, k_2\, p} \left( \frac{(\xi_{V(1)} - 1)\left(2\,(k_1 \cdot p) + k_1{}^2\right)\left(2\,(k_1 \cdot k_2) + k_1{}^2\right)}{k_2{}^2 .\left(k_1{}^2\right)^2 .(k_1 + p)^2 .(k_2 - p)^{22} .(k_1 + k_2)^2} + \frac{2\,(k_1 \cdot p + 2\,(k_2 \cdot p) + k_1 \cdot k_2) + k_1{}^2}{k_2{}^2 . k_1{}^2 .(k_1 + p)^2 .(k_2 - p)^{22} .(k_1 + k_2)^2} \right)$$

$$\tilde{\Sigma}_{13}(p, k_1, k_2) = i\, e^4\, Q1\, (k_1 \cdot u) \Bigg( (\xi_{V(1)} - 1) \Bigg( \left(k_2{}^2 - p^2\right)\left(-2\,(k_1 \cdot p) - 2\,(k_2 \cdot p) + p^2 + 2\,(k_1 \cdot k_2) + k_2{}^2\right)$$

$$\Bigg( \frac{\left(k_1{}^2 - p^2\right)(\xi_{V(1)} - 1)\left(-2\,(k_1 \cdot p) - 2\,(k_2 \cdot p) + p^2 + 2\,(k_1 \cdot k_2) + k_1{}^2\right)}{k_1{}^2 . k_2{}^2 . k_1{}^2 .(k_1 - p)^{22} .(k_2 - p)^{22} .(k_1 + k_2 - p)^2} +$$

$$\frac{2\,(k_2 \cdot p) - p^2 + 2\,(k_1 \cdot k_2) + k_1{}^2}{k_1{}^2 . k_2{}^2 . k_1{}^2 .(k_1 - p)^2 .(k_2 - p)^{22} .(k_1 + k_2 - p)^2} \Bigg) +$$

$$\frac{\left(k_1{}^2 - p^2\right)\left(2\,(k_1 \cdot p) - p^2 + 2\,(k_1 \cdot k_2) + k_2{}^2\right)\left(-2\,(k_1 \cdot p) - 2\,(k_2 \cdot p) + p^2 + 2\,(k_1 \cdot k_2) + k_1{}^2\right)}{k_1{}^2 . k_2{}^2 . k_1{}^2 .(k_1 - p)^{22} .(k_2 - p)^2 .(k_1 + k_2 - p)^2} \Bigg) +$$

$$\frac{\left(2\,(k_1 \cdot p) - p^2 + 2\,(k_1 \cdot k_2) + k_2{}^2\right)\left(2\,(k_2 \cdot p) - p^2 + 2\,(k_1 \cdot k_2) + k_1{}^2\right)}{k_1{}^2 . k_2{}^2 . k_1{}^2 .(k_1 - p)^2 .(k_2 - p)^2 .(k_1 + k_2 - p)^2} \Bigg)$$

$$\tilde{\Sigma}_{14}(p, k_1, k_2) = 8\, e^4\, Q2\, \epsilon^{b\, k_1\, k_2\, p} \Bigg( \frac{(\xi_{V(1)} - 1)\left(k_2{}^2 - 2\,(k_2 \cdot p)\right)\left(-2\,(k_2 \cdot p) + 2\,(k_1 \cdot k_2) + k_2{}^2\right)}{k_1{}^2 .\left(k_2{}^2\right)^2 . k_1{}^2 .(k_1 - p)^2 .(k_2 - p)^2 .(k_1 + k_2 - p)^2} +$$

$$\frac{-4\,(k_1 \cdot p) - 4\,(k_2 \cdot p) + 4\,p^2 + 2\,(k_1 \cdot k_2) + k_2{}^2}{k_1{}^2 . k_2{}^2 . k_1{}^2 .(k_1 - p)^2 .(k_2 - p)^2 .(k_1 + k_2 - p)^2} \Bigg)$$

$$\tilde{\Sigma}_{15}(p, k_1, k_2) = i\, e^4\, Q1\, (k_2 \cdot u) \Bigg( \left(k_1{}^2 - p^2\right)(\xi_{V(1)} - 1)\left(-2\,(k_1 \cdot p) - 2\,(k_2 \cdot p) + p^2 + 2\,(k_1 \cdot k_2) + k_1{}^2\right)$$

$$\Bigg( \frac{\left(k_1{}^2 - p^2\right)(\xi_{V(1)} - 1)\left(-2\,(k_1 \cdot p) - 2\,(k_2 \cdot p) + p^2 + 2\,(k_1 \cdot k_2) + k_1{}^2\right)}{\left(k_2{}^2\right)^2 . k_1{}^2 .(k_1 - p)^{24} .(k_1 + k_2 - p)^2} + \frac{2\left(2\,(k_2 \cdot p) - p^2 + 2\,(k_1 \cdot k_2) + k_1{}^2\right)}{\left(k_2{}^2\right)^2 . k_1{}^2 .(k_1 - p)^{23} .(k_1 + k_2 - p)^2} \Bigg) +$$

$$\frac{\left(2\,(k_2 \cdot p) - p^2 + 2\,(k_1 \cdot k_2) + k_1{}^2\right)^2}{\left(k_2{}^2\right)^2 . k_1{}^2 .(k_1 - p)^{22} .(k_1 + k_2 - p)^2} \Bigg)$$

$$\tilde{\Sigma}_{16}(p, k_1, k_2) = -i\, e^4\, Q1\, (k_2 \cdot u) \Bigg( \left(k_1{}^2 - p^2\right)(\xi_{V(1)} - 1)\left(-2\,(k_1 \cdot p) - 2\,(k_2 \cdot p) + p^2 + 2\,(k_1 \cdot k_2) + k_1{}^2\right)$$

$$\Bigg( \frac{\left(k_1{}^2 - p^2\right)(\xi_{V(1)} - 1)\left(-2\,(k_1 \cdot p) - 2\,(k_2 \cdot p) + p^2 + 2\,(k_1 \cdot k_2) + k_1{}^2\right)}{\left(k_2{}^2\right)^2 . k_1{}^2 .(k_1 - p)^{24} .(k_1 + k_2 - p)^2} + \frac{2\left(2\,(k_2 \cdot p) - p^2 + 2\,(k_1 \cdot k_2) + k_1{}^2\right)}{\left(k_2{}^2\right)^2 . k_1{}^2 .(k_1 - p)^{23} .(k_1 + k_2 - p)^2} \Bigg) +$$

$$\frac{\left(2\,(k_2 \cdot p) - p^2 + 2\,(k_1 \cdot k_2) + k_1{}^2\right)^2}{\left(k_2{}^2\right)^2 . k_1{}^2 .(k_1 - p)^{22} .(k_1 + k_2 - p)^2} \Bigg)$$

$$\tilde{\Sigma}_{17}(p, k_1, k_2) = i\, e^4\, Q1\, (k_2 \cdot u) \Bigg( (\xi_{V(1)} - 1)$$

$$\left(\left(-2\,(k_1\cdot p)+p^2+k_1{}^2-k_2{}^2\right)^2\left(\frac{(\xi_{V(1)}-1)\left(k_1{}^2-2\,(k_1\cdot p)\right)^2}{\left(k_2{}^2\right)^2.\left(k_1{}^2\right)^2.(\,k_1-p\,)^{22}.(\,k_1+k_2-p\,)^{22}}+\frac{-4\,(k_1\cdot p)+4\,p^2+k_1{}^2}{\left(k_2{}^2\right)^2.k_1{}^2.(\,k_1-p\,)^{22}.(\,k_1+k_2-p\,)^{22}}\right)+\right.$$

$$\left.\frac{\left(k_1{}^2-2\,(k_1\cdot p)\right)^2\left(-2\,(k_1\cdot p)+2\,(k_2\cdot p)+p^2-2\,(k_1\cdot k_2)+k_1{}^2+k_2{}^2\right)}{\left(k_2{}^2\right)^2.\left(k_1{}^2\right)^2.(\,k_1-p\,)^{22}.(\,k_1+k_2-p\,)^2}\right)+$$

$$\left.\frac{\left(-4\,(k_1\cdot p)+4\,p^2+k_1{}^2\right)\left(-2\,(k_1\cdot p)+2\,(k_2\cdot p)+p^2-2\,(k_1\cdot k_2)+k_1{}^2+k_2{}^2\right)}{\left(k_2{}^2\right)^2.k_1{}^2.(\,k_1-p\,)^{22}.(\,k_1+k_2-p\,)^2}\right)$$

$$\tilde{\Sigma}_{18}(p,k_1,k_2)=0$$

$$\tilde{\Sigma}_{19}(p,k_1,k_2)=i\,\mathrm{e}^2\,\lambda\,\mathrm{Q1}\left(\frac{\left(k_1{}^2-p^2\right)(\xi_{V(1)}-1)\,(k_1\cdot u-p\cdot u)}{k_2{}^2.k_1{}^2.(\,k_1-p\,)^{22}.(\,-k_1+k_2+p\,)^2}+\frac{p\cdot u+k_1\cdot u}{k_2{}^2.k_1{}^2.(\,k_1-p\,)^2.(\,-k_1+k_2+p\,)^2}\right)$$

$$\tilde{\Sigma}_{20}(p,k_1,k_2)=-2\,i\,\mathrm{e}^4\,\mathrm{Q1}\left((\xi_{V(1)}-1)\left((-p\cdot u+k_1\cdot u-k_2\cdot u)\right.\right.$$

$$\left(\frac{(\xi_{V(1)}-1)\left(k_1{}^2-2\,(k_1\cdot p)\right)\left(-k_1\cdot p-k_1\cdot k_2+k_1{}^2\right)}{k_2{}^2.\left(k_1{}^2\right)^2.(\,k_1-p\,)^2.(\,-k_1+k_2+p\,)^{22}}+\frac{-3\,(k_1\cdot p)+2\,(k_2\cdot p)+2\,p^2-k_1\cdot k_2+k_1{}^2}{k_2{}^2.k_1{}^2.(\,k_1-p\,)^2.(\,-k_1+k_2+p\,)^{22}}\right)+$$

$$\left.\left.\frac{\left(k_1{}^2-2\,(k_1\cdot p)\right)(k_1\cdot u)}{k_2{}^2.\left(k_1{}^2\right)^2.(\,k_1-p\,)^2.(\,-k_1+k_2+p\,)^2}\right)+\frac{k_1\cdot u-2\,(p\cdot u)}{k_2{}^2.k_1{}^2.(\,k_1-p\,)^2.(\,-k_1+k_2+p\,)^2}\right)$$

$$\tilde{\Sigma}_{21}(p,k_1,k_2)=-i\,\mathrm{e}^2\,\lambda\,\mathrm{Q1}\left(\frac{(\xi_{V(1)}-1)\left(k_1{}^2-2\,(k_1\cdot p)\right)(k_1\cdot u)}{\left(k_1{}^2\right)^2.k_2{}^2.(\,k_1-p\,)^{22}}+\frac{k_1\cdot u-2\,(p\cdot u)}{k_1{}^2.k_2{}^2.(\,k_1-p\,)^{22}}\right)$$

$$\tilde{\Sigma}_{22}(p,k_1,k_2)=$$

$$2\,i\,\mathrm{e}^4\,\mathrm{Q1}\left(\left(k_1{}^2-p^2\right)(\xi_{V(1)}-1)\,(k_1\cdot u-p\cdot u)\left(\frac{(\xi_{V(1)}-1)\left(-2\,(k_1\cdot p)+p^2+k_1{}^2\right)}{k_1{}^2.k_2{}^2.(\,k_1-p\,)^{24}}+\frac{2}{k_1{}^2.k_2{}^2.(\,k_1-p\,)^{23}}\right)+\frac{p\cdot u+k_1\cdot u}{k_1{}^2.k_2{}^2.(\,k_1-p\,)^{22}}\right)$$

$$\tilde{\Sigma}_{23}(p,k_1,k_2)=$$

$$-i\,\mathrm{e}^4\,\mathrm{Q1}\left((\xi_{V(1)}-1)\left(\frac{D\left(k_1{}^2-2\,(k_1\cdot p)\right)(k_1\cdot u)}{\left(k_1{}^2\right)^2.k_2{}^2.(\,k_1-p\,)^{22}}+k_2{}^2\left(\frac{(\xi_{V(1)}-1)\left(k_1{}^2-2\,(k_1\cdot p)\right)(k_1\cdot u)}{\left(k_1{}^2\right)^2.\left(k_2{}^2\right)^2.(\,k_1-p\,)^{22}}+\frac{k_1\cdot u-2\,(p\cdot u)}{k_1{}^2.\left(k_2{}^2\right)^2.(\,k_1-p\,)^{22}}\right)\right)+\right.$$

$$\left.\frac{D\,(k_1\cdot u-2\,(p\cdot u))}{k_1{}^2.k_2{}^2.(\,k_1-p\,)^{22}}\right)$$

$$\tilde{\Sigma}_{24}(p,k_1,k_2)=\frac{i\,\lambda^2\,\mathrm{Q1}\,(k_1\cdot u)}{k_1{}^2.k_2{}^2.k_1{}^2.(\,-k_1+k_2+p\,)^2}$$

$$\tilde{\Sigma}_{25}(p,k_1,k_2)=-\frac{i\,\lambda^2\,\mathrm{Q1}\,(k_1\cdot u)}{2\,k_1{}^2.k_2{}^2.k_1{}^2.(\,-k_1+k_2+p\,)^2}$$

$$\tilde{\Sigma}_{26}(p,k_1,k_2)=2\,i\,\mathrm{e}^4\,\mathrm{Q1}\,(k_1\cdot u)$$

$$\left(\frac{D}{k_1{}^2.k_2{}^2.k_1{}^2.(\,-k_1+k_2+p\,)^2}+(\xi_{V(1)}-1)\left(\frac{(\xi_{V(1)}-1)\left(k_2\cdot p-(k_1\cdot k_2)+k_2{}^2\right)^2}{k_1{}^2.\left(k_2{}^2\right)^2.k_1{}^2.(\,-k_1+k_2+p\,)^{22}}+\frac{k_2{}^2}{k_1{}^2.\left(k_2{}^2\right)^2.k_1{}^2.(\,-k_1+k_2+p\,)^2}+\right.\right.$$

$$\left.\left.\frac{-2\,(k_1\cdot p)+2\,(k_2\cdot p)+p^2-2\,(k_1\cdot k_2)+k_1{}^2+k_2{}^2}{k_1{}^2.k_2{}^2.k_1{}^2.(\,-k_1+k_2+p\,)^{22}}\right)\right)$$

$$\tilde{\Sigma}_{27}(p,k_1,k_2)=0$$

$$\tilde{\Sigma}_{28}(p,k_1,k_2)=i\,\mathrm{e}^2\,\lambda\,\mathrm{Q1}\left(\frac{(\xi_{V(1)}-1)\left(2\,(k_1\cdot p)+k_1{}^2\right)(k_1\cdot u)}{k_2{}^2.\left(k_1{}^2\right)^2.(\,k_1+p\,)^2.(\,k_2-k_1\,)^2}+\frac{2\,(p\cdot u)+k_1\cdot u}{k_2{}^2.k_1{}^2.(\,k_1+p\,)^2.(\,k_2-k_1\,)^2}\right)$$

$$\tilde{\Sigma}_{29}(p,k_1,k_2)=$$

$$-2\,i\,\mathrm{e}^4\,\mathrm{Q1}\left((\xi_{V(1)}-1)\left(\left(k_1{}^2-p^2\right)\left(\frac{(\xi_{V(1)}-1)\left(k_1\cdot p-k_2\cdot p-k_1\cdot k_2+k_1{}^2\right)(k_1\cdot u-k_2\cdot u)}{k_2{}^2.k_1{}^2.(\,k_1+p\,)^{22}.(\,k_2-k_1\,)^{22}}+\frac{p\cdot u+k_1\cdot u}{k_2{}^2.k_1{}^2.(\,k_1+p\,)^{22}.(\,k_2-k_1\,)^2}\right)+\right.\right.$$

$$\frac{\left(-k_1\cdot p+k_2\cdot p-k_1\cdot k_2+{k_1}^2\right)(k_1\cdot u-k_2\cdot u)}{{k_2}^2.{k_1}^2.(k_1+p)^2.(k_2-k_1)^{22}}\Bigg)+\frac{k_1\cdot u-p\cdot u}{{k_2}^2.{k_1}^2.(k_1+p)^2.(k_2-k_1)^2}\Bigg)$$

$$\tilde{\Sigma}_{30}(p,k_1,k_2)=-i\,\mathrm{e}^2\,\lambda\,\mathrm{Q1}\left(\frac{\left({k_1}^2-{k_2}^2\right)(\xi_{V(1)}-1)(k_1\cdot u+k_2\cdot u)}{{k_2}^2.{k_1}^2.(k_1+k_2)^{22}.(k_1+k_2+p)^2}+\frac{k_1\cdot u-k_2\cdot u}{{k_2}^2.{k_1}^2.(k_1+k_2)^2.(k_1+k_2+p)^2}\right)$$

$$\tilde{\Sigma}_{31}(p,k_1,k_2)=-2\,i\,\mathrm{e}^4\,\mathrm{Q1}$$
$$\left((\xi_{V(1)}-1)\left(\left(2(k_1\cdot k_2)+{k_2}^2\right)\left(\frac{(\xi_{V(1)}-1)\left(k_2\cdot p+k_1\cdot k_2+{k_2}^2\right)(p\cdot u+k_1\cdot u+k_2\cdot u)}{\left({k_2}^2\right)^2.{k_1}^2.(k_1+k_2)^2.(k_1+k_2+p)^{22}}+\frac{k_2\cdot u}{\left({k_2}^2\right)^2.{k_1}^2.(k_1+k_2)^2.(k_1+k_2+p)^2}\right)+\right.\right.$$
$$\left.\left.\frac{\left(2(k_1\cdot p)+k_2\cdot p+3(k_1\cdot k_2)+2{k_1}^2+{k_2}^2\right)(p\cdot u+k_1\cdot u+k_2\cdot u)}{{k_2}^2.{k_1}^2.(k_1+k_2)^2.(k_1+k_2+p)^{22}}\right)+\frac{2(k_1\cdot u)+k_2\cdot u}{{k_2}^2.{k_1}^2.(k_1+k_2)^2.(k_1+k_2+p)^2}\right)$$

$$\tilde{\Sigma}_{32}(p,k_1,k_2)=-\frac{i\,\lambda^2\,\mathrm{Q1}\,(k_1\cdot u)}{\left({k_1}^2\right)^3.{k_2}^2}$$

$$\tilde{\Sigma}_{33}(p,k_1,k_2)=\frac{i\,\lambda^2\,\mathrm{Q1}\,(k_1\cdot u)}{\left({k_1}^2\right)^3.{k_2}^2}$$

$$\tilde{\Sigma}_{34}(p,k_1,k_2)=-i\,\mathrm{e}^2\,\lambda\,\mathrm{Q1}\,(k_1\cdot u)\left(\frac{D}{\left({k_1}^2\right)^3.{k_2}^2}+\frac{{k_2}^2(\xi_{V(1)}-1)}{\left({k_1}^2\right)^3.\left({k_2}^2\right)^2}\right)$$

$$\tilde{\Sigma}_{35}(p,k_1,k_2)=i\,\mathrm{e}^2\,\lambda\,\mathrm{Q1}\,(k_1\cdot u)\left(\frac{D}{\left({k_1}^2\right)^3.{k_2}^2}+\frac{{k_2}^2(\xi_{V(1)}-1)}{\left({k_1}^2\right)^3.\left({k_2}^2\right)^2}\right)$$

$$\tilde{\Sigma}_{36}(p,k_1,k_2)=0$$

$$\tilde{\Sigma}_{37}(p,k_1,k_2)=i\,\mathrm{e}^2\,\lambda\,\mathrm{Q1}\left(\frac{(\xi_{V(1)}-1)\left(2(k_1\cdot k_2)+{k_2}^2\right)(k_2\cdot u)}{\left({k_2}^2\right)^2.{k_1}^2.(k_1+k_2)^{22}}+\frac{2(k_1\cdot u)+k_2\cdot u}{{k_2}^2.{k_1}^2.(k_1+k_2)^{22}}\right)$$

$$\tilde{\Sigma}_{38}(p,k_1,k_2)=-i\,\mathrm{e}^2\,\lambda\,\mathrm{Q1}\left(\frac{(\xi_{V(1)}-1)\left(2(k_1\cdot k_2)+{k_2}^2\right)(k_2\cdot u)}{\left({k_2}^2\right)^2.{k_1}^2.(k_1+k_2)^{22}}+\frac{2(k_1\cdot u)+k_2\cdot u}{{k_2}^2.{k_1}^2.(k_1+k_2)^{22}}\right)$$

$$\tilde{\Sigma}_{39}(p,k_1,k_2)=-2\,i\,\mathrm{e}^4\,\mathrm{Q1}$$
$$\left(\left({k_1}^2-{k_2}^2\right)(\xi_{V(1)}-1)(k_1\cdot u+k_2\cdot u)\left(\frac{(\xi_{V(1)}-1)\left(2(k_1\cdot k_2)+{k_1}^2+{k_2}^2\right)}{{k_2}^2.{k_1}^2.(k_1+k_2)^{24}}+\frac{2}{{k_2}^2.{k_1}^2.(k_1+k_2)^{23}}\right)+\frac{k_1\cdot u-k_2\cdot u}{{k_2}^2.{k_1}^2.(k_1+k_2)^{22}}\right)$$

$$\tilde{\Sigma}_{40}(p,k_1,k_2)=i\,\mathrm{e}^2\,\lambda\,\mathrm{Q1}\left(\frac{(\xi_{V(1)}-1)\left(2(k_1\cdot p)+{k_1}^2\right)(k_1\cdot u)}{\left({k_1}^2\right)^2.{k_2}^2.(k_1+p)^{22}}+\frac{2(p\cdot u)+k_1\cdot u}{{k_1}^2.{k_2}^2.(k_1+p)^{22}}\right)$$

$$\tilde{\Sigma}_{41}(p,k_1,k_2)=$$
$$-2\,i\,\mathrm{e}^4\,\mathrm{Q1}\left(\left({k_1}^2-p^2\right)(\xi_{V(1)}-1)(p\cdot u+k_1\cdot u)\left(\frac{(\xi_{V(1)}-1)\left(2(k_1\cdot p)+p^2+{k_1}^2\right)}{{k_1}^2.{k_2}^2.(k_1+p)^{24}}+\frac{2}{{k_1}^2.{k_2}^2.(k_1+p)^{23}}\right)+\frac{k_1\cdot u-p\cdot u}{{k_1}^2.{k_2}^2.(k_1+p)^{22}}\right)$$

$$\tilde{\Sigma}_{42}(p,k_1,k_2)=$$
$$i\,\mathrm{e}^4\,\mathrm{Q1}\left((\xi_{V(1)}-1)\left(\frac{D\left(2(k_1\cdot p)+{k_1}^2\right)(k_1\cdot u)}{\left({k_1}^2\right)^2.{k_2}^2.(k_1+p)^{22}}+{k_2}^2\left(\frac{(\xi_{V(1)}-1)\left(2(k_1\cdot p)+{k_1}^2\right)(k_1\cdot u)}{\left({k_1}^2\right)^2.\left({k_2}^2\right)^2.(k_1+p)^{22}}+\frac{2(p\cdot u)+k_1\cdot u}{{k_1}^2.\left({k_2}^2\right)^2.(k_1+p)^{22}}\right)\right)+\right.$$
$$\left.\frac{D(2(p\cdot u)+k_1\cdot u)}{{k_1}^2.{k_2}^2.(k_1+p)^{22}}\right)$$

$$\tilde{\Sigma}_{43}(p,k_1,k_2)=-i\,\mathrm{e}^2\,\lambda\,\mathrm{Q1}\left(\frac{\left({k_1}^2-{k_2}^2\right)(\xi_{V(1)}-1)(k_1\cdot u+k_2\cdot u)}{{k_2}^2.{k_1}^2.(k_1+k_2)^{22}.(k_1+k_2-p)^2}+\frac{k_1\cdot u-k_2\cdot u}{{k_2}^2.{k_1}^2.(k_1+k_2)^2.(k_1+k_2-p)^2}\right)$$

$$\tilde{\Sigma}_{44}(p,k_1,k_2)=2\,i\,\mathrm{e}^4\,\mathrm{Q1}\left((\xi_{V(1)}-1)\right.$$

$$\left(\left(2\,(k_1\cdot k_2)+k_2{}^2\right)\left(\frac{(\xi_{V(1)}-1)\left(-k_2\cdot p+k_1\cdot k_2+k_2{}^2\right)(-p\cdot u+k_1\cdot u+k_2\cdot u)}{\left(k_2{}^2\right)^2.k_1{}^2.(k_1+k_2)^2.(k_1+k_2-p)^{22}}+\frac{k_2\cdot u}{\left(k_2{}^2\right)^2.k_1{}^2.(k_1+k_2)^2.(k_1+k_2-p)^2}\right)+\right.$$

$$\left.\frac{\left(-2\,(k_1\cdot p)-k_2\cdot p+3\,(k_1\cdot k_2)+2\,k_1{}^2+k_2{}^2\right)(-p\cdot u+k_1\cdot u+k_2\cdot u)}{k_2{}^2.k_1{}^2.(k_1+k_2)^2.(k_1+k_2-p)^{22}}\right)+\frac{2\,(k_1\cdot u)+k_2\cdot u}{k_2{}^2.k_1{}^2.(k_1+k_2)^2.(k_1+k_2-p)^2}\Bigg)$$

$$\tilde{\Sigma}_{45}(p,k_1,k_2)=-i\,e^2\,\lambda\,\mathrm{Q1}\,(k_1\cdot u)\left(\frac{\left(k_1{}^2-p^2\right)^2(\xi_{V(1)}-1)}{\left(k_1{}^2\right)^3.k_2{}^2.(k_1-p)^{22}}+\frac{2\,(k_1\cdot p)+p^2+k_1{}^2}{\left(k_1{}^2\right)^3.k_2{}^2.(k_1-p)^2}\right)$$

$$\tilde{\Sigma}_{46}(p,k_1,k_2)=-i\,e^4\,\mathrm{Q1}\,(k_1\cdot u)$$

$$\left((\xi_{V(1)}-1)\left(\frac{D\left(k_1{}^2-p^2\right)^2}{\left(k_1{}^2\right)^3.k_2{}^2.(k_1-p)^{22}}+k_2{}^2\left(\frac{\left(k_1{}^2-p^2\right)^2(\xi_{V(1)}-1)}{\left(k_1{}^2\right)^3.\left(k_2{}^2\right)^2.(k_1-p)^{22}}+\frac{2\,(k_1\cdot p)+p^2+k_1{}^2}{\left(k_1{}^2\right)^3.\left(k_2{}^2\right)^2.(k_1-p)^2}\right)\right)+\frac{D\left(2\,(k_1\cdot p)+p^2+k_1{}^2\right)}{\left(k_1{}^2\right)^3.k_2{}^2.(k_1-p)^2}\right)$$

$$\tilde{\Sigma}_{47}(p,k_1,k_2)=0$$

$$\tilde{\Sigma}_{48}(p,k_1,k_2)=$$

$$-2\,i\,e^4\,\mathrm{Q1}\,(k_1\cdot u)\left(\left(k_1{}^2-p^2\right)^2(\xi_{V(1)}-1)\left(\frac{(\xi_{V(1)}-1)\left(-2\,(k_1\cdot p)+p^2+k_1{}^2\right)}{\left(k_1{}^2\right)^2.k_2{}^2.(k_1-p)^{24}}+\frac{2}{\left(k_1{}^2\right)^2.k_2{}^2.(k_1-p)^{23}}\right)+\frac{2\,(k_1\cdot p)+p^2+k_1{}^2}{\left(k_1{}^2\right)^2.k_2{}^2.(k_1-p)^{22}}\right)$$

$$\tilde{\Sigma}_{49}(p,k_1,k_2)=0$$

$$\tilde{\Sigma}_{50}(p,k_1,k_2)=0$$

$$\tilde{\Sigma}_{51}(p,k_1,k_2)=$$

$$2\,i\,e^4\,\mathrm{Q1}\,(k_1\cdot u)\left((\xi_{V(1)}-1)\left(\left(k_2{}^2-p^2\right)\left(\frac{\left(k_1{}^2-p^2\right)(\xi_{V(1)}-1)\left(k_1\cdot p-k_2\cdot p-p^2+k_1\cdot k_2\right)}{\left(k_1{}^2\right)^2.k_2{}^2.(k_1-p)^{22}.(k_2+p)^{22}}+\frac{k_1\cdot p+k_2\cdot p+p^2+k_1\cdot k_2}{k_2{}^2.\left(k_1{}^2\right)^2.(k_2+p)^{22}.(k_1-p)^2}\right)+\right.\right.$$

$$\left.\left.\frac{\left(k_1{}^2-p^2\right)\left(-k_1\cdot p-k_2\cdot p+p^2+k_1\cdot k_2\right)}{\left(k_1{}^2\right)^2.k_2{}^2.(k_1-p)^{22}.(k_2+p)^2}\right)+\frac{-k_1\cdot p+k_2\cdot p-p^2+k_1\cdot k_2}{\left(k_1{}^2\right)^2.k_2{}^2.(k_1-p)^2.(k_2+p)^2}\right)$$

$$\tilde{\Sigma}_{52}(p,k_1,k_2)=-8\,e^4\,\mathrm{Q2}\,\epsilon^{b\,k_1\,k_2\,p}\left(\frac{\left(k_2{}^2-p^2\right)(\xi_{V(1)}-1)}{k_2{}^2.\left(k_1{}^2\right)^2.(k_2+p)^{22}.(k_1-p)^2}+\frac{1}{\left(k_1{}^2\right)^2.k_2{}^2.(k_1-p)^2.(k_2+p)^2}\right)$$

$$\tilde{\Sigma}_{53}(p,k_1,k_2)=i\,e^2\,\lambda\,\mathrm{Q1}\,(k_1\cdot u-p\cdot u)\left(\frac{(\xi_{V(1)}-1)\left(k_1{}^2-2\,(k_1\cdot p)\right)^2}{\left(k_1{}^2\right)^2.k_2{}^2.(k_1-p)^{23}}+\frac{-4\,(k_1\cdot p)+4\,p^2+k_1{}^2}{k_1{}^2.k_2{}^2.(k_1-p)^{23}}\right)$$

$$\tilde{\Sigma}_{54}(p,k_1,k_2)=$$

$$i\,e^4\,\mathrm{Q1}\,(k_1\cdot u-p\cdot u)\left((\xi_{V(1)}-1)\left(\frac{D\left(k_1{}^2-2\,(k_1\cdot p)\right)^2}{\left(k_1{}^2\right)^2.k_2{}^2.(k_1-p)^{23}}+k_2{}^2\left(\frac{(\xi_{V(1)}-1)\left(k_1{}^2-2\,(k_1\cdot p)\right)^2}{\left(k_1{}^2\right)^2.\left(k_2{}^2\right)^2.(k_1-p)^{23}}+\frac{-4\,(k_1\cdot p)+4\,p^2+k_1{}^2}{k_1{}^2.\left(k_2{}^2\right)^2.(k_1-p)^{23}}\right)\right)+\right.$$

$$\left.\frac{D\left(-4\,(k_1\cdot p)+4\,p^2+k_1{}^2\right)}{k_1{}^2.k_2{}^2.(k_1-p)^{23}}\right)$$

$$\tilde{\Sigma}_{55}(p,k_1,k_2)=0$$

$$\tilde{\Sigma}_{56}(p,k_1,k_2)=i\,e^2\,\lambda\,\mathrm{Q1}\,(k_2\cdot u)\left(\frac{(\xi_{V(1)}-1)\left(k_1{}^2-2\,(k_1\cdot p)\right)^2}{\left(k_1{}^2\right)^2.\left(k_2{}^2\right)^2.(k_1-p)^{22}}+\frac{-4\,(k_1\cdot p)+4\,p^2+k_1{}^2}{k_1{}^2.\left(k_2{}^2\right)^2.(k_1-p)^{22}}\right)$$

$$\tilde{\Sigma}_{57}(p,k_1,k_2)=$$

$$2\,i\,e^4\,\mathrm{Q1}\,(k_2\cdot u)\left(\left(k_1{}^2-p^2\right)^2(\xi_{V(1)}-1)\left(\frac{(\xi_{V(1)}-1)\left(-2\,(k_1\cdot p)+p^2+k_1{}^2\right)}{k_1{}^2.\left(k_2{}^2\right)^2.(k_1-p)^{24}}+\frac{2}{k_1{}^2.\left(k_2{}^2\right)^2.(k_1-p)^{23}}\right)+\frac{2\,(k_1\cdot p)+p^2+k_1{}^2}{k_1{}^2.\left(k_2{}^2\right)^2.(k_1-p)^{22}}\right)$$

$$\tilde{\Sigma}_{58}(p,k_1,k_2)=0$$

$$\tilde{\Sigma}_{59}(p,k_1,k_2)=-2\,i\,e^4\,\mathrm{Q1}\,(k_2\cdot u)$$

$$\left((\xi_{V(1)}-1)\left(\left(k_2{}^2-p^2\right)\left(\frac{\left(k_1{}^2-p^2\right)(\xi_{V(1)}-1)\left(-k_1\cdot p-k_2\cdot p+p^2+k_1\cdot k_2\right)}{\left(k_2{}^2\right)^2.k_1{}^2.(k_2-p)^{22}.(k_1-p)^{22}}+\frac{-k_1\cdot p+k_2\cdot p-p^2+k_1\cdot k_2}{\left(k_2{}^2\right)^2.k_1{}^2.(k_2-p)^{22}.(k_1-p)^2}\right)+\right.\right.$$

$$\frac{\left(k_1{}^2-p^2\right)\left(k_1\cdot p-k_2\cdot p-p^2+k_1\cdot k_2\right)}{\left(k_2{}^2\right)^2.k_1{}^2.(k_2-p)^2.(k_1-p)^{22}}\Bigg)+\frac{k_1\cdot p+k_2\cdot p+p^2+k_1\cdot k_2}{\left(k_2{}^2\right)^2.k_1{}^2.(k_2-p)^2.(k_1-p)^2}\Bigg)$$

$$\tilde{\Sigma}_{60}(p,k_1,k_2)=8\,\mathrm{e}^4\,\mathrm{Q2}\,\epsilon^{b\,k_1\,k_2\,p}\left(\frac{\left(k_1{}^2-p^2\right)\left(\xi_{V(1)}-1\right)}{\left(k_2{}^2\right)^2.k_1{}^2.(k_2-p)^2.(k_1-p)^{22}}+\frac{1}{\left(k_2{}^2\right)^2.k_1{}^2.(k_2-p)^2.(k_1-p)^2}\right)$$

$$\tilde{\Sigma}_{61}(p,k_1,k_2)=$$

$$i\,\mathrm{e}^2\,\lambda\,\mathrm{Q1}\,(k_1\cdot u)\left(\frac{\left(k_1{}^2-p^2\right)\left(\xi_{V(1)}-1\right)\left(-2\,(k_1\cdot p)-2\,(k_2\cdot p)+p^2+2\,(k_1\cdot k_2)+k_1{}^2\right)}{k_1{}^2.k_2{}^2.k_1{}^2.(k_1-p)^{22}.(k_1+k_2-p)^2}+\frac{2\,(k_2\cdot p)-p^2+2\,(k_1\cdot k_2)+k_1{}^2}{k_1{}^2.k_2{}^2.k_1{}^2.(k_1-p)^2.(k_1+k_2-p)^2}\right)$$

$$\tilde{\Sigma}_{62}(p,k_1,k_2)=8\,\mathrm{e}^4\,\mathrm{Q2}\,\epsilon^{b\,k_1\,k_2\,p}\left(\frac{1}{k_1{}^2.k_2{}^2.k_1{}^2.(k_1-p)^2.(k_1+k_2-p)^2}-\frac{\left(\xi_{V(1)}-1\right)\left(-2\,(k_1\cdot p)+p^2+k_1{}^2-k_2{}^2\right)}{k_1{}^2.k_2{}^2.k_1{}^2.(k_1-p)^2.(k_1+k_2-p)^{22}}\right)$$

$$\tilde{\Sigma}_{63}(p,k_1,k_2)=-\frac{8\,\mathrm{e}^2\,\lambda\,\mathrm{Q2}\,\epsilon^{b\,k_1\,k_2\,p}}{k_1{}^2.k_2{}^2.k_1{}^2.(k_1-p)^2.(k_2-k_1)^2}$$

$$\tilde{\Sigma}_{64}(p,k_1,k_2)=-2\,i\,\mathrm{e}^4\,\mathrm{Q1}\,(k_1\cdot u)$$

$$\Bigg(\left(\xi_{V(1)}-1\right)\Bigg(\left(k_1{}^2-p^2\right)\left(\frac{\left(k_1{}^2-k_2{}^2\right)\left(\xi_{V(1)}-1\right)\left(-k_1\cdot p+k_2\cdot p-k_1\cdot k_2+k_1{}^2\right)}{k_1{}^2.k_2{}^2.k_1{}^2.(k_1-p)^{22}.(k_2-k_1)^{22}}+\frac{-k_1\cdot p-k_2\cdot p+k_1\cdot k_2+k_1{}^2}{k_1{}^2.k_2{}^2.k_1{}^2.(k_1-p)^{22}.(k_2-k_1)^2}\right)+$$

$$\frac{\left(k_1{}^2-k_2{}^2\right)\left(k_1\cdot p-k_2\cdot p-k_1\cdot k_2+k_1{}^2\right)}{k_1{}^2.k_2{}^2.k_1{}^2.(k_1-p)^2.(k_2-k_1)^{22}}\Bigg)+\frac{k_1\cdot p+k_2\cdot p+k_1\cdot k_2+k_1{}^2}{k_1{}^2.k_2{}^2.k_1{}^2.(k_1-p)^2.(k_2-k_1)^2}\Bigg)$$

$$\tilde{\Sigma}_{65}(p,k_1,k_2)=i\,\mathrm{e}^4\,\mathrm{Q1}\Bigg(\left(\xi_{V(1)}-1\right)\Bigg(\left(-2\,(k_1\cdot p)+p^2+k_1{}^2-k_2{}^2\right)(-p\cdot u+k_1\cdot u+k_2\cdot u)$$

$$\left(\frac{\left(\xi_{V(1)}-1\right)\left(k_1{}^2-2\,(k_1\cdot p)\right)^2}{k_2{}^2.\left(k_1{}^2\right)^2.(k_1-p)^{22}.(k_1+k_2-p)^{22}}+\frac{-4\,(k_1\cdot p)+4\,p^2+k_1{}^2}{k_2{}^2.k_1{}^2.(k_1-p)^{22}.(k_1+k_2-p)^{22}}\right)+$$

$$\frac{\left(k_1{}^2-2\,(k_1\cdot p)\right)^2(-p\cdot u+k_1\cdot u-k_2\cdot u)}{k_2{}^2.\left(k_1{}^2\right)^2.(k_1-p)^{22}.(k_1+k_2-p)^2}\Bigg)+\frac{\left(-4\,(k_1\cdot p)+4\,p^2+k_1{}^2\right)(-p\cdot u+k_1\cdot u-k_2\cdot u)}{k_2{}^2.k_1{}^2.(k_1-p)^{22}.(k_1+k_2-p)^2}\Bigg)$$

$$\tilde{\Sigma}_{66}(p,k_1,k_2)=i\,\mathrm{e}^4\,\mathrm{Q1}\Bigg(\left(k_1{}^2-p^2\right)\left(\xi_{V(1)}-1\right)\Bigg(\frac{\left(k_1{}^2-p^2\right)\left(\xi_{V(1)}-1\right)\left(-2\,(k_1\cdot p)-2\,(k_2\cdot p)+p^2+2\,(k_1\cdot k_2)+k_1{}^2\right)(k_1\cdot u-p\cdot u)}{k_2{}^2.k_1{}^2.(k_1-p)^{24}.(k_1+k_2-p)^2}+$$

$$\frac{2\left(-(k_1\cdot p)\,(k_1\cdot u)-(k_1\cdot p)\,(p\cdot u)-2\,(k_2\cdot p)\,(p\cdot u)+p^2\,(p\cdot u)+2\,(k_1\cdot k_2)\,(k_1\cdot u)+k_1{}^2\,(k_1\cdot u)\right)}{k_2{}^2.k_1{}^2.(k_1-p)^{23}.(k_1+k_2-p)^2}\Bigg)+$$

$$\frac{\left(2\,(k_2\cdot p)-p^2+2\,(k_1\cdot k_2)+k_1{}^2\right)(p\cdot u+k_1\cdot u)}{k_2{}^2.k_1{}^2.(k_1-p)^{22}.(k_1+k_2-p)^2}\Bigg)$$

$$\tilde{\Sigma}_{67}(p,k_1,k_2)=i\,\mathrm{e}^4\,\mathrm{Q1}\Bigg(\left(\xi_{V(1)}-1\right)\Bigg(\left(-2\,(k_1\cdot p)+p^2+k_1{}^2-k_2{}^2\right)(-p\cdot u+k_1\cdot u-k_2\cdot u)$$

$$\left(\frac{\left(\xi_{V(1)}-1\right)\left(k_1{}^2-2\,(k_1\cdot p)\right)^2}{k_2{}^2.\left(k_1{}^2\right)^2.(k_1-p)^{22}.(-k_1+k_2+p)^{22}}+\frac{-4\,(k_1\cdot p)+4\,p^2+k_1{}^2}{k_2{}^2.k_1{}^2.(k_1-p)^{22}.(-k_1+k_2+p)^{22}}\right)+$$

$$\frac{\left(k_1{}^2-2\,(k_1\cdot p)\right)^2(-p\cdot u+k_1\cdot u+k_2\cdot u)}{k_2{}^2.\left(k_1{}^2\right)^2.(k_1-p)^{22}.(-k_1+k_2+p)^2}\Bigg)+\frac{\left(-4\,(k_1\cdot p)+4\,p^2+k_1{}^2\right)(-p\cdot u+k_1\cdot u+k_2\cdot u)}{k_2{}^2.k_1{}^2.(k_1-p)^{22}.(-k_1+k_2+p)^2}\Bigg)$$

$$\tilde{\Sigma}_{68}(p,k_1,k_2)=-i\,\mathrm{e}^4\,\mathrm{Q1}\Bigg(\left(k_1{}^2-p^2\right)\left(\xi_{V(1)}-1\right)\Bigg(\frac{\left(k_1{}^2-p^2\right)\left(\xi_{V(1)}-1\right)\left(-2\,(k_1\cdot p)+2\,(k_2\cdot p)+p^2-2\,(k_1\cdot k_2)+k_1{}^2\right)(k_1\cdot u-p\cdot u)}{k_2{}^2.k_1{}^2.(k_1-p)^{24}.(-k_1+k_2+p)^2}+$$

$$\frac{2\left(-(k_1\cdot p)\,(k_1\cdot u)-(k_1\cdot p)\,(p\cdot u)+2\,(k_2\cdot p)\,(p\cdot u)+p^2\,(p\cdot u)-2\,(k_1\cdot k_2)\,(k_1\cdot u)+k_1{}^2\,(k_1\cdot u)\right)}{k_2{}^2.k_1{}^2.(k_1-p)^{23}.(-k_1+k_2+p)^2}\Bigg)+$$

$$\frac{\left(-2\,(k_2\cdot p)-p^2-2\,(k_1\cdot k_2)+k_1{}^2\right)(p\cdot u+k_1\cdot u)}{k_2{}^2.k_1{}^2.(k_1-p)^{22}.(-k_1+k_2+p)^2}\Bigg)$$

$$\tilde{\Sigma}_{69}(p,k_1,k_2)=-i\,e^4\,Q1\Bigg((\xi_{V(1)}-1)\left(k_1{}^2-2\,(k_1\cdot k_2)\right)\Bigg(\frac{(\xi_{V(1)}-1)\left(2\,(k_1\cdot p)+k_1{}^2\right)\left(k_1{}^2-2\,(k_1\cdot k_2)\right)(k_1\cdot u)}{k_2{}^2.\left(k_1{}^2\right)^4.(k_1+p)^2.(k_2-k_1)^2}+$$

$$\frac{2\left(-2\,(k_2\cdot p)(k_1\cdot u)-2\,(k_1\cdot p)(k_2\cdot u)+2\,(k_1\cdot p)(k_1\cdot u)-(k_1\cdot k_2)(k_1\cdot u)+k_1{}^2\,(k_1\cdot u-k_2\cdot u)\right)}{k_2{}^2.\left(k_1{}^2\right)^3.(k_1+p)^2.(k_2-k_1)^2}\Bigg)+$$

$$\frac{\left(2\,(k_1\cdot p)-4\,(k_2\cdot p)-2\,(k_1\cdot k_2)+k_1{}^2\right)(k_1\cdot u-2\,(k_2\cdot u))}{k_2{}^2.\left(k_1{}^2\right)^2.(k_1+p)^2.(k_2-k_1)^2}\Bigg)$$

$$\tilde{\Sigma}_{70}(p,k_1,k_2)=i\,e^4\,Q1\Bigg((\xi_{V(1)}-1)$$

$$\Bigg(\left(k_1{}^2-p^2\right)(p\cdot u+k_1\cdot u)\Bigg(\frac{\left(k_1{}^2-k_2{}^2\right)^2(\xi_{V(1)}-1)}{k_2{}^2.\left(k_1{}^2\right)^2.(k_1+p)^{22}.(k_2-k_1)^{22}}+\frac{2\,(k_1\cdot k_2)+k_1{}^2+k_2{}^2}{k_2{}^2.\left(k_1{}^2\right)^2.(k_1+p)^{22}.(k_2-k_1)^2}\Bigg)+$$

$$\frac{\left(k_1{}^2-k_2{}^2\right)^2(k_1\cdot u-p\cdot u)}{k_2{}^2.\left(k_1{}^2\right)^2.(k_1+p)^2.(k_2-k_1)^{22}}\Bigg)+\frac{\left(2\,(k_1\cdot k_2)+k_1{}^2+k_2{}^2\right)(k_1\cdot u-p\cdot u)}{k_2{}^2.\left(k_1{}^2\right)^2.(k_1+p)^2.(k_2-k_1)^2}\Bigg)$$

$$\tilde{\Sigma}_{71}(p,k_1,k_2)=-i\,e^4\,Q1\Bigg((\xi_{V(1)}-1)\Bigg(\left(k_1{}^2-p^2\right)\left(2\,(k_1\cdot p)-2\,(k_2\cdot p)+p^2-2\,(k_1\cdot k_2)+k_1{}^2\right)$$

$$\Bigg(\frac{\left(k_1{}^2-k_2{}^2\right)(\xi_{V(1)}-1)(k_1\cdot u-k_2\cdot u)}{k_2{}^2.k_1{}^2.(k_1+p)^{22}.(k_1-k_2)^{22}.(-k_1+k_2-p)^2}+\frac{k_1\cdot u+k_2\cdot u}{k_2{}^2.k_1{}^2.(k_1+p)^{22}.(k_1-k_2)^2.(-k_1+k_2-p)^2}\Bigg)+$$

$$\frac{\left(k_1{}^2-k_2{}^2\right)\left(2\,(k_2\cdot p)-p^2-2\,(k_1\cdot k_2)+k_1{}^2\right)(k_1\cdot u-k_2\cdot u)}{k_2{}^2.k_1{}^2.(k_1+p)^2.(k_1-k_2)^{22}.(-k_1+k_2-p)^2}\Bigg)+\frac{\left(2\,(k_2\cdot p)-p^2-2\,(k_1\cdot k_2)+k_1{}^2\right)(k_1\cdot u+k_2\cdot u)}{k_2{}^2.k_1{}^2.(k_1+p)^2.(k_1-k_2)^2.(-k_1+k_2-p)^2}\Bigg)$$

$$\tilde{\Sigma}_{72}(p,k_1,k_2)=\frac{8\,e^2\,\lambda\,Q2\,\epsilon^{b\,k_1\,k_2\,p}}{k_1{}^2.k_2{}^2.k_1{}^2.(k_1-p)^2.(k_1+k_2)^2}$$

$$\tilde{\Sigma}_{73}(p,k_1,k_2)=-2\,i\,e^4\,Q1\,(k_1\cdot u)$$

$$\Bigg((\xi_{V(1)}-1)\Bigg(\left(k_1{}^2-p^2\right)\Bigg(\frac{\left(k_1{}^2-k_2{}^2\right)(\xi_{V(1)}-1)\left(-k_1\cdot p-k_2\cdot p+k_1\cdot k_2+k_1{}^2\right)}{k_1{}^2.k_2{}^2.k_1{}^2.(k_1-p)^{22}.(k_1+k_2)^{22}}+\frac{-k_1\cdot p+k_2\cdot p-k_1\cdot k_2+k_1{}^2}{k_1{}^2.k_2{}^2.k_1{}^2.(k_1-p)^{22}.(k_1+k_2)^2}\Bigg)+$$

$$\frac{\left(k_1{}^2-k_2{}^2\right)\left(k_1\cdot p+k_2\cdot p+k_1\cdot k_2+k_1{}^2\right)}{k_1{}^2.k_2{}^2.k_1{}^2.(k_1-p)^2.(k_1+k_2)^{22}}\Bigg)+\frac{k_1\cdot p-k_2\cdot p-k_1\cdot k_2+k_1{}^2}{k_1{}^2.k_2{}^2.k_1{}^2.(k_1-p)^2.(k_1+k_2)^2}\Bigg)$$

$$\tilde{\Sigma}_{74}(p,k_1,k_2)=-i\,e^2\,\lambda\,Q1\,(k_1\cdot u)\Bigg(\frac{\left(k_1{}^2-p^2\right)(\xi_{V(1)}-1)\left(-2\,(k_1\cdot p)+2\,(k_2\cdot p)+p^2-2\,(k_1\cdot k_2)+k_1{}^2\right)}{k_1{}^2.k_2{}^2.k_1{}^2.(k_1-p)^{22}.(-k_1+k_2+p)^2}+$$

$$\frac{-2\,(k_2\cdot p)-p^2-2\,(k_1\cdot k_2)+k_1{}^2}{k_1{}^2.k_2{}^2.k_1{}^2.(k_1-p)^2.(-k_1+k_2+p)^2}\Bigg)$$

$$\tilde{\Sigma}_{75}(p,k_1,k_2)=8\,e^4\,Q2\,\epsilon^{b\,k_1\,k_2\,p}\Bigg(\frac{1}{k_1{}^2.k_2{}^2.k_1{}^2.(k_1-p)^2.(-k_1+k_2+p)^2}-\frac{(\xi_{V(1)}-1)\left(-2\,(k_1\cdot p)+p^2+k_1{}^2-k_2{}^2\right)}{k_1{}^2.k_2{}^2.k_1{}^2.(k_1-p)^2.(-k_1+k_2+p)^{22}}\Bigg)$$

$$\tilde{\Sigma}_{76}(p,k_1,k_2)=-i\,e^2\,\lambda\,Q1\,(k_1\cdot u)\Bigg(\frac{\left(k_1{}^2-k_2{}^2\right)^2(\xi_{V(1)}-1)}{k_1{}^2.k_2{}^2.\left(k_1{}^2\right)^2.(k_2-k_1)^{22}}+\frac{2\,(k_1\cdot k_2)+k_1{}^2+k_2{}^2}{k_1{}^2.k_2{}^2.\left(k_1{}^2\right)^2.(k_2-k_1)^2}\Bigg)$$

$$\tilde{\Sigma}_{77}(p,k_1,k_2)=i\,e^2\,\lambda\,Q1\,(k_1\cdot u)\Bigg(\frac{\left(k_1{}^2-k_2{}^2\right)^2(\xi_{V(1)}-1)}{k_1{}^2.k_2{}^2.\left(k_1{}^2\right)^2.(k_2-k_1)^{22}}+\frac{2\,(k_1\cdot k_2)+k_1{}^2+k_2{}^2}{k_1{}^2.k_2{}^2.\left(k_1{}^2\right)^2.(k_2-k_1)^2}\Bigg)$$

$$\tilde{\Sigma}_{78}(p,k_1,k_2)=0$$

$$\tilde{\Sigma}_{79}(p, k_1, k_2) = i\, e^2\, \lambda\, \mathrm{Q1}\, (k_1 \cdot u) \left( \frac{(\xi_{V(1)} - 1)\left(k_2{}^2 - 2\,(k_1 \cdot k_2)\right)^2}{k_1{}^2.\left(k_2{}^2\right)^2.k_1{}^2.(\,k_2 - k_1\,)^2.(\,k_1 - k_2\,)^2} + \frac{-4\,(k_1 \cdot k_2) + 4\,k_1{}^2 + k_2{}^2}{k_1{}^2.k_2{}^2.k_1{}^2.(\,k_2 - k_1\,)^2.(\,k_1 - k_2\,)^2} \right)$$

$$\tilde{\Sigma}_{80}(p, k_1, k_2) =$$

$$2\, i\, e^4\, \mathrm{Q1}\, (k_1 \cdot u) \left( \left(k_1{}^2 - k_2{}^2\right)^2 (\xi_{V(1)} - 1) \left( \frac{(\xi_{V(1)} - 1)\left(-2\,(k_1 \cdot k_2) + k_1{}^2 + k_2{}^2\right)}{k_1{}^2.k_2{}^2.k_1{}^2.(\,k_2 - k_1\,)^{22}.(\,k_1 - k_2\,)^{22}} + \frac{1}{k_1{}^2.k_2{}^2.k_1{}^2.(\,k_2 - k_1\,)^2.(\,k_1 - k_2\,)^{22}} + \right.\right.$$

$$\left.\left. \frac{1}{k_1{}^2.k_2{}^2.k_1{}^2.(\,k_2 - k_1\,)^{22}.(\,k_1 - k_2\,)^2} \right) + \frac{2\,(k_1 \cdot k_2) + k_1{}^2 + k_2{}^2}{k_1{}^2.k_2{}^2.k_1{}^2.(\,k_2 - k_1\,)^2.(\,k_1 - k_2\,)^2} \right)$$

$$\tilde{\Sigma}_{81}(p, k_1, k_2) = 0$$

$$\tilde{\Sigma}_{82}(p, k_1, k_2) = i\, e^4\, \mathrm{Q1} \left( (\xi_{V(1)} - 1)\left(k_1{}^2 - 2\,(k_1 \cdot k_2)\right) \left( \frac{(\xi_{V(1)} - 1)\left(k_1{}^2 - 2\,(k_1 \cdot p)\right)\left(k_1{}^2 - 2\,(k_1 \cdot k_2)\right)(k_1 \cdot u)}{k_2{}^2.\left(k_1{}^2\right)^4.(\,k_1 - p\,)^2.(\,k_2 - k_1\,)^2} + \right.\right.$$

$$\left. \frac{2\left(2\,(k_2 \cdot p)\,(k_1 \cdot u) + 2\,(k_1 \cdot p)\,(k_2 \cdot u) - 2\,(k_1 \cdot p)\,(k_1 \cdot u) - (k_1 \cdot k_2)\,(k_1 \cdot u) + k_1{}^2\,(k_1 \cdot u - k_2 \cdot u)\right)}{k_2{}^2.\left(k_1{}^2\right)^3.(\,k_1 - p\,)^2.(\,k_2 - k_1\,)^2} \right) +$$

$$\left. \frac{\left(k_1{}^2 - 2\,(k_1 \cdot p - 2\,(k_2 \cdot p) + k_1 \cdot k_2)\right)(k_1 \cdot u - 2\,(k_2 \cdot u))}{k_2{}^2.\left(k_1{}^2\right)^2.(\,k_1 - p\,)^2.(\,k_2 - k_1\,)^2} \right)$$

$$\tilde{\Sigma}_{83}(p, k_1, k_2) = -i\, e^4\, \mathrm{Q1} \left( (\xi_{V(1)} - 1) \right.$$

$$\left( \left(k_1{}^2 - p^2\right)(k_1 \cdot u - p \cdot u) \left( \frac{\left(k_1{}^2 - k_2{}^2\right)^2 (\xi_{V(1)} - 1)}{k_2{}^2.\left(k_1{}^2\right)^2.(\,k_1 - p\,)^{22}.(\,k_2 - k_1\,)^{22}} + \frac{2\,(k_1 \cdot k_2) + k_1{}^2 + k_2{}^2}{k_2{}^2.\left(k_1{}^2\right)^2.(\,k_1 - p\,)^{22}.(\,k_2 - k_1\,)^2} \right) + \right.$$

$$\left.\left. \frac{\left(k_1{}^2 - k_2{}^2\right)^2 (p \cdot u + k_1 \cdot u)}{k_2{}^2.\left(k_1{}^2\right)^2.(\,k_1 - p\,)^2.(\,k_2 - k_1\,)^{22}} \right) + \frac{\left(2\,(k_1 \cdot k_2) + k_1{}^2 + k_2{}^2\right)(p \cdot u + k_1 \cdot u)}{k_2{}^2.\left(k_1{}^2\right)^2.(\,k_1 - p\,)^2.(\,k_2 - k_1\,)^2} \right)$$

$$\tilde{\Sigma}_{84}(p, k_1, k_2) = i\, e^4\, \mathrm{Q1} \left( (\xi_{V(1)} - 1) \left( \left(k_1{}^2 - p^2\right)\left(-2\,(k_1 \cdot p) + 2\,(k_2 \cdot p) + p^2 - 2\,(k_1 \cdot k_2) + k_1{}^2\right) \right.\right.$$

$$\left( \frac{\left(k_1{}^2 - k_2{}^2\right)(\xi_{V(1)} - 1)\,(k_1 \cdot u - k_2 \cdot u)}{k_2{}^2.k_1{}^2.(\,k_1 - p\,)^{22}.(\,k_1 - k_2\,)^{22}.(\,-k_1 + k_2 + p\,)^2} + \frac{k_1 \cdot u + k_2 \cdot u}{k_2{}^2.k_1{}^2.(\,k_1 - p\,)^{22}.(\,k_1 - k_2\,)^2.(\,-k_1 + k_2 + p\,)^2} \right) +$$

$$\left.\left. \frac{\left(k_1{}^2 - k_2{}^2\right)\left(-2\,(k_2 \cdot p) - p^2 - 2\,(k_1 \cdot k_2) + k_1{}^2\right)(k_1 \cdot u - k_2 \cdot u)}{k_2{}^2.k_1{}^2.(\,k_1 - p\,)^2.(\,k_1 - k_2\,)^{22}.(\,-k_1 + k_2 + p\,)^2} \right) + \frac{\left(-2\,(k_2 \cdot p) - p^2 - 2\,(k_1 \cdot k_2) + k_1{}^2\right)(k_1 \cdot u + k_2 \cdot u)}{k_2{}^2.k_1{}^2.(\,k_1 - p\,)^2.(\,k_1 - k_2\,)^2.(\,-k_1 + k_2 + p\,)^2} \right)$$

$$\tilde{\Sigma}_{85}(p, k_1, k_2) = i\, e^4\, \mathrm{Q1}\, (k_2 \cdot u) \left( (\xi_{V(1)} - 1) \left( \left(k_1{}^2 - p^2\right)\left(2\,(k_1 \cdot p) + 2\,(k_2 \cdot p) + p^2 + 2\,(k_1 \cdot k_2) + k_1{}^2\right) \right.\right.$$

$$\left( \frac{\left(k_1{}^2 - k_2{}^2\right)(\xi_{V(1)} - 1)\left(2\,(k_1 \cdot p) + 2\,(k_2 \cdot p) + 2\,(k_1 \cdot k_2) + k_1{}^2 + k_2{}^2\right)}{\left(k_2{}^2\right)^2.k_1{}^2.(\,k_1 + p\,)^{22}.(\,k_1 + k_2\,)^{22}.(\,k_1 + k_2 + p\,)^2} + \right.$$

$$\left. \frac{2\,(k_1 \cdot p) - 2\,(k_2 \cdot p) + k_1{}^2 - k_2{}^2}{\left(k_2{}^2\right)^2.k_1{}^2.(\,k_1 + p\,)^{22}.(\,k_1 + k_2\,)^2.(\,k_1 + k_2 + p\,)^2} \right) +$$

$$\left. \frac{\left(k_1{}^2 - k_2{}^2\right)\left(2\,(k_1 \cdot p) + 2\,(k_2 \cdot p) + 2\,(k_1 \cdot k_2) + k_1{}^2 + k_2{}^2\right)\left(-2\,(k_2 \cdot p) - p^2 + 2\,(k_1 \cdot k_2) + k_1{}^2\right)}{\left(k_2{}^2\right)^2.k_1{}^2.(\,k_1 + p\,)^2.(\,k_1 + k_2\,)^{22}.(\,k_1 + k_2 + p\,)^2} \right) +$$

$$\left. \frac{\left(2\,(k_1 \cdot p) - 2\,(k_2 \cdot p) + k_1{}^2 - k_2{}^2\right)\left(-2\,(k_2 \cdot p) - p^2 + 2\,(k_1 \cdot k_2) + k_1{}^2\right)}{\left(k_2{}^2\right)^2.k_1{}^2.(\,k_1 + p\,)^2.(\,k_1 + k_2\,)^2.(\,k_1 + k_2 + p\,)^2} \right)$$

$$\tilde{\Sigma}_{86}(p, k_1, k_2) = i\, e^4\, \mathrm{Q1}\, (k_1 \cdot u) \left( \left(k_1{}^2 - p^2\right)(\xi_{V(1)} - 1)\left(-2\,(k_1 \cdot p) + 2\,(k_2 \cdot p) + p^2 - 2\,(k_1 \cdot k_2) + k_1{}^2\right) \right.$$

$$\left(\frac{\left(k_1^2-p^2\right)(\xi_{V(1)}-1)\left(-2(k_1\cdot p)+2(k_2\cdot p)+p^2-2(k_1\cdot k_2)+k_1^2\right)}{k_1^2.k_2^2.k_1^2.(k_1-p)^{24}.(-k_1+k_2+p)^2}+\frac{2\left(-2(k_2\cdot p)-p^2-2(k_1\cdot k_2)+k_1^2\right)}{k_1^2.k_2^2.k_1^2.(k_1-p)^{23}.(-k_1+k_2+p)^2}\right)+$$

$$\left.\frac{\left(2(k_2\cdot p)+p^2+2(k_1\cdot k_2)-k_1^2\right)^2}{k_1^2.k_2^2.k_1^2.(k_1-p)^{22}.(-k_1+k_2+p)^2}\right)$$

$$\tilde{\Sigma}_{87}(p,k_1,k_2)=0$$

$$\tilde{\Sigma}_{88}(p,k_1,k_2)=$$

$$i\,e^4\,Q1\,(k_1\cdot u)\left((\xi_{V(1)}-1)\left(\left(k_1^2-p^2\right)^2\left(\frac{\left(k_1^2-k_2^2\right)^2(\xi_{V(1)}-1)}{\left(k_1^2\right)^2.k_2^2.k_1^2.(k_1-p)^{22}.(k_1+k_2)^{22}}+\frac{-2(k_1\cdot k_2)+k_1^2+k_2^2}{\left(k_1^2\right)^2.k_2^2.k_1^2.(k_1-p)^{22}.(k_1+k_2)^2}\right)+\right.\right.$$

$$\left.\left.\frac{\left(k_1^2-k_2^2\right)^2\left(2(k_1\cdot p)+p^2+k_1^2\right)}{\left(k_1^2\right)^2.k_2^2.k_1^2.(k_1-p)^2.(k_1+k_2)^{22}}\right)+\frac{\left(2(k_1\cdot p)+p^2+k_1^2\right)\left(-2(k_1\cdot k_2)+k_1^2+k_2^2\right)}{\left(k_1^2\right)^2.k_2^2.k_1^2.(k_1-p)^2.(k_1+k_2)^2}\right)$$

$$\tilde{\Sigma}_{89}(p,k_1,k_2)=8\,e^4\,Q2\,\epsilon^{b\,k_1\,k_2\,p}\left(\frac{(\xi_{V(1)}-1)\left(k_1^2-2(k_1\cdot p)\right)\left(2(k_1\cdot k_2)+k_1^2\right)}{\left(k_1^2\right)^3.k_2^2.k_1^2.(k_1-p)^2.(k_1+k_2)^2}+\frac{-2(k_1\cdot p)-4(k_2\cdot p)+2(k_1\cdot k_2)+k_1^2}{\left(k_1^2\right)^2.k_2^2.k_1^2.(k_1-p)^2.(k_1+k_2)^2}\right)$$

$$\tilde{\Sigma}_{90}(p,k_1,k_2)=-i\,e^4\,Q1\,(k_1\cdot u-p\cdot u)$$

$$\left((\xi_{V(1)}-1)\left(\left(-2(k_1\cdot p)+p^2+k_1^2-k_2^2\right)^2\left(\frac{(\xi_{V(1)}-1)\left(k_1^2-2(k_1\cdot p)\right)^2}{k_2^2.\left(k_1^2\right)^2.(k_1-p)^{23}.(-k_1+k_2+p)^{22}}+\frac{-4(k_1\cdot p)+4p^2+k_1^2}{k_2^2.k_1^2.(k_1-p)^{23}.(-k_1+k_2+p)^{22}}\right)+\right.\right.$$

$$\left.\frac{\left(k_1^2-2(k_1\cdot p)\right)^2\left(-2(k_1\cdot p)-2(k_2\cdot p)+p^2+2(k_1\cdot k_2)+k_1^2+k_2^2\right)}{k_2^2.\left(k_1^2\right)^2.(k_1-p)^{23}.(-k_1+k_2+p)^2}\right)+$$

$$\left.\frac{\left(-4(k_1\cdot p)+4p^2+k_1^2\right)\left(-2(k_1\cdot p)-2(k_2\cdot p)+p^2+2(k_1\cdot k_2)+k_1^2+k_2^2\right)}{k_2^2.k_1^2.(k_1-p)^{23}.(-k_1+k_2+p)^2}\right)$$

$$\tilde{\Sigma}_{91}(p,k_1,k_2)=8\,e^4\,Q2\,\epsilon^{b\,k_1\,k_2\,p}\left(\frac{\left(k_1^2-p^2\right)(\xi_{V(1)}-1)\left(-2(k_1\cdot p)+2(k_2\cdot p)+p^2-2(k_1\cdot k_2)+k_1^2\right)}{k_2^2.k_1^2.(k_1-p)^{24}.(-k_1+k_2+p)^2}+\right.$$

$$\left.\frac{-2(k_2\cdot p)-p^2-2(k_1\cdot k_2)+k_1^2}{k_2^2.k_1^2.(k_1-p)^{23}.(-k_1+k_2+p)^2}\right)$$

$$\tilde{\Sigma}_{92}(p,k_1,k_2)=2\,i\,e^4\,Q1\left((\xi_{V(1)}-1)\left((p\cdot u+k_2\cdot u)\left(\frac{\left(k_1^2-p^2\right)(\xi_{V(1)}-1)\left(k_1\cdot p-k_2\cdot p-p^2+k_1\cdot k_2\right)}{k_2^2.k_1^2.(k_2+p)^{22}.(k_1-p)^{22}}+\right.\right.\right.$$

$$\left.\left.\left.\frac{k_1\cdot p+k_2\cdot p+p^2+k_1\cdot k_2}{k_2^2.k_1^2.(k_2+p)^{22}.(k_1-p)^2}\right)+\frac{\left(k_1^2-p^2\right)(k_1\cdot u-p\cdot u)}{k_1^2.k_2^2.(k_1-p)^{22}.(k_2+p)^2}\right)+\frac{p\cdot u+k_1\cdot u}{k_2^2.k_1^2.(k_2+p)^2.(k_1-p)^2}\right)$$

$$\tilde{\Sigma}_{93}(p,k_1,k_2)=-\frac{i\,\lambda^2\,Q1\,(k_1\cdot u)}{\left(k_2^2\right)^2.\left(k_1^2\right)^2}$$

$$\tilde{\Sigma}_{94}(p,k_1,k_2)=-2\,i\,e^4\,Q1\,(k_1\cdot u)\left(\frac{D}{\left(k_2^2\right)^2.\left(k_1^2\right)^2}+k_2^2(\xi_{V(1)}-1)\left(\frac{k_2^2(\xi_{V(1)}-1)}{\left(k_2^2\right)^4.\left(k_1^2\right)^2}+\frac{2}{\left(k_2^2\right)^3.\left(k_1^2\right)^2}\right)\right)$$

$$\tilde{\Sigma}_{95}(p,k_1,k_2)=0$$

$$\tilde{\Sigma}_{96}(p,k_1,k_2)=$$

$$-2\,i\,e^4\,Q1\left((\xi_{V(1)}-1)\left((k_2\cdot u-p\cdot u)\left(\frac{\left(k_1^2-p^2\right)(\xi_{V(1)}-1)\left(-k_1\cdot p+k_2\cdot p-p^2+k_1\cdot k_2\right)}{k_2^2.k_1^2.(k_2-p)^{22}.(k_1+p)^{22}}+\frac{-k_1\cdot p-k_2\cdot p+p^2+k_1\cdot k_2}{k_2^2.k_1^2.(k_2-p)^{22}.(k_1+p)^2}\right)+\right.\right.$$

$$\left.\left.\frac{\left(k_1^2-p^2\right)(p\cdot u+k_1\cdot u)}{k_1^2.k_2^2.(k_1+p)^{22}.(k_2-p)^2}\right)+\frac{k_1\cdot u-p\cdot u}{k_2^2.k_1^2.(k_2-p)^2.(k_1+p)^2}\right)$$

We simplify the integrals into a set of fundamental ones by employing the TARCER Mathematica package.

Our results are as follows :

$$(4\,\pi)^D\,\Sigma_1(p) = -\frac{i\,e^2\,\lambda\,Q1\left(\left(3\,D^2 - 20\,D + 32\right)\xi_{V(1)} - D^2 + 3\,D - 2\right)(p\cdot u)\,\mathbf{J}^{(D)}_{\{1,0\}\{1,0\}\{1,0\}}}{(D-6)\,(D-4)\,p^2}$$

$$(4\,\pi)^D\,\Sigma_2(p) = -\frac{i\,e^2\,\lambda\,Q1\left(\left(3\,D^2 - 20\,D + 32\right)\xi_{V(1)} - D^2 + 3\,D - 2\right)(p\cdot u)\,\mathbf{J}^{(D)}_{\{1,0\}\{1,0\}\{1,0\}}}{(D-6)\,(D-4)\,p^2}$$

$$(4\,\pi)^D\,\Sigma_3(p) = \frac{1}{(D-6)\,(D-4)\,p^2}\,i\,e^4\,Q1\left(2\,D^5 - 27\,D^4 + 136\,D^3 - 313\,D^2 + \left(2\,D^5 - 36\,D^4 + 257\,D^3 - 914\,D^2 + 1626\,D - 1160\right)\xi^2_{V(1)} + \left(-4\,D^5 + 63\,D^4 - 384\,D^3 + 1118\,D^2 - 1515\,D + 722\right)\xi_{V(1)} + 322\,D - 120\right)(p\cdot u)\,\mathbf{J}^{(D)}_{\{1,0\}\{1,0\}\{1,0\}}$$

$$(4\,\pi)^D\,\Sigma_4(p) = 0$$

$$(4\,\pi)^D\,\Sigma_5(p) = \frac{1}{2\,(D-6)\,(D-4)^2\,p^2}\,i\,e^4\,Q1\,(p\cdot u)\left(\left(D^2 - 10\,D + 24\right)p^2\left(D^3 - 7\,D^2 + \left(-2\,D^3 + 18\,D^2 - 55\,D + 58\right)\xi_{V(1)} + (D-4)^2\,(D-3)\,\xi^2_{V(1)} + 18\,D - 16\right)\left(\mathbf{B}^{(D)}_{\{1,0\}\{1,0\}}\right)^2 - 2\left(2\,(D-4)^2\left(2\,D^3 - 22\,D^2 + 80\,D - 95\right)\xi^2_{V(1)} + \left(-8\,D^5 + 132\,D^4 - 839\,D^3 + 2567\,D^2 - 3766\,D + 2104\right)\xi_{V(1)} + 4\left(D^5 - 14\,D^4 + 72\,D^3 - 173\,D^2 + 200\,D - 96\right)\right)\mathbf{J}^{(D)}_{\{1,0\}\{1,0\}\{1,0\}}\right)$$

$$(4\,\pi)^D\,\Sigma_6(p) = \frac{1}{2\,(D-6)\,(D-4)^2\,p^2}\,i\,e^4\,Q1\,(p\cdot u)\left(\left(D^2 - 10\,D + 24\right)p^2\left(D^3 - 7\,D^2 + \left(-2\,D^3 + 18\,D^2 - 55\,D + 58\right)\xi_{V(1)} + (D-4)^2\,(D-3)\,\xi^2_{V(1)} + 18\,D - 16\right)\left(\mathbf{B}^{(D)}_{\{1,0\}\{1,0\}}\right)^2 - 2\left(2\,(D-4)^2\left(2\,D^3 - 22\,D^2 + 80\,D - 95\right)\xi^2_{V(1)} + \left(-8\,D^5 + 132\,D^4 - 839\,D^3 + 2567\,D^2 - 3766\,D + 2104\right)\xi_{V(1)} + 4\left(D^5 - 14\,D^4 + 72\,D^3 - 173\,D^2 + 200\,D - 96\right)\right)\mathbf{J}^{(D)}_{\{1,0\}\{1,0\}\{1,0\}}\right)$$

$$(4\,\pi)^D\,\Sigma_7(p) = -\frac{i\,e^2\,\lambda\,Q1\left(\left(3\,D^2 - 20\,D + 32\right)\xi_{V(1)} - D^2 + 3\,D - 2\right)(p\cdot u)\,\mathbf{J}^{(D)}_{\{1,0\}\{1,0\}\{1,0\}}}{(D-6)\,(D-4)\,p^2}$$

$$(4\,\pi)^D\,\Sigma_8(p) = -\frac{i\,e^2\,\lambda\,Q1\left(\left(3\,D^2 - 20\,D + 32\right)\xi_{V(1)} - D^2 + 3\,D - 2\right)(p\cdot u)\,\mathbf{J}^{(D)}_{\{1,0\}\{1,0\}\{1,0\}}}{(D-6)\,(D-4)\,p^2}$$

$$(4\,\pi)^D\,\Sigma_9(p) = \frac{1}{(D-6)\,(D-4)\,p^2}\,i\,e^4\,Q1\left(2\,D^5 - 27\,D^4 + 136\,D^3 - 313\,D^2 + \left(2\,D^5 - 36\,D^4 + 257\,D^3 - 914\,D^2 + 1626\,D - 1160\right)\xi^2_{V(1)} + \left(-4\,D^5 + 63\,D^4 - 384\,D^3 + 1118\,D^2 - 1515\,D + 722\right)\xi_{V(1)} + 322\,D - 120\right)(p\cdot u)\,\mathbf{J}^{(D)}_{\{1,0\}\{1,0\}\{1,0\}}$$

$$(4\,\pi)^D\,\Sigma_{10}(p) = 0$$

$$(4\,\pi)^D\,\Sigma_{11}(p) = \frac{1}{4\,(D-6)\,(D-4)^2\,p^2}\,i\,e^4\,Q1\,(p\cdot u)\left(\left(D^2 - 10\,D + 24\right)p^2\left((D-4)^2\left(D^2 - 6\,D + 7\right)\xi^2_{V(1)} + \left(D^2 - 8\,D + 11\right)(D-2)^2 + \left(-2\,D^4 + 26\,D^3 - 117\,D^2 + 217\,D - 140\right)\xi_{V(1)}\right)\left(\mathbf{B}^{(D)}_{\{1,0\}\{1,0\}}\right)^2 + 4\left(\left(8\,D^5 - 146\,D^4 + 1055\,D^3 - 3778\,D^2 + 6712\,D - 4736\right)\xi^2_{V(1)} + \left(-16\,D^5 + 252\,D^4 - 1525\,D^3 + 4403\,D^2 - 5970\,D + 2936\right)\xi_{V(1)} + 2\left(4\,D^5 - 53\,D^4 + 259\,D^3 - 582\,D^2 + 602\,D - 240\right)\right)\mathbf{J}^{(D)}_{\{1,0\}\{1,0\}\{1,0\}}\right)$$

$$(4\,\pi)^D\,\Sigma_{12}(p) = 0$$

$$(4\,\pi)^D\,\Sigma_{13}(p) = \frac{1}{4\,(D-6)\,(D-4)^2\,p^2}\,i\,e^4\,Q1\,(p\cdot u)\left(\left(D^2 - 10\,D + 24\right)p^2\left((D-4)^2\left(D^2 - 6\,D + 7\right)\xi^2_{V(1)} + \left(D^2 - 8\,D + 11\right)(D-2)^2 + \left(-2\,D^4 + 26\,D^3 - 117\,D^2 + 217\,D - 140\right)\xi_{V(1)}\right)\left(\mathbf{B}^{(D)}_{\{1,0\}\{1,0\}}\right)^2 + 4\left(\left(8\,D^5 - 146\,D^4 + 1055\,D^3 - 3778\,D^2 + 6712\,D - 4736\right)\xi^2_{V(1)} + \left(-16\,D^5 + 252\,D^4 - 1525\,D^3 + 4403\,D^2 - 5970\,D + 2936\right)\xi_{V(1)} + 2\left(4\,D^5 - 53\,D^4 + 259\,D^3 - 582\,D^2 + 602\,D - 240\right)\right)\mathbf{J}^{(D)}_{\{1,0\}\{1,0\}\{1,0\}}\right)$$

$$(4\,\pi)^D\,\Sigma_{14}(p) = 0$$

$$(4\,\pi)^D\,\Sigma_{15}(p) = -\frac{2\,i\,(D-2)\,e^4\,Q1\left(2\left(D^2 - 6\,D + 8\right) + (8 - 3\,D)\,\xi_{V(1)}\right)(p\cdot u)\,\mathbf{J}^{(D)}_{\{1,0\}\{1,0\}\{1,0\}}}{(D-8)\,(D-6)\,(D-4)\,p^2}$$

$$(4\,\pi)^D\,\Sigma_{16}(p) = \frac{2\,i\,(D-2)\,e^4\,Q1\left(2\left(D^2 - 6\,D + 8\right) + (8 - 3\,D)\,\xi_{V(1)}\right)(p\cdot u)\,\mathbf{J}^{(D)}_{\{1,0\}\{1,0\}\{1,0\}}}{(D-8)\,(D-6)\,(D-4)\,p^2}$$

$$(4\,\pi)^D\,\Sigma_{17}(p) =$$

$$-\frac{1}{(D-6)(D-4)\,p^2} 2\,i\,\mathrm{e}^4\,\mathrm{Q1}\left(2\,(D-3)\left(D^2-5\,D+4\right)^2+\left(2\,D^5-34\,D^4+235\,D^3-823\,D^2+1456\,D-1036\right)\xi_{V(1)}^2+\right.$$
$$\left.\left(-4\,D^5+60\,D^4-353\,D^3+1003\,D^2-1338\,D+632\right)\xi_{V(1)}\right)(p\cdot u)\,\mathbf{J}^{(D)}_{\{1,0\}\{1,0\}\{1,0\}}$$

$$(4\,\pi)^D\,\Sigma_{18}(p)=0$$

$$(4\,\pi)^D\,\Sigma_{19}(p)=\frac{2\,i\,\mathrm{e}^2\,\lambda\,\mathrm{Q1}\left(\left(3\,D^2-20\,D+32\right)\xi_{V(1)}-D^2+3\,D-2\right)(p\cdot u)\,\mathbf{J}^{(D)}_{\{1,0\}\{1,0\}\{1,0\}}}{(D-6)(D-4)\,p^2}$$

$$(4\,\pi)^D\,\Sigma_{20}(p)=\frac{1}{(D-6)(D-4)\,p^2} i\,\mathrm{e}^4\,\mathrm{Q1}\left(2\,D^4-21\,D^3+72\,D^2+2\left(D^4-14\,D^3+75\,D^2-181\,D+164\right)\xi_{V(1)}^2+\right.$$
$$\left.\left(-4\,D^4+49\,D^3-212\,D^2+369\,D-202\right)\xi_{V(1)}-95\,D+42\right)(p\cdot u)\,\mathbf{J}^{(D)}_{\{1,0\}\{1,0\}\{1,0\}}$$

$$(4\,\pi)^D\,\Sigma_{21}(p)=0$$
$$(4\,\pi)^D\,\Sigma_{22}(p)=0$$
$$(4\,\pi)^D\,\Sigma_{23}(p)=0$$

$$(4\,\pi)^D\,\Sigma_{24}(p)=-\frac{i\,(D-3)\,\lambda^2\,\mathrm{Q1}\,(p\cdot u)\,\mathbf{J}^{(D)}_{\{1,0\}\{1,0\}\{1,0\}}}{p^2}$$

$$(4\,\pi)^D\,\Sigma_{25}(p)=\frac{i\,(D-3)\,\lambda^2\,\mathrm{Q1}\,(p\cdot u)\,\mathbf{J}^{(D)}_{\{1,0\}\{1,0\}\{1,0\}}}{2\,p^2}$$

$$(4\,\pi)^D\,\Sigma_{26}(p)=-\frac{i\,(D-3)\,\mathrm{e}^4\,\mathrm{Q1}\left(\left(D^2-5\,D+8\right)\xi_{V(1)}^2-2\left(D^2-5\,D+4\right)\xi_{V(1)}+(D-1)\,D\right)(p\cdot u)\,\mathbf{J}^{(D)}_{\{1,0\}\{1,0\}\{1,0\}}}{2\,p^2}$$

$$(4\,\pi)^D\,\Sigma_{27}(p)=0$$

$$(4\,\pi)^D\,\Sigma_{28}(p)=\frac{2\,i\,\mathrm{e}^2\,\lambda\,\mathrm{Q1}\left(\left(3\,D^2-20\,D+32\right)\xi_{V(1)}-D^2+3\,D-2\right)(p\cdot u)\,\mathbf{J}^{(D)}_{\{1,0\}\{1,0\}\{1,0\}}}{(D-6)(D-4)\,p^2}$$

$$(4\,\pi)^D\,\Sigma_{29}(p)=\frac{1}{(D-6)(D-4)\,p^2} i\,\mathrm{e}^4\,\mathrm{Q1}\left(2\,D^4-21\,D^3+72\,D^2+2\left(D^4-14\,D^3+75\,D^2-181\,D+164\right)\xi_{V(1)}^2+\right.$$
$$\left.\left(-4\,D^4+49\,D^3-212\,D^2+369\,D-202\right)\xi_{V(1)}-95\,D+42\right)(p\cdot u)\,\mathbf{J}^{(D)}_{\{1,0\}\{1,0\}\{1,0\}}$$

$$(4\,\pi)^D\,\Sigma_{30}(p)=0$$

$$(4\,\pi)^D\,\Sigma_{31}(p)=\frac{i\,(D-3)\,\mathrm{e}^4\,\mathrm{Q1}\left(\left(D^2-7\,D+12\right)\xi_{V(1)}^2+\left(-2\,D^2+9\,D-7\right)\xi_{V(1)}+(D-1)^2\right)(p\cdot u)\,\mathbf{J}^{(D)}_{\{1,0\}\{1,0\}\{1,0\}}}{(D-4)\,p^2}$$

$$(4\,\pi)^D\,\Sigma_{32}(p)=0$$
$$(4\,\pi)^D\,\Sigma_{33}(p)=0$$
$$(4\,\pi)^D\,\Sigma_{34}(p)=0$$
$$(4\,\pi)^D\,\Sigma_{35}(p)=0$$
$$(4\,\pi)^D\,\Sigma_{36}(p)=0$$
$$(4\,\pi)^D\,\Sigma_{37}(p)=0$$
$$(4\,\pi)^D\,\Sigma_{38}(p)=0$$
$$(4\,\pi)^D\,\Sigma_{39}(p)=0$$
$$(4\,\pi)^D\,\Sigma_{40}(p)=0$$
$$(4\,\pi)^D\,\Sigma_{41}(p)=0$$
$$(4\,\pi)^D\,\Sigma_{42}(p)=0$$
$$(4\,\pi)^D\,\Sigma_{43}(p)=0$$

$$(4\,\pi)^D\,\Sigma_{44}(p)=\frac{i\,(D-3)\,\mathrm{e}^4\,\mathrm{Q1}\left(\left(D^2-7\,D+12\right)\xi_{V(1)}^2+\left(-2\,D^2+9\,D-7\right)\xi_{V(1)}+(D-1)^2\right)(p\cdot u)\,\mathbf{J}^{(D)}_{\{1,0\}\{1,0\}\{1,0\}}}{(D-4)\,p^2}$$

$$(4\,\pi)^D\,\Sigma_{45}(p)=0$$
$$(4\,\pi)^D\,\Sigma_{46}(p)=0$$
$$(4\,\pi)^D\,\Sigma_{47}(p)=0$$
$$(4\,\pi)^D\,\Sigma_{48}(p)=0$$
$$(4\,\pi)^D\,\Sigma_{49}(p)=0$$
$$(4\,\pi)^D\,\Sigma_{50}(p)=0$$
$$(4\,\pi)^D\,\Sigma_{51}(p)=$$

$$\frac{1}{4} i\, e^4\, Q1 \left(\left(D^3 - 12 D^2 + 49 D - 68\right) \xi_{V(1)}^2 + \left(-2 D^3 + 18 D^2 - 49 D + 33\right) \xi_{V(1)} + (D-4)(D-1)^2\right)(p \cdot u)\left(\mathbf{B}^{(D)}_{\{1,0\}\{1,0\}}\right)^2$$

$$(4\pi)^D\, \Sigma_{52}(p) = 0$$
$$(4\pi)^D\, \Sigma_{53}(p) = 0$$
$$(4\pi)^D\, \Sigma_{54}(p) = 0$$
$$(4\pi)^D\, \Sigma_{55}(p) = 0$$
$$(4\pi)^D\, \Sigma_{56}(p) = 0$$
$$(4\pi)^D\, \Sigma_{57}(p) = 0$$
$$(4\pi)^D\, \Sigma_{58}(p) = 0$$

$$(4\pi)^D\, \Sigma_{59}(p) = \frac{1}{4} i\, e^4\, Q1 \left(\left(D^3 - 12 D^2 + 49 D - 68\right) \xi_{V(1)}^2 + \left(-2 D^3 + 18 D^2 - 49 D + 33\right) \xi_{V(1)} + (D-4)(D-1)^2\right)(p \cdot u)\left(\mathbf{B}^{(D)}_{\{1,0\}\{1,0\}}\right)^2$$

$$(4\pi)^D\, \Sigma_{60}(p) = 0$$
$$(4\pi)^D\, \Sigma_{61}(p) = 0$$
$$(4\pi)^D\, \Sigma_{62}(p) = 0$$
$$(4\pi)^D\, \Sigma_{63}(p) = 0$$

$$(4\pi)^D\, \Sigma_{64}(p) = -\frac{1}{(D-6)(D-4)\, p^2} i\, e^4\, Q1 \left(4\left(D^2 - 7 D + 12\right)(D-1)^2 + \left(4 D^4 - 54 D^3 + 275 D^2 - 626 D + 536\right) \xi_{V(1)}^2 + \left(-8 D^4 + 90 D^3 - 365 D^2 + 609 D - 326\right) \xi_{V(1)}\right)(p \cdot u)\, \mathbf{J}^{(D)}_{\{1,0\}\{1,0\}\{1,0\}}$$

$$(4\pi)^D\, \Sigma_{65}(p) = -\frac{1}{(D-6)(D-4)\, p^2} 2\, i\, e^4\, Q1 \left(2\left(D^2 - 7 D + 12\right)(D-1)^2 + \left(2 D^4 - 28 D^3 + 147 D^2 - 342 D + 296\right) \xi_{V(1)}^2 + \left(-4 D^4 + 46 D^3 - 189 D^2 + 317 D - 170\right) \xi_{V(1)}\right)(p \cdot u)\, \mathbf{J}^{(D)}_{\{1,0\}\{1,0\}\{1,0\}}$$

$$(4\pi)^D\, \Sigma_{66}(p) = 0$$

$$(4\pi)^D\, \Sigma_{67}(p) = -\frac{1}{(D-6)(D-4)\, p^2} 2\, i\, e^4\, Q1 \left(2\left(D^2 - 7 D + 12\right)(D-1)^2 + \left(2 D^4 - 28 D^3 + 147 D^2 - 342 D + 296\right) \xi_{V(1)}^2 + \left(-4 D^4 + 46 D^3 - 189 D^2 + 317 D - 170\right) \xi_{V(1)}\right)(p \cdot u)\, \mathbf{J}^{(D)}_{\{1,0\}\{1,0\}\{1,0\}}$$

$$(4\pi)^D\, \Sigma_{68}(p) = 0$$

$$(4\pi)^D\, \Sigma_{69}(p) = -\frac{2\, i\, (D-2)\, e^4\, Q1\, (p \cdot u)\, \mathbf{J}^{(D)}_{\{1,0\}\{1,0\}\{1,0\}}}{(D-6)(D-4)\, p^2}$$

$$(4\pi)^D\, \Sigma_{70}(p) = -\frac{i\, e^4\, Q1 \left(\left(2 D^3 - 19 D^2 + 59 D - 60\right) \xi_{V(1)}^2 + \left(-4 D^3 + 29 D^2 - 63 D + 38\right) \xi_{V(1)} + 2(D-3)(D-1)^2\right)(p \cdot u)\, \mathbf{J}^{(D)}_{\{1,0\}\{1,0\}\{1,0\}}}{(D-4)\, p^2}$$

$$(4\pi)^D\, \Sigma_{71}(p) = \frac{1}{4(D-4)^2\, p^2} i\, e^4\, Q1\, (p \cdot u) \Big((D-4)\, p^2 \left(D^3 - 6 D^2 + \left(-2 D^3 + 15 D^2 - 33 D + 20\right) \xi_{V(1)} + (D-4)^2 (D-1)\, \xi_{V(1)}^2 + 11 D - 8\right)\left(\mathbf{B}^{(D)}_{\{1,0\}\{1,0\}}\right)^2 - 4(D-3)\left(2 D^3 - 11 D^2 + \left(-4 D^3 + 33 D^2 - 81 D + 52\right) \xi_{V(1)} + 2(D-4)^2 (D-3)\, \xi_{V(1)}^2 + 16 D - 8\right) \mathbf{J}^{(D)}_{\{1,0\}\{1,0\}\{1,0\}}\Big)$$

$$(4\pi)^D\, \Sigma_{72}(p) = 0$$

$$(4\pi)^D\, \Sigma_{73}(p) = -\frac{1}{(D-6)(D-4)\, p^2} i\, e^4\, Q1 \left(4\left(D^2 - 7 D + 12\right)(D-1)^2 + \left(4 D^4 - 54 D^3 + 275 D^2 - 626 D + 536\right) \xi_{V(1)}^2 + \left(-8 D^4 + 90 D^3 - 365 D^2 + 609 D - 326\right) \xi_{V(1)}\right)(p \cdot u)\, \mathbf{J}^{(D)}_{\{1,0\}\{1,0\}\{1,0\}}$$

$$(4\pi)^D\, \Sigma_{74}(p) = 0$$
$$(4\pi)^D\, \Sigma_{75}(p) = 0$$
$$(4\pi)^D\, \Sigma_{76}(p) = 0$$
$$(4\pi)^D\, \Sigma_{77}(p) = 0$$
$$(4\pi)^D\, \Sigma_{78}(p) = 0$$
$$(4\pi)^D\, \Sigma_{79}(p) = 0$$
$$(4\pi)^D\, \Sigma_{80}(p) = 0$$
$$(4\pi)^D\, \Sigma_{81}(p) = 0$$

$$(4\,\pi)^D\,\Sigma_{82}(p) = -\frac{2\,i\,(D-2)\,\mathrm{e}^4\,\mathrm{Q1}\,(p\cdot u)\,\mathbf{J}^{(D)}_{\{1,0\}\,\{1,0\}\,\{1,0\}}}{(D-6)\,(D-4)\,p^2}$$

$$(4\,\pi)^D\,\Sigma_{83}(p) =$$
$$-\frac{i\,\mathrm{e}^4\,\mathrm{Q1}\,\left(\left(2\,D^3-19\,D^2+59\,D-60\right)\xi^2_{V(1)}+\left(-4\,D^3+29\,D^2-63\,D+38\right)\xi_{V(1)}+2\,(D-3)\,(D-1)^2\right)(p\cdot u)\,\mathbf{J}^{(D)}_{\{1,0\}\,\{1,0\}\,\{1,0\}}}{(D-4)\,p^2}$$

$$(4\,\pi)^D\,\Sigma_{84}(p) = \frac{1}{4\,(D-4)^2\,p^2}\,i\,\mathrm{e}^4\,\mathrm{Q1}\,(p\cdot u)$$
$$\left((D-4)\,p^2\left(D^3-6\,D^2+\left(-2\,D^3+15\,D^2-33\,D+20\right)\xi_{V(1)}+(D-4)^2\,(D-1)\,\xi^2_{V(1)}+11\,D-8\right)\left(\mathbf{B}^{(D)}_{\{1,0\}\,\{1,0\}}\right)^2-\right.$$
$$\left.4\,(D-3)\left(2\,D^3-11\,D^2+\left(-4\,D^3+33\,D^2-81\,D+52\right)\xi_{V(1)}+2\,(D-4)^2\,(D-3)\,\xi^2_{V(1)}+16\,D-8\right)\mathbf{J}^{(D)}_{\{1,0\}\,\{1,0\}\,\{1,0\}}\right)$$

$$(4\,\pi)^D\,\Sigma_{85}(p) = \frac{1}{(D-6)\,(D-4)^2\,p^2}\,i\,\mathrm{e}^4\,\mathrm{Q1}\,(p\cdot u)$$
$$\left(\left(D^2-10\,D+24\right)p^2\,(\xi_{V(1)}-1)\left(\left(D^2-7\,D+12\right)\xi_{V(1)}-D^2+6\,D-10\right)\left(\mathbf{B}^{(D)}_{\{1,0\}\,\{1,0\}}\right)^2+\right.$$
$$\left(-4\,D^6+66\,D^5-434\,D^4+1448\,D^3-2576\,D^2+\left(-4\,D^6+86\,D^5-769\,D^4+3681\,D^3-9990\,D^2+14\,608\,D-8992\right)\right.$$
$$\left.\left.\xi^2_{V(1)}+2\left(4\,D^6-76\,D^5+589\,D^4-2380\,D^3+5263\,D^2-5986\,D+2696\right)\xi_{V(1)}+2360\,D-960\right)\mathbf{J}^{(D)}_{\{1,0\}\,\{1,0\}\,\{1,0\}}\right)$$

$$(4\,\pi)^D\,\Sigma_{86}(p) = -\frac{4\,i\,(D-2)\,\mathrm{e}^4\,\mathrm{Q1}\,(p\cdot u)\,\mathbf{J}^{(D)}_{\{1,0\}\,\{1,0\}\,\{1,0\}}}{(D-6)\,p^2}$$

$$(4\,\pi)^D\,\Sigma_{87}(p) = 0$$

$$(4\,\pi)^D\,\Sigma_{88}(p) = \frac{1}{(D-6)\,(D-4)\,p^2}4\,i\,\mathrm{e}^4\,\mathrm{Q1}$$
$$\left(2\left(D^2-7\,D+12\right)(D-1)^2+\left(2\,D^4-26\,D^3+127\,D^2-275\,D+222\right)\xi^2_{V(1)}+\left(-4\,D^4+44\,D^3-173\,D^2+279\,D-146\right)\xi_{V(1)}\right)$$
$$(p\cdot u)\,\mathbf{J}^{(D)}_{\{1,0\}\,\{1,0\}\,\{1,0\}}$$

$$(4\,\pi)^D\,\Sigma_{89}(p) = 0$$

$$(4\,\pi)^D\,\Sigma_{90}(p) = \frac{1}{(D-6)\,(D-4)\,p^2}4\,i\,\mathrm{e}^4\,\mathrm{Q1}$$
$$\left(2\left(D^2-7\,D+12\right)(D-1)^2+\left(2\,D^4-26\,D^3+127\,D^2-275\,D+222\right)\xi^2_{V(1)}+\left(-4\,D^4+44\,D^3-173\,D^2+279\,D-146\right)\xi_{V(1)}\right)$$
$$(p\cdot u)\,\mathbf{J}^{(D)}_{\{1,0\}\,\{1,0\}\,\{1,0\}}$$

$$(4\,\pi)^D\,\Sigma_{91}(p) = 0$$

$$(4\,\pi)^D\,\Sigma_{92}(p) = \frac{1}{4}\,i\,\mathrm{e}^4\,\mathrm{Q1}\left(\left(D^2-9\,D+20\right)\xi^2_{V(1)}+\left(-2\,D^2+11\,D-9\right)\xi_{V(1)}+(D-1)^2\right)(p\cdot u)\left(\mathbf{B}^{(D)}_{\{1,0\}\,\{1,0\}}\right)^2$$

$$(4\,\pi)^D\,\Sigma_{93}(p) = 0$$

$$(4\,\pi)^D\,\Sigma_{94}(p) = 0$$

$$(4\,\pi)^D\,\Sigma_{95}(p) = 0$$

$$(4\,\pi)^D\,\Sigma_{96}(p) = \frac{1}{4}\,i\,\mathrm{e}^4\,\mathrm{Q1}\left(\left(D^2-9\,D+20\right)\xi^2_{V(1)}+\left(-2\,D^2+11\,D-9\right)\xi_{V(1)}+(D-1)^2\right)(p\cdot u)\left(\mathbf{B}^{(D)}_{\{1,0\}\,\{1,0\}}\right)^2$$

## II. FINAL REMARKS

In this supplementary material, we have presented additional information and calculation details that were not included in the main text. Specifically, we have included the two-loop Lorentz-violating diagrams related to the photon and scalar field self-energies.

### Acknowledgments

The work of A. Yu. P. has been partially supported by the CNPq project No. 301562/2019-9. The work of A. C. L. has been partially supported by the CNPq project No. 404310/2023-0.

---

[1] R. Mertig, M. Bohm and A. Denner, Comput. Phys. Commun. **64**, 345-359 (1991) doi:10.1016/0010-4655(91)90130-D; V. Shtabovenko, R. Mertig and F. Orellana, Comput. Phys. Commun. **207**, 432-444 (2016) doi:10.1016/j.cpc.2016.06.008 [arXiv:1601.01167 [hep-ph]]; V. Shtabovenko, R. Mertig and F. Orellana, Comput. Phys. Commun. **256**, 107478 (2020). doi:10.1016/j.cpc.2020.107478 [arXiv:2001.04407 [hep-ph]];

[2] T. Hahn, Comput. Phys. Commun. **140**, 418-431 (2001) doi:10.1016/S0010-4655(01)00290-9 [arXiv:hep-ph/0012260 [hep-ph]].

[3] A. Alloul, N. D. Christensen, C. Degrande, C. Duhr, and B. Fuks, Comput. Phys. Commun. **185**, 2250 (2014).

[4] V. Shtabovenko, Comput. Phys. Commun. **218**, 48-65 (2017) doi:10.1016/j.cpc.2017.04.014 [arXiv:1611.06793 [physics.comp-ph]].

[5] R. Mertig and R. Scharf, Comput. Phys. Commun. **111**, 265-273 (1998) doi:10.1016/S0010-4655(98)00042-3 [arXiv:hep-ph/9801383 [hep-ph]].

[6] O. V. Tarasov, Nucl. Phys. B **502**, 455-482 (1997) doi:10.1016/S0550-3213(97)00376-3 [arXiv:hep-ph/9703319 [hep-ph]].

[7] S. P. Martin and D. G. Robertson, Comput. Phys. Commun. **174**, 133-151 (2006) doi:10.1016/j.cpc.2005.08.005 [arXiv:hep-ph/0501132 [hep-ph]].

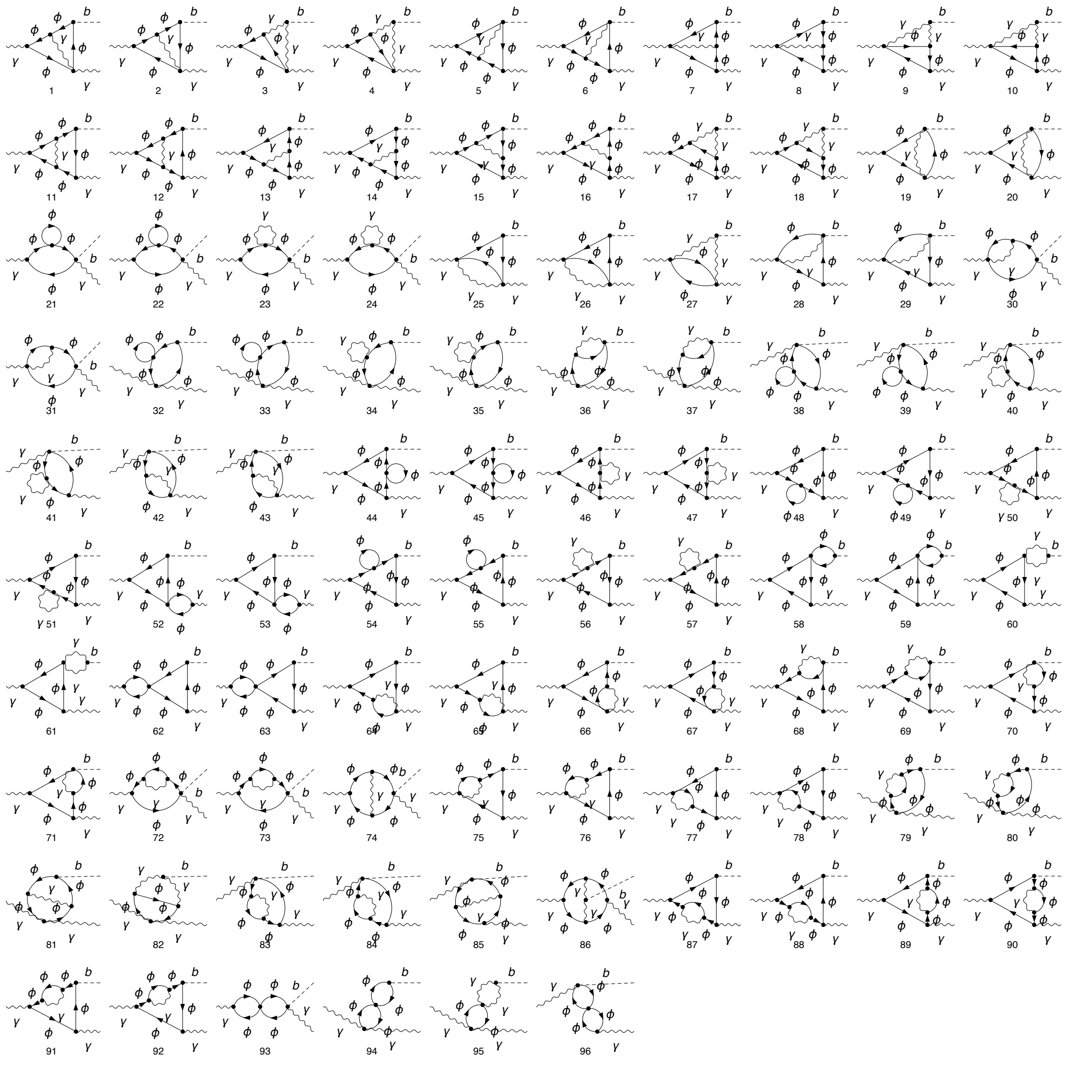

Figure 1: Feynman diagrams for the LV corrections to the two-loop photon self-energy.

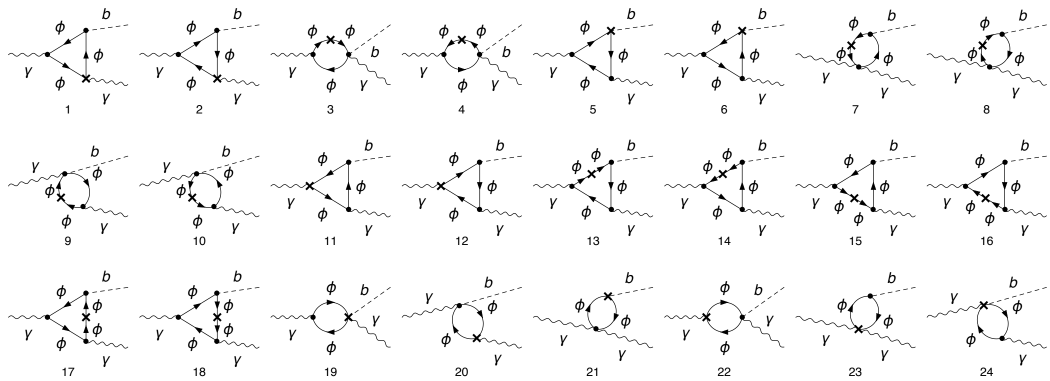

Figure 2: These one-loop Feynman diagrams illustrate the LV corrections to the photon self-energy, featuring a counterterm insertion.

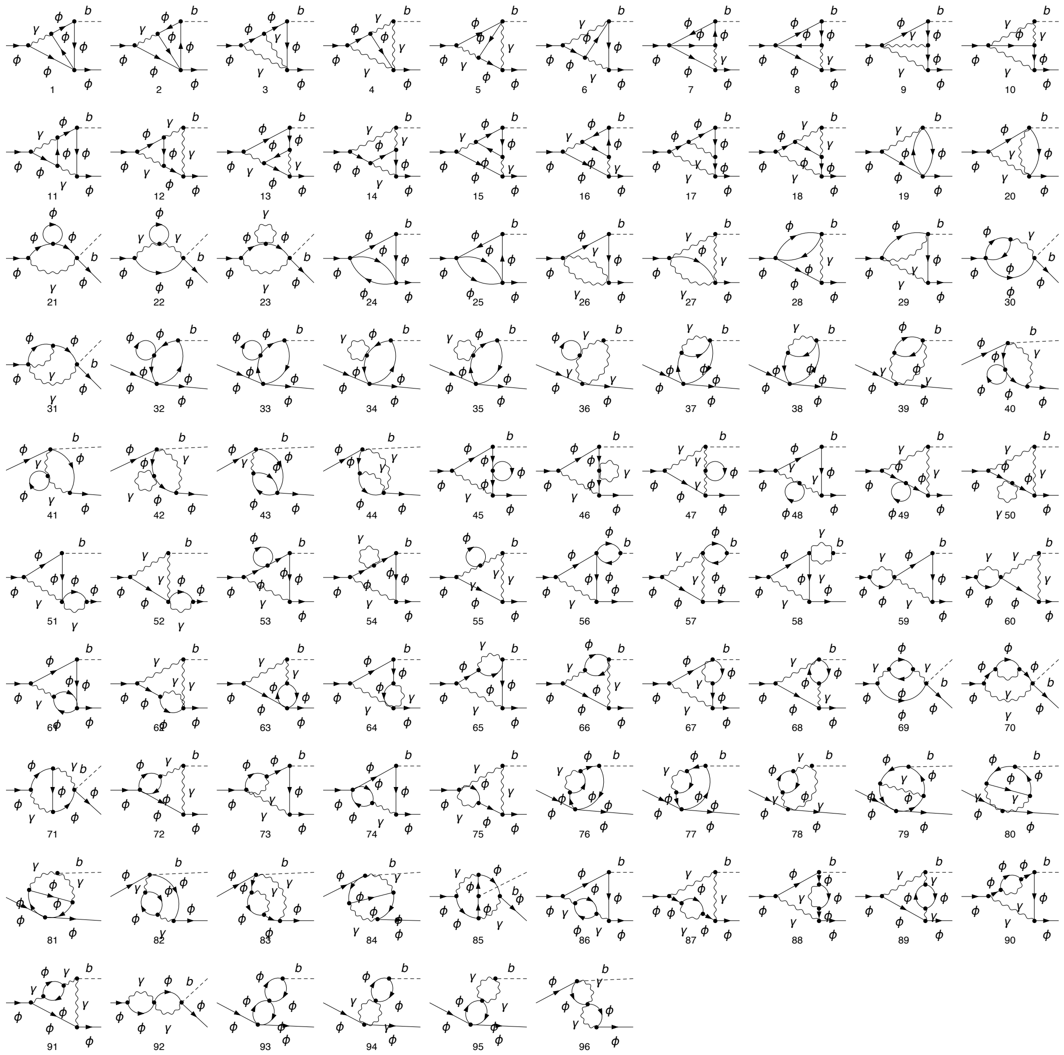

Figure 3: Feynman diagrams for the LV corrections to the two-loop scalar field self-energy.
